# Supplementary material for: A connection between $\gamma$-ray and parsec-scale radio flares in the blazar 3C 273
Source: arXiv:1703.07976 ancillary file (2017-03-23)
Supplement: Supplementary file 1 [file lisakov_radio2gamma_online.pdf]

## 1 THE FULL SET OF DATA USED IN THE ANALYSIS

Here we present details on the data used in the analysis:

- a summary of the observational data quality at 7 mm,
- total intensity maps with model components overlaid for the epochs 2009 Oct 25, 2009 Dec 05, 2010 Jan 26 in addition to 2009 Aug 28 presented in the article (Fig. 1),
- color version of spectral index slices in the transition zone for  $\alpha_{43-24}$  and  $\alpha_{15-8}$  for all epochs,
- spectral index along the ridge line for the epochs mentioned above for  $\alpha_{43-24}$ ,  $\alpha_{24-15}$ ,  $\alpha_{15-8}$ ,  $\alpha_{8-5}$ , and
- spectral index maps for the epochs mentioned above for  $\alpha_{43-24}$ ,  $\alpha_{24-15}$ ,  $\alpha_{15-8}$ ,  $\alpha_{8-5}$ .

Parameters of adjacent components in the model fit are not completely independent. To reduce the impact of uncertainties of single adjacent model components parameters we considered clusters of components, which contain 2 – 6 components each. all components in a cluster are believed to move with the same bulk velocity.

We have found two clusters in the 3C273 jet structure at 7 mm. Both clusters are model fitted with a different set of components on different epochs (Fig. 16–18): a closer one (*K1*) consists of 2 strong components with additional weaker ones, a distant one (*K2*) consists of a single strong component surrounded with weaker ones. In both cases strong components could be cross-identified across epochs for kinematics analysis but measurements are strongly scattered due to an impact of adjacent components. Meanwhile both clusters are isolated from each other and from other parts of the jet which makes cluster kinematics measurements less scattered and reveals fine effects.

Spectral index ( $S \propto \nu^{+\alpha}$ ) maps (Fig. 19–22) at any observed frequency display an opaque core with spectral index  $\alpha > 0$  and optically thin jet with  $\alpha < 0$ . Spectral index slices were fitted with two different intrinsic distributions: a *ramp* function, which has extended transition from  $\alpha > 0$  to  $\alpha < 0$ , and a simple *step* function, with sharp drop of spectral index. Both distributions were convolved with the beam and compared to the measured spectral index values. Spectral index values along the slices across the core in the direction of the jet for  $\alpha_{43-24}$  and  $\alpha_{15-8}$  are displayed at Fig. 23 and 24. In all cases except  $\alpha_{43-24}$  at the epoch 2010 Jan 26 the *ramp* function describes spectral index better than a simple *step*.

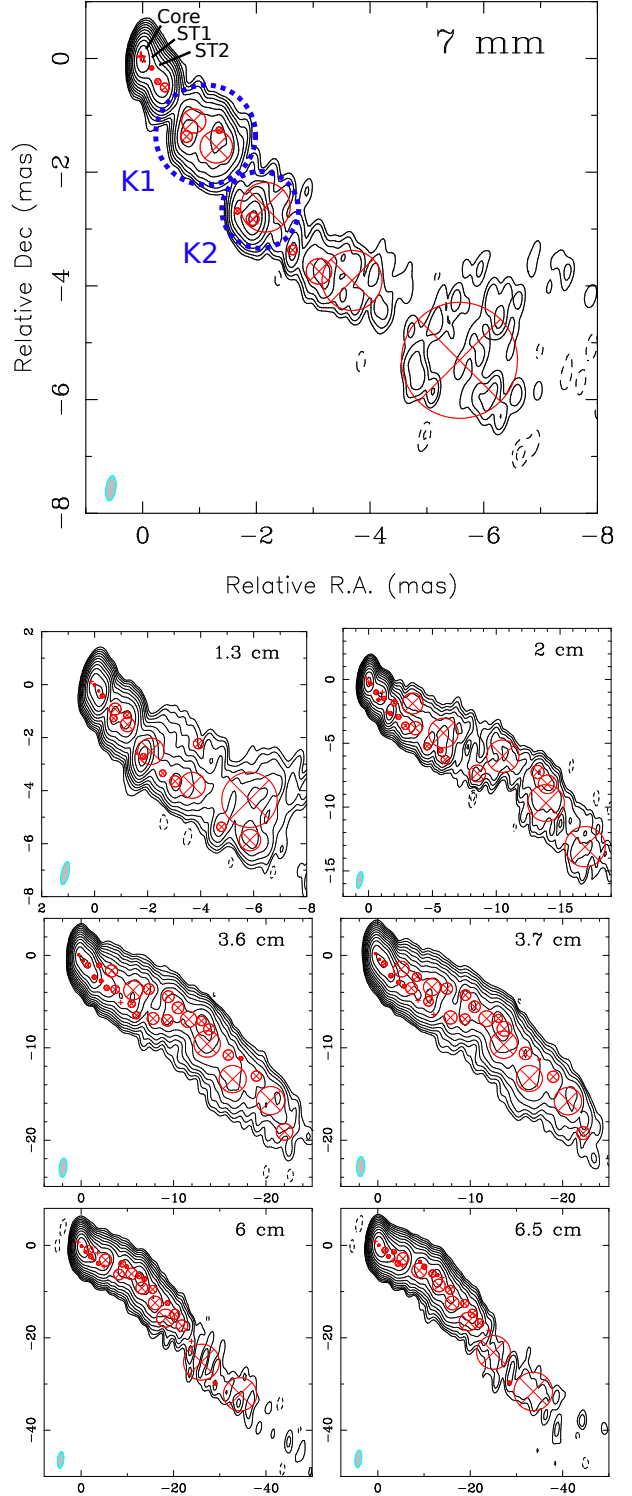

**Figure 16.** Models obtained with model fitting for epoch 2009 Dec 05. Plus signs denote  $\delta$ -function components while circles with crosses show the FWHM of Gaussian components. Axes are relative Right Ascension – relative Declination. Units are milliarcseconds. Wavelength is denoted in the upper right corner. Beam area at half maximum is shown in lower left corner. Two dashed circles on the 7 mm map mark clusters used for core shuttle analysis. Contours are plotted with a factor of 2. Image parameters (lowest contour value mJy beam<sup>-1</sup>, peak Jy beam<sup>-1</sup>): 7 mm (4, 4.7), 1.3 cm (4, 4.2), 2 cm (5, 6.6), 3.6 cm (3, 6.3), 3.7 cm (3, 6.8), 6 cm (4, 8.8), 6.5 cm (4, 9.0).

| Date        | MJD   | $N_{\text{eq}}$ | Number of<br>visibilities | Comments                                                  |
|-------------|-------|-----------------|---------------------------|-----------------------------------------------------------|
| 2008-01-17  | 54482 | 8               | 1829                      | -HN, NL 60% lost                                          |
| 2008-02-29  | 54525 | 8               | 2433                      | -HN, -FD                                                  |
| *2008-06-12 | 54629 | 6               | 1168                      | -BR, - LA, -PT                                            |
| *2008-07-06 | 54653 | 7.5             | 1956                      | -BR, -OV                                                  |
| 2008-08-15  | 54693 | 9.5             | 2408                      |                                                           |
| 2008-09-10  | 54719 | 9.5             | 3783                      |                                                           |
| 2008-11-16  | 54786 | 9               | 3159                      | MK 60% lost                                               |
| 2008-12-21  | 54821 | 9               | 3304                      | -HN                                                       |
| 2009-01-24  | 54855 | 10              | 4026                      |                                                           |
| 2009-02-22  | 54884 | 10              | 3991                      |                                                           |
| 2009-04-01  | 54922 | 10              | 3632                      |                                                           |
| 2009-05-30  | 54981 | 10              | 3493                      |                                                           |
| 2009-06-21  | 55003 | 8.7             | 2938                      | -NL                                                       |
| 2009-07-26  | 55038 | 8.7             | 2610                      | -PT                                                       |
| 2009-08-16  | 55059 | 10              | 3553                      |                                                           |
| 2009-08-28  | 55071 | 10              | 6250                      | our multifrequency observations                           |
| 2009-09-16  | 55090 | 9               | 2822                      | HN 50% lost                                               |
| 2009-10-16  | 55120 | 9               | 3324                      | -SC                                                       |
| 2009-10-25  | 55129 | 9.5             | 7628                      | our multifrequency observations                           |
| *2009-11-28 | 55163 | 7.5             | 2217                      | -MK, KP 75% lost, HN 75% lost                             |
| 2009-12-05  | 55170 | 9               | 6145                      | our multifrequency observations, SC 30% lost, NL 40% lost |
| 2010-01-10  | 55206 | 8.5             | 2866                      | -HN, KP 50% lost                                          |
| 2010-01-26  | 55222 | 8.5             | 5138                      | our multifrequency observations, -HN, NL 40% lost         |
| 2010-02-11  | 55238 | 8.5             | 2607                      | -HN                                                       |
| 2010-03-06  | 55261 | 9               | 3200                      | PT 50% lost                                               |
| 2010-05-19  | 55335 | 9.7             | 3332                      |                                                           |
| 2010-06-14  | 55361 | 8               | 1500                      | -PT, BR 60% lost                                          |
| 2010-08-01  | 55409 | 8.7             | 1839                      | -FD                                                       |
| 2010-08-21  | 55429 | 9               | 1542                      | -FD                                                       |
| 2010-09-18  | 55457 | 8.5             | 1499                      | -FD, SC 30% lost                                          |
| 2010-10-24  | 55493 | 9.7             | 3346                      |                                                           |
| 2010-12-04  | 55534 | 9.5             | 3537                      |                                                           |
| 2011-01-02  | 55563 | 9.5             | 3338                      |                                                           |
| 2011-02-04  | 55596 | 8.5             | 1976                      | -PT                                                       |
| 2011-04-21  | 55672 | 8.7             | 2132                      | -NL                                                       |
| 2011-05-22  | 55703 | 8               | 1151                      | -BR, PT 60% lost, SC 30% lost                             |
| 2011-06-12  | 55724 | 8               | 1323                      | -OV, HN 80% lost, BR 30% lost                             |
| 2011-07-21  | 55763 | 9               | 2116                      | PT 40% lost                                               |
| 2011-08-23  | 55796 | 8.7             | 1646                      | -MK                                                       |
| 2011-09-16  | 55820 | 9               | 1944                      | MK 50% lost, SC 30% lost                                  |
| 2011-10-16  | 55850 | 9               | 1969                      | HN 50% lost, SC 30% lost                                  |
| 2011-12-02  | 55897 | 9               | 2488                      |                                                           |
| 2012-01-27  | 55953 | 8               | 1603                      | -FD, HN 75% lost                                          |
| 2012-03-05  | 55991 | 9               | 1868                      | MK 30% lost                                               |
| 2012-04-02  | 56019 | 8.7             | 1888                      | -LA                                                       |
| *2012-05-26 | 56073 | 6.5             | 864                       | -MK, -OV, -LA                                             |
| 2012-07-04  | 56112 | 9.5             | 852                       |                                                           |
| 2012-08-13  | 56152 | 8.5             | 1417                      | -HN, PT 40% lost, SC 30% lost                             |
| 2012-10-28  | 56228 | 9.7             | 2504                      |                                                           |
| *2012-12-22 | 56283 | 6.5             | 1291                      | -PT, -NL, BR 90% lost                                     |

**Table 11.** Epochs and data quality of 7 mm VLBA observations, both from our multifrequency campaign and from the Boston University blazar monitoring.  $N_{\text{eq}}$  – roughly estimated number of antennas after accounting for all flagged data. Number of visibilities is calculated after IF averaging, integration time 20 sec. “-ANTENNA” in comments stands for complete loss. Epochs marked with an asterisk were excluded from analysis. Details on our multifrequency observations (5-43 GHz) are presented in the main text, Table 1.

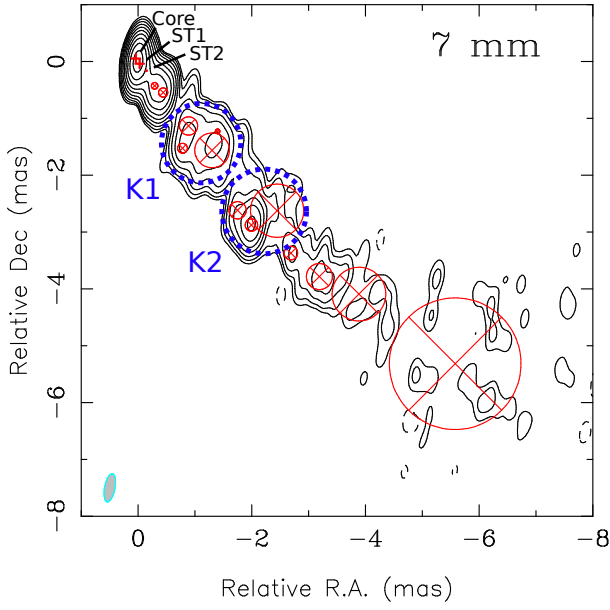

**Figure 17.** Models obtained with model fitting for epoch 2009 Dec 05. In a similar fashion as fig. 16. Image parameters (lowest contour value mJy beam<sup>-1</sup>, peak Jy beam<sup>-1</sup>): 7 mm (9, 6.5), 1.3 cm (8, 3.8), 2 cm (4, 6.5), 3.6 cm (4, 6.7), 3.7 cm (4, 7.4), 6 cm (4, 9.7), 6.5 cm (7, 9.6).

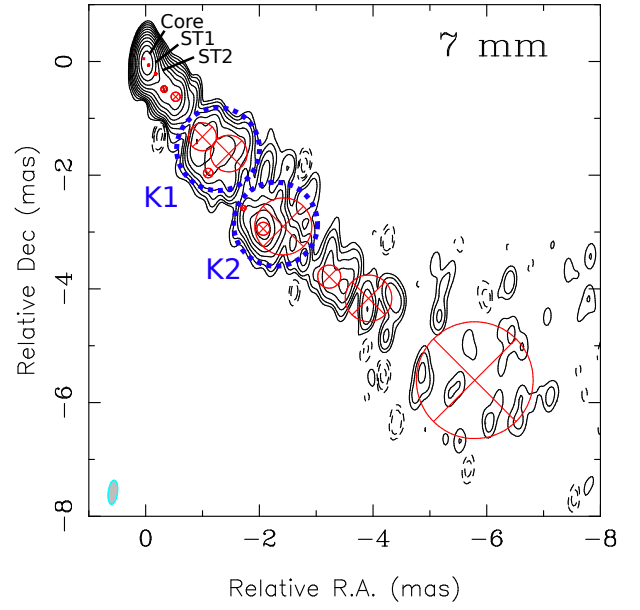

**Figure 18.** Models obtained with model fitting for epoch 2010 Jan 26. In a similar fashion as fig. 16. Image parameters (lowest contour value mJy beam<sup>-1</sup>, peak Jy beam<sup>-1</sup>): 7 mm (5, 8.6), 1.3 cm (10, 5.4), 2 cm (8, 7.4), 3.6 cm (8, 6.3), 3.7 cm (6, 7.3), 6 cm (5, 10.4), 6.5 cm (9, 9.5).

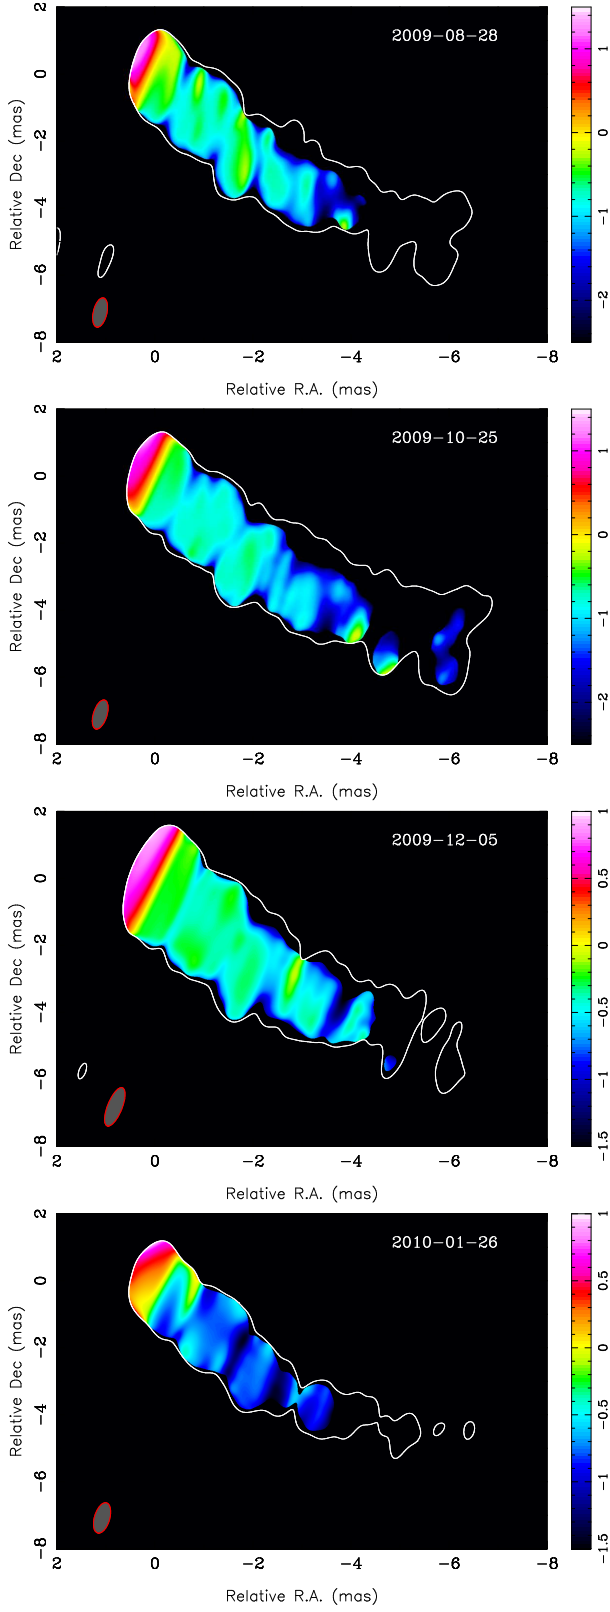

**Figure 19.** Evolution of spectral index between 43.2 and 23.8 GHz for all epochs. The contour represents source structure in full intensity at 24 GHz. Contour values per epoch are 9, 8, 13, 22 mJy. 24 GHz beam is plotted in the bottom left corner.

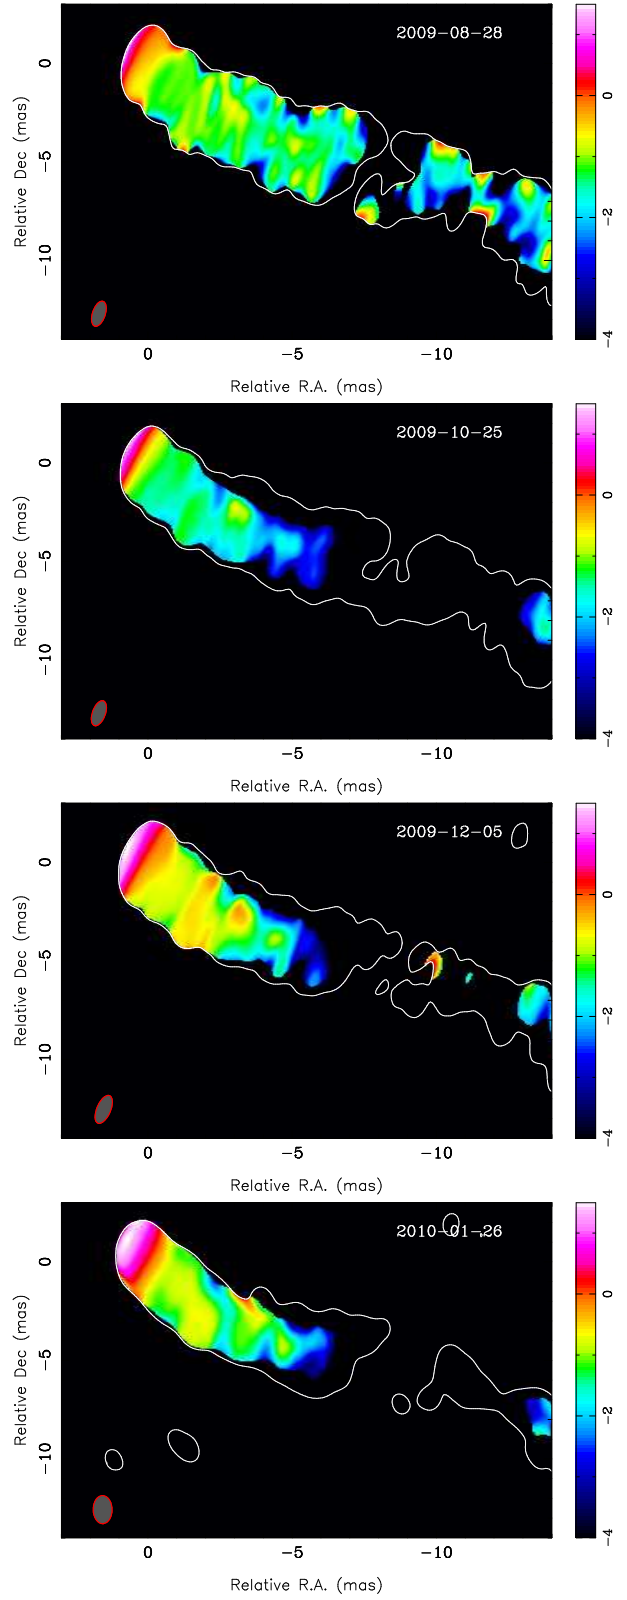

**Figure 20.** Evolution of spectral index between 23.8 and 15.4 GHz for all epochs. The contour represents source structure in full intensity at 15 GHz. Contour values per epoch are 12, 11, 22, 25 mJy. 15 GHz beam is plotted in the bottom left corner.

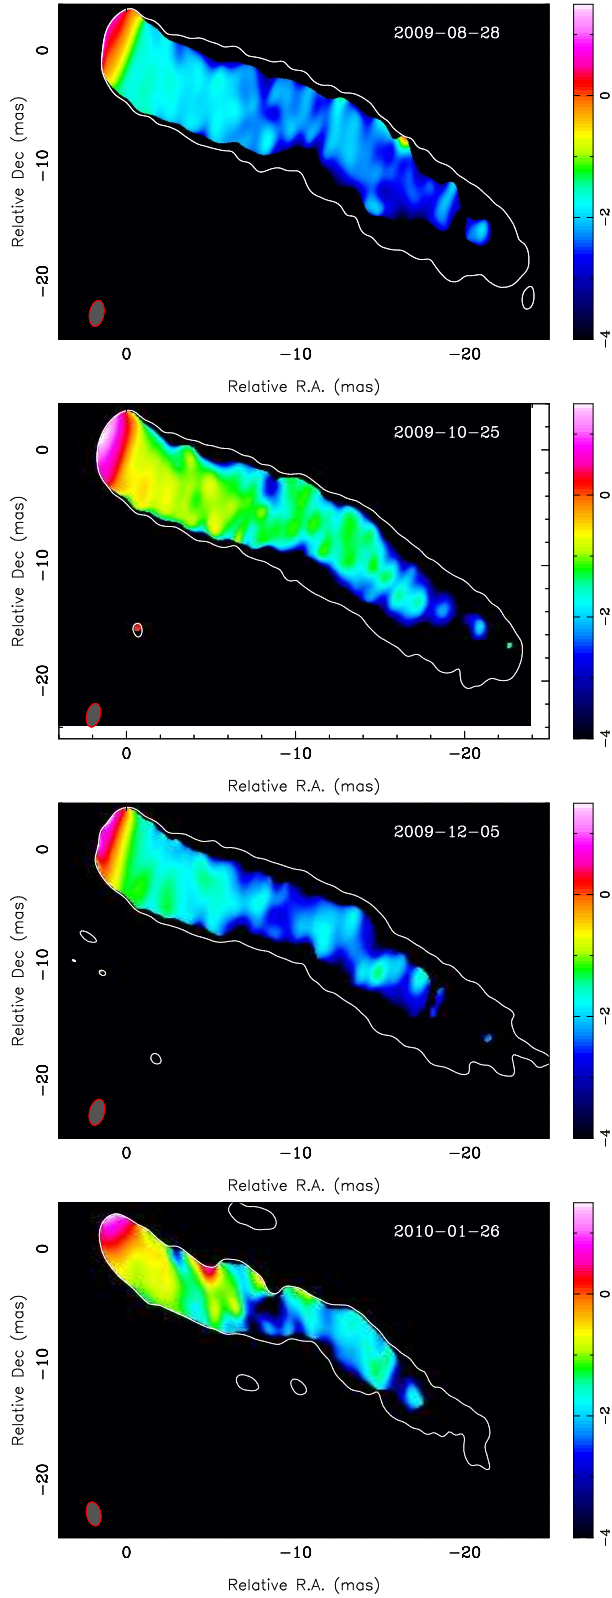

**Figure 21.** Evolution of spectral index between 15.4 and 8.4 GHz for all epochs. The contour represents source structure in full intensity at 8 GHz. Contour values per epoch are 5, 3, 8, 33 mJy. 8.4 GHz beam is plotted in the bottom left corner.

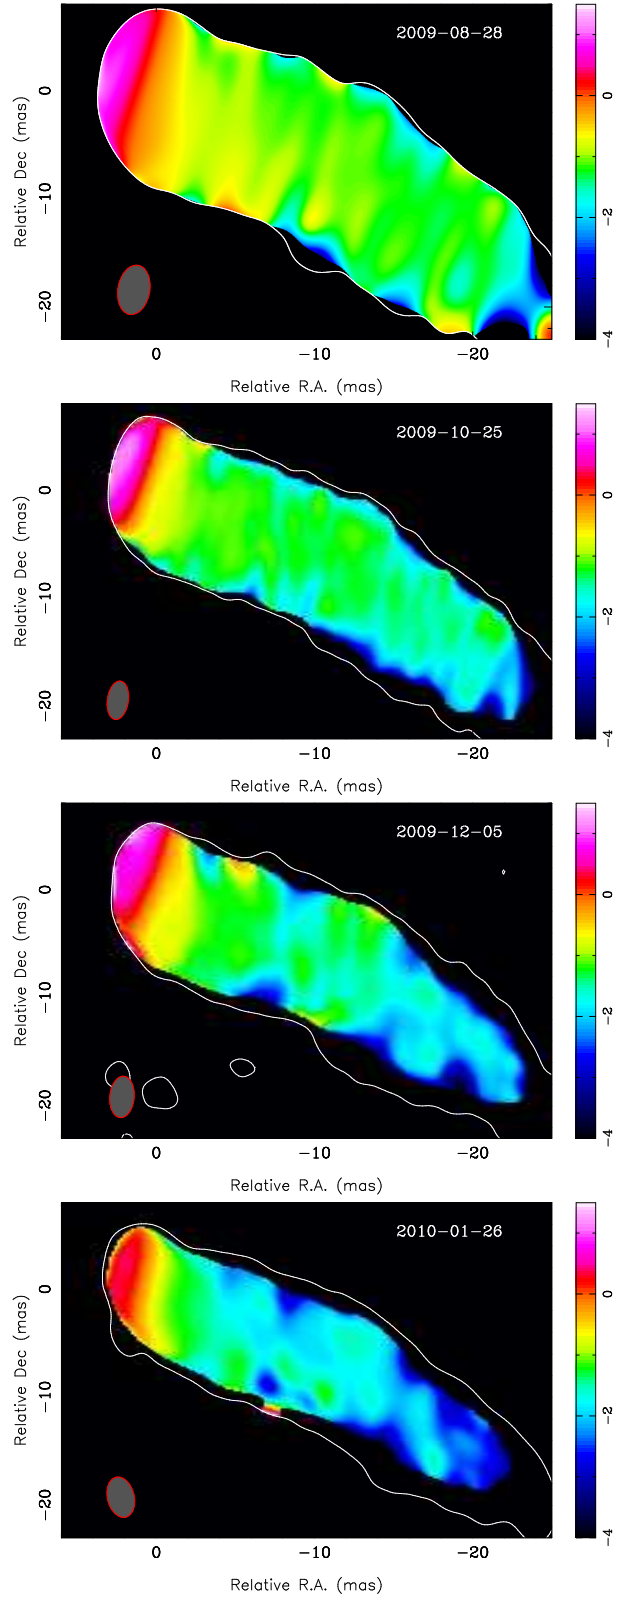

**Figure 22.** Evolution of spectral index between 8.1 and 4.6 GHz for all epochs. The contour represents source structure in full intensity at 5 GHz. Contour values per epoch are 7, 2, 5, 7 mJy. 4.6 GHz beam is plotted in the bottom left corner.

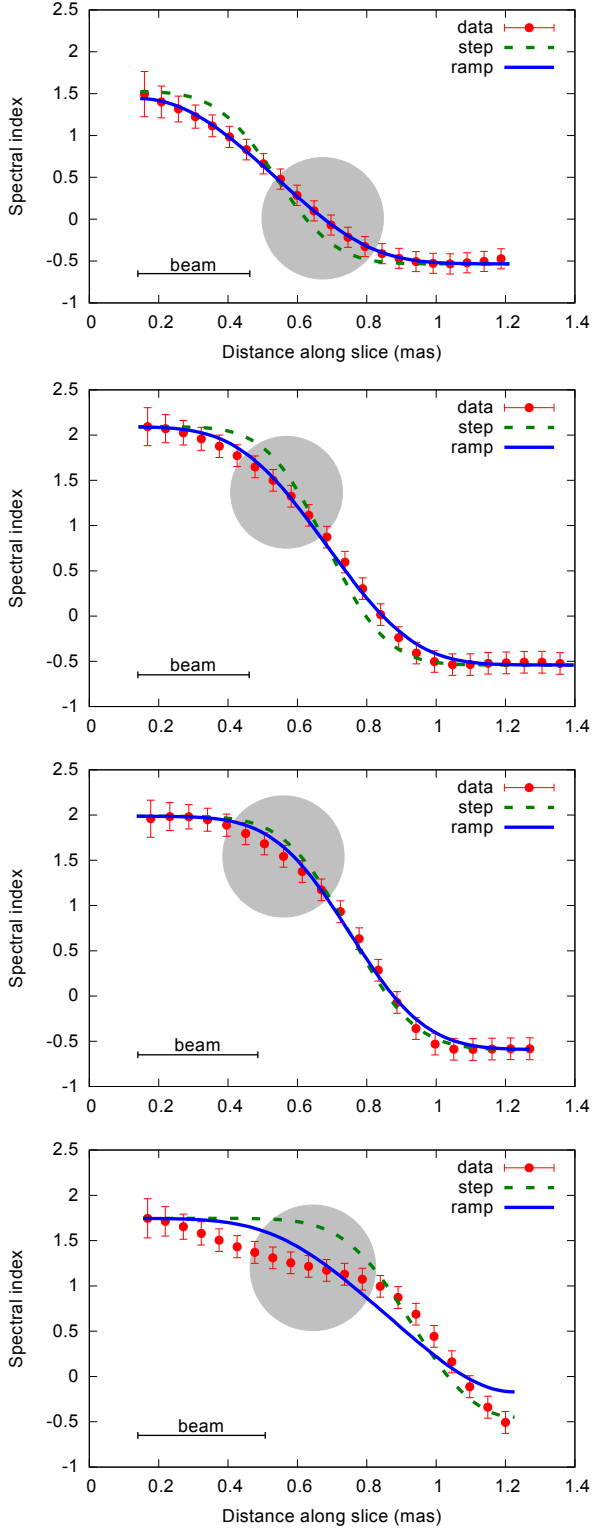

**Figure 23.** Slice of spectral index between 43 and 24 GHz taken along the jet in transition zone at epochs 2009 Aug 28, 2009 Oct 25, 2009 Dec 05, 2010 Jan 26 (top to bottom). Green line is a best fit with a *step* function, blue line is a best fit with *ramp* function. Grey shaded circle represents the FWHM and position of 24 GHz core model component convolved with the beam. Beam FWHM in the slice direction is plotted on bottom left.

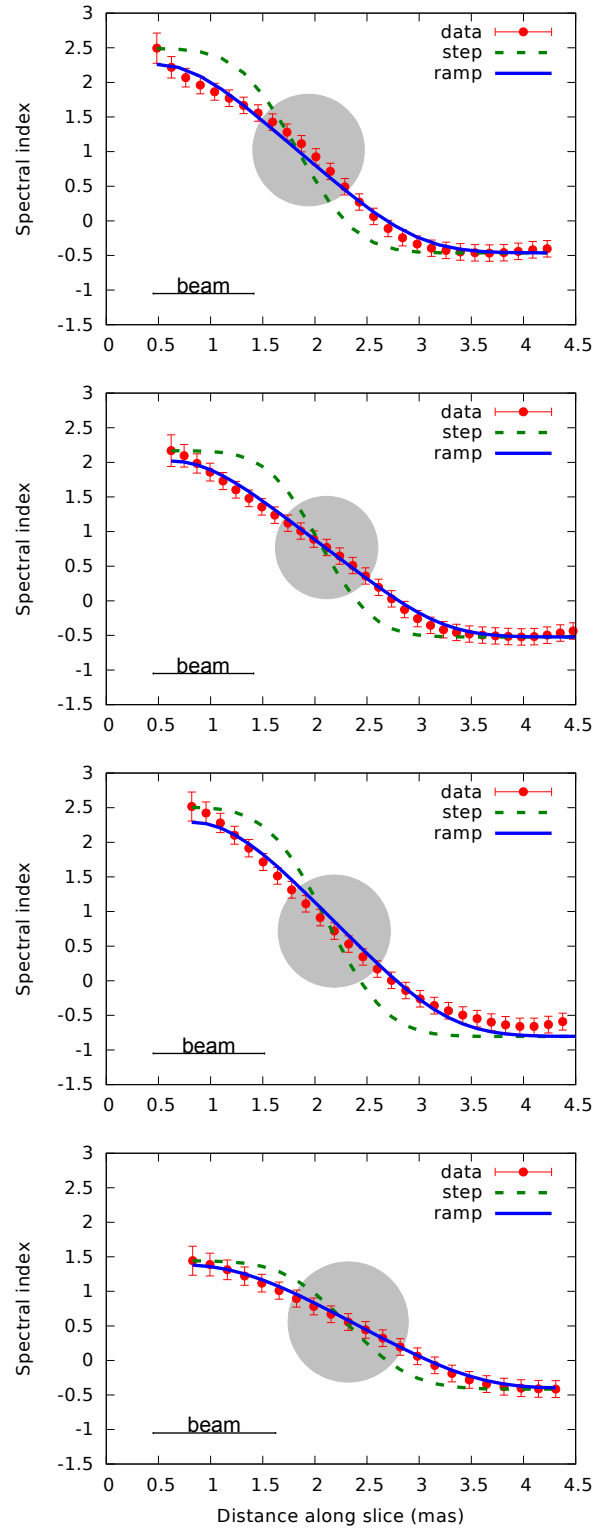

**Figure 24.** Same as in fig. 23 but for 15 – 8 GHz. Grey shaded circle represents the FWHM and position of 8 GHz core model component convolved with the beam.

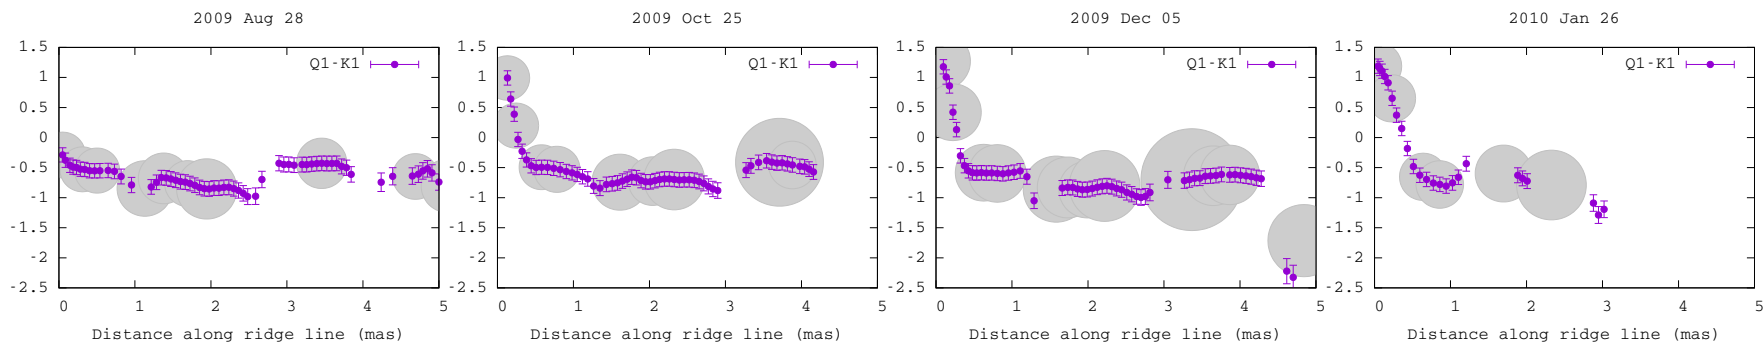

**Figure 25.** Spectral index between 43 and 24 GHz taken along the ridge line at 2009 Aug 28, 2009 Oct 25, 2009 Dec 05, 2010 Jan 26 (left to right). Grey shaded circles represent model components at 24 GHz, convolved with the 24 GHz beam.

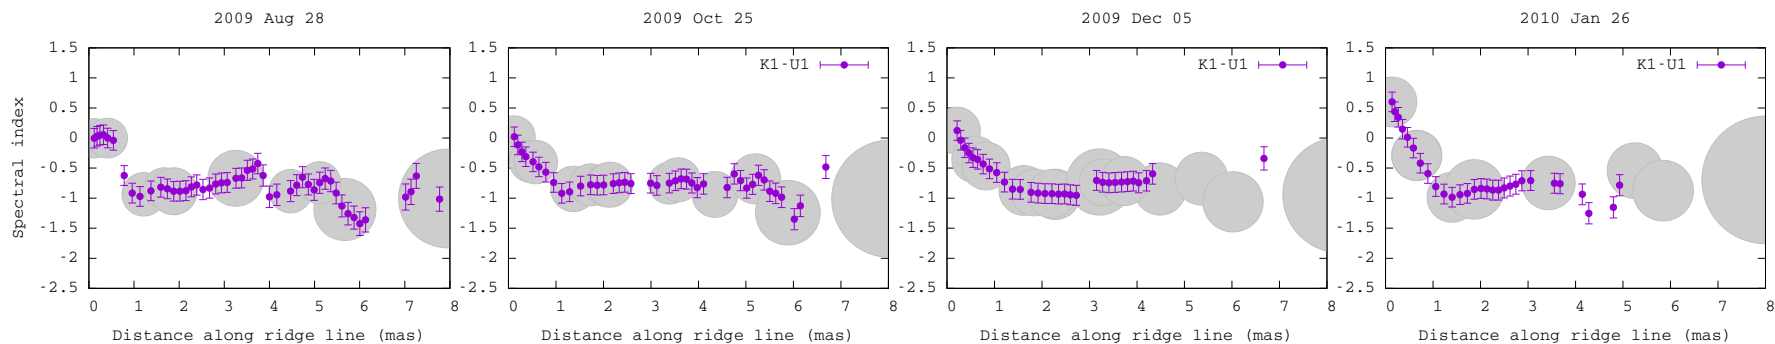

**Figure 26.** Same as fig. 25 but for 24 – 15 GHz. Grey shaded circles represent model components at 15 GHz, convolved with the 15 GHz beam.



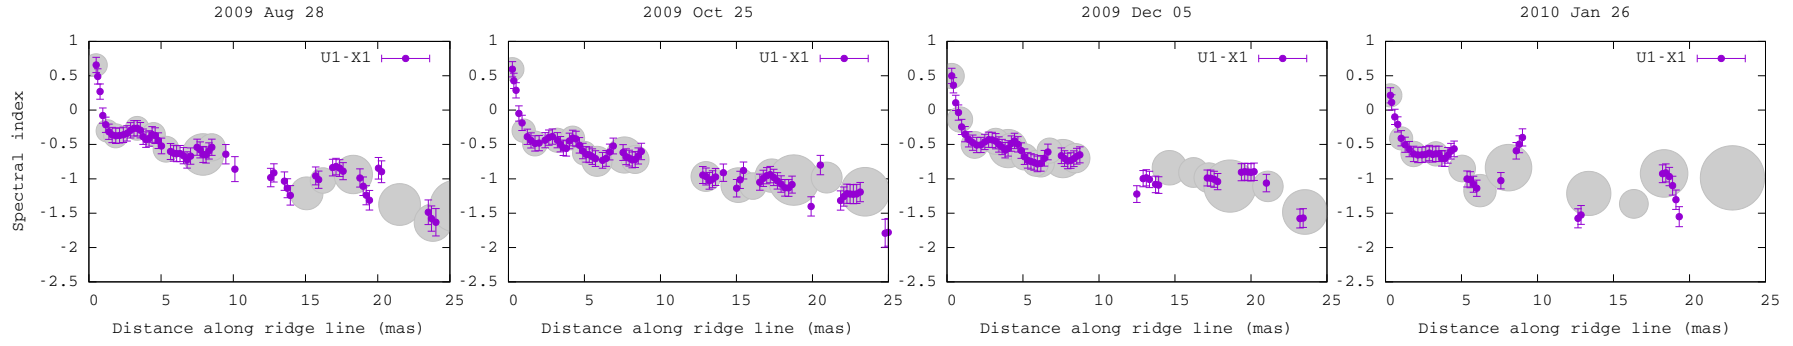

**Figure 27.** Same as fig. 25 but for 15 – 8 GHz. Grey shaded circles represent model components at 8 GHz, convolved with the 8 GHz beam.

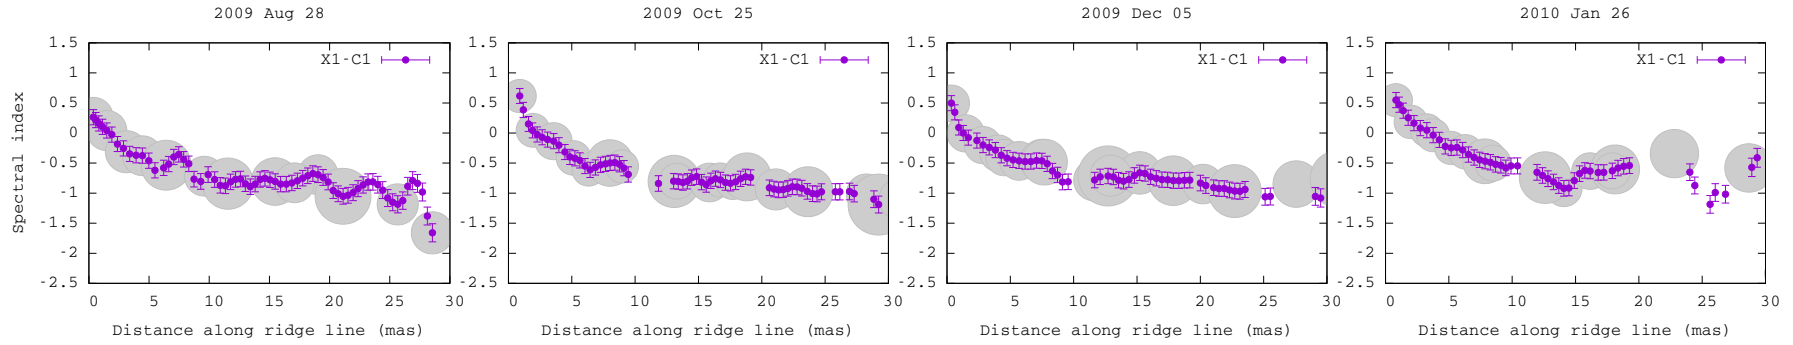

**Figure 28.** Same as fig. 25 but for 8 – 5 GHz. Grey shaded circles represent model components at 5 GHz, convolved with the 5 GHz beam.



Table 12: Modelfit parameters for all epochs. 4.6 GHz data.

| Epoch      | Component | Flux density (Jy) | Rad (mas) | Theta (deg) | Major axis (mas) | Axial ratio | Phi (deg) |
|------------|-----------|-------------------|-----------|-------------|------------------|-------------|-----------|
| 2009_08_28 | 0         | 6.05426           | 0.56779   | 50.40940    | 0                | 1.00000     | 0.00000   |
|            | 1         | 5.71666           | 0.64843   | -146.68800  | 0.39853          | 1.00000     | 0.00000   |
|            | 2         | 5.30306           | 2.23402   | -141.43400  | 1.1442           | 1.00000     | 0.00000   |
|            | 3         | 1.15141           | 3.80385   | -134.86500  | 0                | 1.00000     | 0.00000   |
|            | 4         | 5.43772           | 5.46867   | -126.17600  | 2.5023           | 1.00000     | 0.00000   |
|            | 5         | 0.22616           | 7.37588   | -111.46000  | 0                | 1.00000     | 0.00000   |
|            | 6         | 2.69537           | 10.17910  | -117.75100  | 2.6792           | 1.00000     | 0.00000   |
|            | 7         | 0.15883           | 13.09970  | -134.68400  | 0                | 1.00000     | 0.00000   |
|            | 8         | 3.45308           | 14.13850  | -119.40900  | 2.1566           | 1.00000     | 0.00000   |
|            | 9         | 0.50744           | 16.00560  | -120.19700  | 0                | 1.00000     | 0.00000   |
|            | 10        | 0.30221           | 16.63870  | -132.09400  | 0                | 1.00000     | 0.00000   |
|            | 11        | 2.19486           | 19.31540  | -126.38700  | 3.2588           | 1.00000     | 0.00000   |
|            | 12        | 0.44349           | 23.72240  | -126.94800  | 0.84911          | 1.00000     | 0.00000   |
|            | 13        | 0.33331           | 26.75180  | -126.79800  | 1.1491           | 1.00000     | 0.00000   |
|            | 14        | 0.08053           | 31.75470  | -133.15100  | 0                | 1.00000     | 0.00000   |
| 2009_10_25 | 0         | 2.23873           | 1.05782   | 31.16460    | 0                | 1.00000     | 0.00000   |
|            | 1         | 7.59613           | 0.20626   | -85.90150   | 0.51824          | 1.00000     | 0.00000   |
|            | 2         | 3.64435           | 1.58813   | -141.25400  | 7.454e-07        | 1.00000     | 0.00000   |
|            | 3         | 2.10473           | 1.88618   | -124.22000  | 1.3074           | 1.00000     | 0.00000   |
|            | 4         | 2.55671           | 3.30714   | -136.31400  | 0.77706          | 1.00000     | 0.00000   |
|            | 5         | 0.70604           | 3.76107   | -111.65800  | 0.99757          | 1.00000     | 0.00000   |
|            | 6         | 0.73381           | 4.63608   | -134.10900  | 0                | 1.00000     | 0.00000   |
|            | 7         | 1.12756           | 5.84581   | -131.82400  | 1.1973           | 1.00000     | 0.00000   |
|            | 8         | 3.40905           | 6.15460   | -117.67500  | 2.5684           | 1.00000     | 0.00000   |
|            | 9         | 0.35250           | 6.90996   | -129.96900  | 0                | 1.00000     | 0.00000   |
|            | 10        | 0.32823           | 9.77763   | -111.24000  | 0.6395           | 1.00000     | 0.00000   |
|            | 11        | 1.74112           | 10.46590  | -121.27100  | 3.1772           | 1.00000     | 0.00000   |
|            | 12        | 0.67174           | 11.06810  | -114.64000  | 1.0586           | 1.00000     | 0.00000   |
|            | 13        | 1.10526           | 13.32190  | -117.20100  | 1.5712           | 1.00000     | 0.00000   |
|            | 14        | 0.90536           | 14.39680  | -116.50900  | 0.66149          | 1.00000     | 0.00000   |
|            | 15        | 0.32973           | 15.55080  | -116.67500  | 0                | 1.00000     | 0.00000   |
|            | 16        | 2.19109           | 15.81080  | -123.32000  | 2.73             | 1.00000     | 0.00000   |
|            | 17        | 0.55939           | 18.34200  | -121.55100  | 1.9087           | 1.00000     | 0.00000   |
|            | 18        | 1.40976           | 20.37520  | -127.78100  | 2.9411           | 1.00000     | 0.00000   |
|            | 19        | 0.27116           | 22.62800  | -123.74200  | 1.6955           | 1.00000     | 0.00000   |
|            | 20        | 0.25233           | 25.20710  | -125.70300  | 1.7994           | 1.00000     | 0.00000   |
|            | 21        | 0.23628           | 25.64230  | -129.99100  | 4.0372           | 1.00000     | 0.00000   |
|            | 22        | 0.12065           | 27.70730  | -127.38400  | 1.8746           | 1.00000     | 0.00000   |
|            | 23        | 0.02396           | 30.29130  | -127.37300  | 0                | 1.00000     | 0.00000   |
|            | 24        | 0.09785           | 34.09620  | -132.75400  | 7.2881           | 1.00000     | 0.00000   |
|            | 25        | 0.02142           | 41.13660  | -136.25100  | 0.73191          | 1.00000     | 0.00000   |
|            | 26        | 0.16797           | 46.16870  | -133.22900  | 8.3226           | 1.00000     | 0.00000   |
| 2009_12_05 | 0         | 2.42644           | 0.57887   | 50.50160    | 0                | 1.00000     | 0.00000   |
|            | 1         | 7.38658           | 0.63673   | -147.59600  | 0.56249          | 1.00000     | 0.00000   |
|            | 2         | 5.15679           | 2.18454   | -145.67900  | 0.60201          | 1.00000     | 0.00000   |
|            | 3         | 0.22152           | 2.81176   | -72.70300   | 2.2962           | 1.00000     | 0.00000   |
|            | 4         | 0.76723           | 3.30185   | -127.85100  | 0.30045          | 1.00000     | 0.00000   |
|            | 5         | 1.42283           | 3.91339   | -143.74300  | 0                | 1.00000     | 0.00000   |
|            | 6         | 1.85035           | 4.68689   | -131.10700  | 1.0063           | 1.00000     | 0.00000   |
|            | 7         | 1.45149           | 6.66921   | -135.46200  | 1.8182           | 1.00000     | 0.00000   |
|            | 8         | 2.86901           | 6.68972   | -120.67400  | 2.1779           | 1.00000     | 0.00000   |
|            | 9         | 0.90889           | 11.56430  | -118.56100  | 1.4847           | 1.00000     | 0.00000   |
|            | 10        | 0.71359           | 10.18180  | -115.77700  | 1.6228           | 1.00000     | 0.00000   |
|            | 11        | 1.21862           | 11.12430  | -125.64800  | 3.7609           | 1.00000     | 0.00000   |
|            | 12        | 0.83937           | 13.71650  | -118.47100  | 1.7113           | 1.00000     | 0.00000   |
|            | 13        | 0.88513           | 14.78610  | -117.68300  | 1.2061           | 1.00000     | 0.00000   |

Continued on next page

Table 12 – continued from previous page

| Epoch      | Component | Flux density<br>(Jy) | Rad<br>(mas) | Theta<br>(deg) | Major axis<br>(mas) | Axial ratio | Phi<br>(deg) |
|------------|-----------|----------------------|--------------|----------------|---------------------|-------------|--------------|
|            | 14        | 2.50406              | 16.08520     | -123.60400     | 2.6459              | 1.00000     | 0.00000      |
|            | 15        | 0.28721              | 18.70870     | -122.84900     | 1.2204              | 1.00000     | 0.00000      |
|            | 16        | 1.57732              | 20.63340     | -128.13400     | 3.0181              | 1.00000     | 0.00000      |
|            | 17        | 0.17903              | 22.96450     | -124.37700     | 1.1555              | 1.00000     | 0.00000      |
|            | 18        | 0.08978              | 24.96490     | -134.86000     | 1.8103              | 1.00000     | 0.00000      |
|            | 19        | 0.38997              | 25.63240     | -126.63400     | 2.2762              | 1.00000     | 0.00000      |
|            | 20        | 0.20699              | 28.73660     | -129.57600     | 3.4879              | 1.00000     | 0.00000      |
|            | 21        | 0.04863              | 37.12370     | -136.67500     | 4.2218              | 1.00000     | 0.00000      |
|            | 22        | 0.16625              | 45.45920     | -133.57600     | 6.4631              | 1.00000     | 0.00000      |
| 2010_01_26 | 0         | 3.81800              | 1.01492      | 42.59840       | 0                   | 1.00000     | 0.00000      |
|            | 1         | 7.24358              | 0.31744      | -141.72400     | 0.38659             | 1.00000     | 0.00000      |
|            | 2         | 1.29598              | 1.75439      | -122.23700     | 0                   | 1.00000     | 0.00000      |
|            | 3         | 2.86093              | 2.00423      | -148.65700     | 0                   | 1.00000     | 0.00000      |
|            | 4         | 0.75302              | 3.15023      | -115.81600     | 1.1863              | 1.00000     | 0.00000      |
|            | 5         | 1.69260              | 3.51804      | -138.68700     | 0                   | 1.00000     | 0.00000      |
|            | 6         | 1.20138              | 4.73292      | -132.91300     | 0.74044             | 1.00000     | 0.00000      |
|            | 7         | 2.99450              | 6.01976      | -116.68000     | 2.3717              | 1.00000     | 0.00000      |
|            | 8         | 1.01537              | 6.45632      | -131.10400     | 1.1118              | 1.00000     | 0.00000      |
|            | 9         | 1.52090              | 10.14490     | -122.15100     | 3.1351              | 1.00000     | 0.00000      |
|            | 10        | 0.62438              | 10.31720     | -114.96600     | 0.81666             | 1.00000     | 0.00000      |
|            | 11        | 0.80128              | 11.74530     | -115.87400     | 1.2067              | 1.00000     | 0.00000      |
|            | 12        | 1.20535              | 13.93620     | -117.01900     | 1.2293              | 1.00000     | 0.00000      |
|            | 13        | 1.91849              | 15.30410     | -123.91400     | 2.8399              | 1.00000     | 0.00000      |
|            | 14        | 0.68197              | 15.59860     | -119.04300     | 1.105               | 1.00000     | 0.00000      |
|            | 15        | 0.31335              | 17.38510     | -120.38300     | 0.71318             | 1.00000     | 0.00000      |
|            | 16        | 1.45724              | 19.82180     | -127.99000     | 2.7753              | 1.00000     | 0.00000      |
|            | 17        | 0.42457              | 22.00440     | -123.76800     | 1.6783              | 1.00000     | 0.00000      |
|            | 18        | 0.05322              | 24.56580     | -133.32300     | 0                   | 1.00000     | 0.00000      |
|            | 19        | 0.46940              | 25.93150     | -127.30700     | 2.7903              | 1.00000     | 0.00000      |
|            | 20        | 0.06417              | 28.31840     | -127.41400     | 0                   | 1.00000     | 0.00000      |
|            | 21        | 0.05853              | 33.45740     | -134.84600     | 1.7275              | 1.00000     | 0.00000      |
|            | 22        | 0.07085              | 41.46770     | -135.94200     | 3.1223              | 1.00000     | 0.00000      |
|            | 23        | 0.14871              | 47.64650     | -132.64200     | 6.4147              | 1.00000     | 0.00000      |

Table 13: Modelfit parameters for all epochs. 5.0 GHz data.

| Epoch      | Component | Flux density<br>(Jy) | Rad<br>(mas) | Theta<br>(deg) | Major axis<br>(mas) | Axial ratio | Phi<br>(deg) |
|------------|-----------|----------------------|--------------|----------------|---------------------|-------------|--------------|
| 2009_08_28 | 0         | 4.51980              | 0.51337      | 52.99310       | 0.42039             | 1.00000     | 0.00000      |
|            | 1         | 6.92735              | 0.58192      | -152.73800     | 0.62279             | 1.00000     | 0.00000      |
|            | 2         | 3.51364              | 1.97208      | -147.52000     | 0.43415             | 1.00000     | 0.00000      |
|            | 3         | 3.46163              | 3.21147      | -135.59900     | 1.3801              | 1.00000     | 0.00000      |
|            | 4         | 5.80708              | 5.77580      | -127.71900     | 3.0322              | 0.89970     | 83.99020     |
|            | 5         | 2.42579              | 10.54140     | -118.06200     | 2.5804              | 1.00000     | 0.00000      |
|            | 6         | 3.27232              | 14.46720     | -119.44100     | 2.1519              | 1.00000     | 0.00000      |
|            | 7         | 1.37642              | 17.96100     | -124.89700     | 2.5095              | 1.00000     | 0.00000      |
|            | 8         | 1.26882              | 21.08260     | -127.51200     | 3.3552              | 1.00000     | 0.00000      |
|            | 9         | 0.44513              | 25.53510     | -126.98500     | 2.1328              | 1.00000     | 0.00000      |
|            | 10        | 0.26093              | 16.10100     | -131.90200     | 1.0168              | 1.00000     | 0.00000      |
|            | 11        | 0.13367              | 12.61250     | -134.96600     | 0.038034            | 1.00000     | 0.00000      |
|            | 12        | 0.09844              | 29.48670     | -133.16200     | 2.0329e-07          | 1.00000     | 0.00000      |
| 2009_10_25 | 0         | 2.37447              | 0.96126      | 43.17490       | 0                   | 1.00000     | 0.00000      |
|            | 1         | 7.56234              | 0.18210      | -146.35700     | 0.53055             | 1.00000     | 0.00000      |
|            | 2         | 4.53966              | 1.66567      | -147.26400     | 0.49513             | 1.00000     | 0.00000      |
|            | 3         | 1.11464              | 1.88743      | -120.92800     | 1.8884              | 1.00000     | 0.00000      |

Continued on next page

Table 13 – continued from previous page

| Epoch      | Component | Flux density<br>(Jy) | Rad<br>(mas) | Theta<br>(deg) | Major<br>axis<br>(mas) | Axial<br>ratio | Phi<br>(deg) |
|------------|-----------|----------------------|--------------|----------------|------------------------|----------------|--------------|
|            | 4         | 2.62736              | 3.14725      | -138.98100     | 0.93922                | 1.00000        | 0.00000      |
|            | 5         | 0.73039              | 4.09521      | -138.33400     | 0                      | 1.00000        | 0.00000      |
|            | 6         | 0.43350              | 3.94419      | -114.33000     | 0                      | 1.00000        | 0.00000      |
|            | 7         | 0.97812              | 5.41271      | -135.77200     | 0.87076                | 1.00000        | 0.00000      |
|            | 8         | 3.67836              | 6.17176      | -120.97400     | 2.6412                 | 1.00000        | 0.00000      |
|            | 9         | 0.51921              | 6.78106      | -132.75600     | 0                      | 1.00000        | 0.00000      |
|            | 10        | 0.61211              | 9.74888      | -113.94700     | 1.4148                 | 1.00000        | 0.00000      |
|            | 11        | 0.72088              | 10.34570     | -127.56900     | 2.2983                 | 1.00000        | 0.00000      |
|            | 12        | 0.51386              | 10.89010     | -114.88800     | 0.75136                | 1.00000        | 0.00000      |
|            | 13        | 1.34610              | 12.54740     | -119.45200     | 2.4907                 | 1.00000        | 0.00000      |
|            | 14        | 1.31071              | 14.22620     | -117.82200     | 1.1159                 | 1.00000        | 0.00000      |
|            | 15        | 0.52494              | 15.51680     | -117.91800     | 1.0073                 | 1.00000        | 0.00000      |
|            | 16        | 1.60144              | 16.04410     | -125.10100     | 2.5512                 | 1.00000        | 0.00000      |
|            | 17        | 0.47108              | 18.19090     | -121.62600     | 1.7436                 | 1.00000        | 0.00000      |
|            | 18        | 1.36665              | 20.28100     | -127.86800     | 2.9214                 | 1.00000        | 0.00000      |
|            | 19        | 0.16576              | 22.48460     | -123.76600     | 1.0171                 | 1.00000        | 0.00000      |
|            | 20        | 0.20587              | 24.13720     | -130.73200     | 3.8961                 | 1.00000        | 0.00000      |
|            | 21        | 0.30062              | 25.17900     | -126.31400     | 2.1555                 | 1.00000        | 0.00000      |
|            | 22        | 0.16210              | 27.91280     | -128.50600     | 2.5267                 | 1.00000        | 0.00000      |
|            | 23        | 0.01899              | 31.62420     | -130.99000     | 0                      | 1.00000        | 0.00000      |
|            | 24        | 0.10159              | 36.28160     | -134.12700     | 7.775                  | 1.00000        | 0.00000      |
|            | 25        | 0.02333              | 41.57390     | -135.79800     | 0.77356                | 1.00000        | 0.00000      |
|            | 26        | 0.12918              | 47.14380     | -133.12300     | 7.1886                 | 1.00000        | 0.00000      |
| 2009_12_05 | 0         | 2.43941              | 0.61372      | 46.28780       | 0                      | 1.00000        | 0.00000      |
|            | 1         | 7.39789              | 0.59813      | -146.60500     | 0.54148                | 1.00000        | 0.00000      |
|            | 2         | 4.18825              | 1.94612      | -145.24500     | 0.36863                | 1.00000        | 0.00000      |
|            | 3         | 3.07246              | 3.02295      | -140.47500     | 1.1754                 | 1.00000        | 0.00000      |
|            | 4         | 1.59974              | 4.27740      | -137.70600     | 0.67299                | 1.00000        | 0.00000      |
|            | 5         | 0.39107              | 4.43386      | -117.18200     | 0                      | 1.00000        | 0.00000      |
|            | 6         | 1.67381              | 5.89981      | -134.53100     | 1.5305                 | 1.00000        | 0.00000      |
|            | 7         | 3.03977              | 6.76210      | -120.74500     | 2.3909                 | 1.00000        | 0.00000      |
|            | 8         | 0.40802              | 7.56960      | -134.78800     | 0                      | 1.00000        | 0.00000      |
|            | 9         | 0.41380              | 10.13290     | -113.30900     | 1.0809                 | 1.00000        | 0.00000      |
|            | 10        | 0.85972              | 10.58310     | -126.99300     | 2.8118                 | 1.00000        | 0.00000      |
|            | 11        | 0.28773              | 11.20320     | -115.68500     | 0                      | 1.00000        | 0.00000      |
|            | 12        | 1.37720              | 12.23720     | -119.91800     | 2.3402                 | 1.00000        | 0.00000      |
|            | 13        | 1.59691              | 14.59540     | -118.63000     | 1.4006                 | 1.00000        | 0.00000      |
|            | 14        | 0.58252              | 16.04980     | -119.07300     | 1.2242                 | 1.00000        | 0.00000      |
|            | 15        | 1.48760              | 16.38850     | -125.87800     | 2.5625                 | 1.00000        | 0.00000      |
|            | 16        | 0.46143              | 18.39920     | -122.11000     | 1.781                  | 1.00000        | 0.00000      |
|            | 17        | 1.31380              | 20.51320     | -127.89100     | 2.7104                 | 1.00000        | 0.00000      |
|            | 18        | 0.20441              | 22.82300     | -124.40700     | 1.3904                 | 1.00000        | 0.00000      |
|            | 19        | 0.30663              | 23.63750     | -131.50000     | 4.4706                 | 1.00000        | 0.00000      |
|            | 20        | 0.31301              | 25.62710     | -126.55100     | 2.1347                 | 1.00000        | 0.00000      |
|            | 21        | 0.16853              | 28.46240     | -128.90600     | 2.6167                 | 1.00000        | 0.00000      |
|            | 22        | 0.15593              | 37.29960     | -134.44500     | 9.0954                 | 1.00000        | 0.00000      |
|            | 23        | 0.05916              | 43.41480     | -135.93300     | 3.005                  | 1.00000        | 0.00000      |
|            | 24        | 0.11580              | 49.76600     | -132.48300     | 6.6324                 | 1.00000        | 0.00000      |
|            | 25        | 0.51123              | 2.14362      | -95.82700      | 2.6518                 | 1.00000        | 0.00000      |
|            | 26        | 0.02617              | 57.28360     | -138.87400     | 1.3176                 | 1.00000        | 0.00000      |
|            | 27        | 0.07630              | 67.77340     | -133.90100     | 12.481                 | 1.00000        | 0.00000      |
| 2010_01_26 | 0         | 2.32059              | 0.77661      | 42.08220       | 6.4201e-08             | 1.00000        | 0.00000      |
|            | 1         | 6.77780              | 0.46251      | -144.43700     | 0.48871                | 1.00000        | 0.00000      |
|            | 2         | 4.43350              | 1.86874      | -142.77300     | 0.31851                | 1.00000        | 0.00000      |
|            | 3         | 0.26405              | 2.68142      | -94.42370      | 2.5597                 | 1.00000        | 0.00000      |
|            | 4         | 2.35597              | 3.19863      | -138.04900     | 1.1208                 | 1.00000        | 0.00000      |
|            | 5         | 1.59960              | 4.30123      | -134.53100     | 1.1                    | 1.00000        | 0.00000      |

Continued on next page

Table 13 – continued from previous page

| Epoch | Component | Flux density<br>(Jy) | Rad<br>(mas) | Theta<br>(deg) | Major<br>axis<br>(mas) | Axial<br>ratio | Phi<br>(deg) |
|-------|-----------|----------------------|--------------|----------------|------------------------|----------------|--------------|
|       | 6         | 0.20730              | 4.51139      | -113.49000     | 0.218                  | 1.00000        | 0.00000      |
|       | 7         | 1.15197              | 5.87674      | -134.90300     | 1.2708                 | 1.00000        | 0.00000      |
|       | 8         | 2.59733              | 6.60033      | -118.81200     | 2.254                  | 1.00000        | 0.00000      |
|       | 9         | 0.47374              | 7.46124      | -131.77200     | 0.011223               | 1.00000        | 0.00000      |
|       | 10        | 1.54607              | 10.47780     | -122.70200     | 3.1353                 | 1.00000        | 0.00000      |
|       | 11        | 0.21896              | 10.57760     | -114.34800     | 0.82329                | 1.00000        | 0.00000      |
|       | 12        | 0.23942              | 11.14200     | -116.02100     | 0.34235                | 1.00000        | 0.00000      |
|       | 13        | 0.72761              | 12.32540     | -117.49700     | 1.5292                 | 1.00000        | 0.00000      |
|       | 14        | 1.28542              | 14.62520     | -117.82200     | 1.4104                 | 1.00000        | 0.00000      |
|       | 15        | 1.52412              | 15.61370     | -124.63800     | 2.7018                 | 1.00000        | 0.00000      |
|       | 16        | 0.55456              | 16.38200     | -120.42300     | 1.1698                 | 1.00000        | 0.00000      |
|       | 17        | 0.22631              | 18.22700     | -121.06000     | 1.309                  | 1.00000        | 0.00000      |
|       | 18        | 1.62542              | 20.25600     | -127.33600     | 3.19                   | 1.00000        | 0.00000      |
|       | 19        | 0.15017              | 23.24920     | -126.15300     | 0.89787                | 1.00000        | 0.00000      |
|       | 20        | 0.07419              | 24.84070     | -133.22200     | 1.3222                 | 1.00000        | 0.00000      |
|       | 21        | 0.29374              | 25.16030     | -125.30900     | 1.5475                 | 1.00000        | 0.00000      |
|       | 22        | 0.24554              | 28.11610     | -129.31900     | 3.0971                 | 1.00000        | 0.00000      |
|       | 23        | 0.07700              | 34.61070     | -136.27400     | 6.4264                 | 1.00000        | 0.00000      |
|       | 24        | 0.14612              | 44.00520     | -133.96500     | 6.4307                 | 1.00000        | 0.00000      |
|       | 25        | 0.05202              | 50.39670     | -133.68400     | 3.5407                 | 1.00000        | 0.00000      |
|       | 26        | 0.05793              | 76.94850     | -113.24000     | 15.818                 | 1.00000        | 0.00000      |

Table 14: Modelfit parameters for all epochs. 8.1 GHz data.

| Epoch      | Component | Flux density<br>(Jy) | Rad<br>(mas) | Theta<br>(deg) | Major<br>axis<br>(mas) | Axial<br>ratio | Phi<br>(deg) |
|------------|-----------|----------------------|--------------|----------------|------------------------|----------------|--------------|
| 2009_08_28 | 0         | 3.59511              | 0.56654      | 34.77410       | 0.20808                | 1.00000        | 0.00000      |
|            | 1         | 2.64192              | 0.23219      | -147.74700     | 0                      | 1.00000        | 0.00000      |
|            | 2         | 7.04849              | 0.83489      | -133.15500     | 0.59723                | 1.00000        | 0.00000      |
|            | 3         | 4.34056              | 2.27501      | -144.56700     | 0.57068                | 1.00000        | 0.00000      |
|            | 4         | 0.14282              | 2.41374      | -94.32120      | 0.89733                | 1.00000        | 0.00000      |
|            | 5         | 0.21078              | 3.25529      | -113.54900     | 2.624e-08              | 1.00000        | 0.00000      |
|            | 6         | 1.10546              | 3.39044      | -140.41000     | 0.50415                | 1.00000        | 0.00000      |
|            | 7         | 1.95535              | 4.22243      | -136.09800     | 0.89404                | 1.00000        | 0.00000      |
|            | 8         | 0.29713              | 4.64032      | -117.09900     | 0.35398                | 1.00000        | 0.00000      |
|            | 9         | 0.65354              | 5.93103      | -136.13900     | 0.7585                 | 1.00000        | 0.00000      |
|            | 10        | 2.21942              | 6.62477      | -120.55300     | 2.4248                 | 1.00000        | 0.00000      |
|            | 11        | 0.81125              | 7.07855      | -131.49500     | 1.063                  | 1.00000        | 0.00000      |
|            | 12        | 0.50199              | 11.39300     | -116.26500     | 1.2585                 | 1.00000        | 0.00000      |
|            | 13        | 0.59022              | 13.23330     | -119.47700     | 1.6605                 | 1.00000        | 0.00000      |
|            | 14        | 0.57370              | 14.38890     | -117.26900     | 0.84381                | 1.00000        | 0.00000      |
|            | 15        | 0.32932              | 15.22330     | -117.24000     | 0.83368                | 1.00000        | 0.00000      |
|            | 16        | 0.30564              | 16.25510     | -128.93800     | 2.3838                 | 1.00000        | 0.00000      |
|            | 17        | 1.17873              | 16.07090     | -122.11800     | 2.1606                 | 1.00000        | 0.00000      |
|            | 18        | 0.64729              | 19.08360     | -124.30000     | 2.442                  | 1.00000        | 0.00000      |
|            | 19        | 0.30569              | 20.87490     | -130.46100     | 2.0766                 | 1.00000        | 0.00000      |
|            | 20        | 0.49408              | 22.41190     | -126.06200     | 3.234                  | 1.00000        | 0.00000      |
|            | 21        | 0.19582              | 26.11580     | -126.49200     | 2.0038                 | 1.00000        | 0.00000      |
|            | 22        | 0.04849              | 28.84750     | -129.74700     | 1.1995                 | 1.00000        | 0.00000      |
|            | 23        | 0.37931              | 10.23620     | -113.71300     | 1.352                  | 1.00000        | 0.00000      |
|            | 24        | 0.23086              | 11.71640     | -126.13300     | 1.0759                 | 1.00000        | 0.00000      |
|            | 25        | 0.44327              | 10.27760     | -128.83100     | 1.7985                 | 1.00000        | 0.00000      |
| 2009_10_25 | 0         | 4.34062              | 0.32190      | 52.48250       | 0.24107                | 1.00000        | 0.00000      |
|            | 1         | 2.77567              | 0.47583      | -157.11700     | 0.24066                | 1.00000        | 0.00000      |
|            | 2         | 6.69811              | 1.15299      | -141.58800     | 0.62011                | 1.00000        | 0.00000      |

Continued on next page

Table 14 – continued from previous page

| Epoch      | Component | Flux density<br>(Jy) | Rad<br>(mas) | Theta<br>(deg) | Major<br>axis<br>(mas) | Axial<br>ratio | Phi<br>(deg) |
|------------|-----------|----------------------|--------------|----------------|------------------------|----------------|--------------|
|            | 3         | 0.76517              | 2.94311      | -120.29600     | 1.6921                 | 1.00000        | 0.00000      |
|            | 4         | 4.14200              | 2.62036      | -146.96000     | 0.47097                | 1.00000        | 0.00000      |
|            | 5         | 0.91313              | 3.68262      | -142.27600     | 0.43267                | 1.00000        | 0.00000      |
|            | 6         | 0.22875              | 4.82481      | -119.03900     | 0.97821                | 1.00000        | 0.00000      |
|            | 7         | 1.05200              | 4.38846      | -139.30100     | 0.38385                | 1.00000        | 0.00000      |
|            | 8         | 1.32525              | 5.09955      | -134.26600     | 1.2728                 | 1.00000        | 0.00000      |
|            | 9         | 0.40781              | 6.52380      | -138.21900     | 0                      | 1.00000        | 0.00000      |
|            | 10        | 1.51667              | 6.79324      | -120.47700     | 1.8349                 | 1.00000        | 0.00000      |
|            | 11        | 0.94332              | 7.40482      | -132.20900     | 1.0334                 | 1.00000        | 0.00000      |
|            | 12        | 0.26225              | 8.29769      | -115.64900     | 1.2254                 | 1.00000        | 0.00000      |
|            | 13        | 0.10138              | 8.81704      | -136.51800     | 0                      | 1.00000        | 0.00000      |
|            | 14        | 0.34570              | 10.34580     | -130.50400     | 1.4226                 | 1.00000        | 0.00000      |
|            | 15        | 0.34843              | 10.41230     | -114.37700     | 1.1537                 | 1.00000        | 0.00000      |
|            | 16        | 0.33107              | 11.68860     | -126.18900     | 1.1487                 | 1.00000        | 0.00000      |
|            | 17        | 0.58580              | 11.84780     | -117.93200     | 1.2447                 | 1.00000        | 0.00000      |
|            | 18        | 0.55114              | 13.62340     | -120.14900     | 1.7045                 | 1.00000        | 0.00000      |
|            | 19        | 0.52124              | 14.71780     | -117.60200     | 0.87081                | 1.00000        | 0.00000      |
|            | 20        | 0.75303              | 15.84020     | -120.12200     | 1.594                  | 1.00000        | 0.00000      |
|            | 21        | 1.26064              | 16.69380     | -125.37400     | 2.9527                 | 1.00000        | 0.00000      |
|            | 22        | 0.27304              | 19.18110     | -123.56800     | 1.3565                 | 1.00000        | 0.00000      |
|            | 23        | 0.04998              | 20.79200     | -122.84500     | 0.22296                | 1.00000        | 0.00000      |
|            | 24        | 0.75006              | 21.12870     | -129.06700     | 2.8123                 | 1.00000        | 0.00000      |
|            | 25        | 0.12940              | 23.07860     | -124.67800     | 1.2209                 | 1.00000        | 0.00000      |
|            | 26        | 0.33021              | 25.92400     | -127.47300     | 2.9673                 | 1.00000        | 0.00000      |
|            | 27        | 0.04054              | 29.39360     | -130.87300     | 1.3998                 | 1.00000        | 0.00000      |
| 2009_12_05 | 0         | 3.97375              | 0.40792      | 41.85040       | 0.15638                | 1.00000        | 0.00000      |
|            | 1         | 2.95167              | 0.20088      | -145.52100     | 0.21328                | 1.00000        | 0.00000      |
|            | 2         | 6.88133              | 1.09576      | -139.42200     | 0.63653                | 1.00000        | 0.00000      |
|            | 3         | 1.04465              | 3.18075      | -124.02200     | 1.9014                 | 1.00000        | 0.00000      |
|            | 4         | 3.92104              | 2.56397      | -145.11200     | 0.4569                 | 1.00000        | 0.00000      |
|            | 5         | 0.69445              | 3.37502      | -141.11300     | 0.33979                | 1.00000        | 0.00000      |
|            | 6         | 0.50658              | 5.02962      | -125.46700     | 0.68336                | 1.00000        | 0.00000      |
|            | 7         | 1.38501              | 4.36542      | -139.07900     | 0.52214                | 1.00000        | 0.00000      |
|            | 8         | 0.43283              | 5.22188      | -137.04700     | 0.39538                | 1.00000        | 0.00000      |
|            | 9         | 0.49797              | 6.42006      | -137.40700     | 0                      | 1.00000        | 0.00000      |
|            | 10        | 1.47469              | 6.60389      | -120.16300     | 1.9022                 | 1.00000        | 0.00000      |
|            | 11        | 0.91815              | 7.45347      | -131.70000     | 1.0124                 | 1.00000        | 0.00000      |
|            | 12        | 0.42052              | 7.95280      | -115.31100     | 1.5555                 | 1.00000        | 0.00000      |
|            | 13        | 0.06530              | 8.88649      | -137.14300     | 0                      | 1.00000        | 0.00000      |
|            | 14        | 0.48975              | 10.36800     | -128.29400     | 2.3175                 | 1.00000        | 0.00000      |
|            | 15        | 0.25324              | 10.41870     | -114.48200     | 0.76529                | 1.00000        | 0.00000      |
|            | 16        | 0.30820              | 11.79930     | -125.30900     | 1.2278                 | 1.00000        | 0.00000      |
|            | 17        | 0.40173              | 11.62160     | -115.42900     | 0.92851                | 1.00000        | 0.00000      |
|            | 18        | 0.56142              | 13.04790     | -119.94500     | 1.5558                 | 1.00000        | 0.00000      |
|            | 19        | 0.79263              | 14.75780     | -118.00300     | 1.0521                 | 1.00000        | 0.00000      |
|            | 20        | 0.37850              | 15.97500     | -119.06100     | 1.0645                 | 1.00000        | 0.00000      |
|            | 21        | 1.53590              | 16.65150     | -124.63400     | 3.0133                 | 1.00000        | 0.00000      |
|            | 22        | 0.25898              | 19.33890     | -123.72700     | 1.1415                 | 1.00000        | 0.00000      |
|            | 23        | 0.05806              | 20.69650     | -122.39600     | 0                      | 1.00000        | 0.00000      |
|            | 24        | 0.63763              | 21.26590     | -129.29300     | 2.4266                 | 1.00000        | 0.00000      |
|            | 25        | 0.16398              | 22.96380     | -124.46600     | 1.4745                 | 1.00000        | 0.00000      |
|            | 26        | 0.28258              | 25.86830     | -126.98500     | 2.6707                 | 1.00000        | 0.00000      |
|            | 27        | 0.07433              | 29.33750     | -129.16500     | 2.8542                 | 1.00000        | 0.00000      |
|            | 28        | 0.09021              | 44.35460     | -134.28600     | 6.7139                 | 1.00000        | 0.00000      |
|            | 29        | 0.05516              | 24.61200     | -135.04000     | 1.7327                 | 1.00000        | 0.00000      |
|            | 30        | 0.02771              | 34.47740     | -134.99800     | 2.6313                 | 1.00000        | 0.00000      |
| 2010_01_26 | 0         | 5.12780              | 0.36970      | 41.39650       | 0.19621                | 1.00000        | 0.00000      |

Continued on next page

Table 14 – continued from previous page

| Epoch | Component | Flux density<br>(Jy) | Rad<br>(mas) | Theta<br>(deg) | Major<br>axis<br>(mas) | Axial<br>ratio | Phi<br>(deg) |
|-------|-----------|----------------------|--------------|----------------|------------------------|----------------|--------------|
|       | 1         | 2.84351              | 0.37506      | -144.70900     | 0.13422                | 1.00000        | 0.00000      |
|       | 2         | 6.91891              | 1.21052      | -140.09300     | 0.70169                | 1.00000        | 0.00000      |
|       | 3         | 4.24969              | 2.68900      | -143.90000     | 0.51748                | 1.00000        | 0.00000      |
|       | 4         | 0.45895              | 3.00061      | -111.33900     | 1.0208                 | 1.00000        | 0.00000      |
|       | 5         | 2.02043              | 4.29892      | -137.45600     | 0.88296                | 1.00000        | 0.00000      |
|       | 6         | 1.34980              | 5.43256      | -132.38900     | 1.5045                 | 1.00000        | 0.00000      |
|       | 7         | 2.52294              | 7.16835      | -120.23600     | 2.6577                 | 1.00000        | 0.00000      |
|       | 8         | 0.88189              | 7.38192      | -132.91000     | 1.2176                 | 1.00000        | 0.00000      |
|       | 9         | 0.18211              | 10.56510     | -136.49600     | 0.28006                | 1.00000        | 0.00000      |
|       | 10        | 1.80537              | 11.93390     | -119.54200     | 2.4879                 | 1.00000        | 0.00000      |
|       | 11        | 1.00821              | 14.97020     | -117.71700     | 1.1357                 | 1.00000        | 0.00000      |
|       | 12        | 1.75309              | 16.55130     | -123.35500     | 2.7357                 | 1.00000        | 0.00000      |
|       | 13        | 1.40056              | 20.78120     | -127.29100     | 3.9538                 | 1.00000        | 0.00000      |
|       | 14        | 0.40968              | 26.07220     | -127.72200     | 3.4985                 | 1.00000        | 0.00000      |

Table 15: Modelfit parameters for all epochs. 8.4 GHz data.

| Epoch      | Component | Flux density<br>(Jy) | Rad<br>(mas) | Theta<br>(deg) | Major<br>axis<br>(mas) | Axial<br>ratio | Phi<br>(deg) |
|------------|-----------|----------------------|--------------|----------------|------------------------|----------------|--------------|
| 2009_08_28 | 0         | 3.60776              | 0.11526      | 64.03790       | 0.18007                | 1.00000        | 0.00000      |
|            | 1         | 2.95685              | 0.66541      | -148.41700     | 0.20019                | 1.00000        | 0.00000      |
|            | 2         | 7.08911              | 1.32642      | -140.30800     | 0.58533                | 1.00000        | 0.00000      |
|            | 3         | 4.11378              | 2.76567      | -146.10800     | 0.4813                 | 1.00000        | 0.00000      |
|            | 4         | 0.64376              | 3.06733      | -121.60500     | 1.5315                 | 1.00000        | 0.00000      |
|            | 5         | 1.18878              | 3.90981      | -142.21100     | 0.41                   | 1.00000        | 0.00000      |
|            | 6         | 0.89808              | 4.60413      | -139.89100     | 0                      | 1.00000        | 0.00000      |
|            | 7         | 0.50220              | 4.73431      | -123.12300     | 1.5216                 | 1.00000        | 0.00000      |
|            | 8         | 1.05314              | 5.24301      | -134.80600     | 0.91988                | 1.00000        | 0.00000      |
|            | 9         | 0.42311              | 6.60645      | -138.46100     | 0                      | 1.00000        | 0.00000      |
|            | 10        | 1.75472              | 7.14412      | -120.86700     | 2.2412                 | 1.00000        | 0.00000      |
|            | 11        | 0.78878              | 7.17651      | -131.06800     | 0.91412                | 1.00000        | 0.00000      |
|            | 12        | 0.32342              | 8.26200      | -135.87800     | 0.90233                | 1.00000        | 0.00000      |
|            | 13        | 0.20691              | 10.52560     | -113.74100     | 1.2472                 | 1.00000        | 0.00000      |
|            | 14        | 0.98807              | 11.18170     | -126.22200     | 2.7765                 | 1.00000        | 0.00000      |
|            | 15        | 0.45569              | 11.78420     | -117.49300     | 1.1677                 | 1.00000        | 0.00000      |
|            | 16        | 0.45949              | 13.63480     | -119.96200     | 1.4562                 | 1.00000        | 0.00000      |
|            | 17        | 0.63241              | 14.86520     | -118.39200     | 0.91461                | 1.00000        | 0.00000      |
|            | 18        | 0.43635              | 15.83620     | -118.91800     | 1.0558                 | 1.00000        | 0.00000      |
|            | 19        | 1.45920              | 16.70470     | -124.62000     | 2.6553                 | 1.00000        | 0.00000      |
|            | 20        | 0.34607              | 19.71720     | -123.90400     | 1.8845                 | 1.00000        | 0.00000      |
|            | 21        | 0.70069              | 21.30460     | -129.36100     | 2.9577                 | 1.00000        | 0.00000      |
|            | 22        | 0.12794              | 23.06920     | -124.93700     | 1.478                  | 1.00000        | 0.00000      |
|            | 23        | 0.34990              | 26.14740     | -127.38900     | 3.3776                 | 1.00000        | 0.00000      |
| 2009_10_25 | 0         | 4.43096              | 0.25658      | 78.72000       | 0.22804                | 1.00000        | 0.00000      |
|            | 1         | 3.12642              | 0.61031      | -161.94000     | 0.29458                | 1.00000        | 0.00000      |
|            | 2         | 6.51826              | 1.29128      | -145.27400     | 0.58598                | 1.00000        | 0.00000      |
|            | 3         | 0.22530              | 2.24740      | -118.57400     | 0.52242                | 1.00000        | 0.00000      |
|            | 4         | 4.07409              | 2.75013      | -148.88900     | 0.45628                | 1.00000        | 0.00000      |
|            | 5         | 0.92473              | 3.52016      | -141.92000     | 0.39733                | 1.00000        | 0.00000      |
|            | 6         | 0.48953              | 3.70147      | -117.08700     | 1.3185                 | 1.00000        | 0.00000      |
|            | 7         | 1.37339              | 4.46185      | -141.77800     | 0.56068                | 1.00000        | 0.00000      |
|            | 8         | 1.12062              | 5.21325      | -134.95300     | 0.9209                 | 1.00000        | 0.00000      |
|            | 9         | 0.37223              | 6.66921      | -139.94700     | 0                      | 1.00000        | 0.00000      |
|            | 10        | 2.00973              | 6.78612      | -123.86400     | 2.0619                 | 1.00000        | 0.00000      |
|            | 11        | 0.63040              | 7.57136      | -133.70300     | 0.77864                | 1.00000        | 0.00000      |

Continued on next page

Table 15 – continued from previous page

| Epoch      | Component | Flux density<br>(Jy) | Rad<br>(mas) | Theta<br>(deg) | Major<br>axis<br>(mas) | Axial<br>ratio | Phi<br>(deg) |
|------------|-----------|----------------------|--------------|----------------|------------------------|----------------|--------------|
|            | 12        | 0.26580              | 8.19253      | -116.42300     | 1.1698                 | 1.00000        | 0.00000      |
|            | 13        | 0.13608              | 8.82530      | -137.25700     | 0.77335                | 1.00000        | 0.00000      |
|            | 14        | 0.27980              | 10.35330     | -131.27300     | 1.2774                 | 1.00000        | 0.00000      |
|            | 15        | 0.34492              | 10.44460     | -115.29800     | 1.2637                 | 1.00000        | 0.00000      |
|            | 16        | 0.37449              | 11.67930     | -127.03000     | 1.2444                 | 1.00000        | 0.00000      |
|            | 17        | 0.56046              | 11.92430     | -118.41900     | 1.2676                 | 1.00000        | 0.00000      |
|            | 18        | 0.48173              | 13.54360     | -120.78000     | 1.7349                 | 1.00000        | 0.00000      |
|            | 19        | 0.67873              | 14.83840     | -118.58000     | 1.0195                 | 1.00000        | 0.00000      |
|            | 20        | 0.42746              | 15.99800     | -119.99600     | 1.1915                 | 1.00000        | 0.00000      |
|            | 21        | 1.42501              | 16.66700     | -125.10100     | 2.8636                 | 1.00000        | 0.00000      |
|            | 22        | 0.21243              | 19.23350     | -124.07700     | 1.1168                 | 1.00000        | 0.00000      |
|            | 23        | 0.05818              | 20.57630     | -122.84800     | 0.43077                | 1.00000        | 0.00000      |
|            | 24        | 0.78537              | 21.17280     | -129.22200     | 2.9413                 | 1.00000        | 0.00000      |
|            | 25        | 0.09855              | 23.02070     | -124.55700     | 1.1089                 | 1.00000        | 0.00000      |
|            | 26        | 0.32566              | 25.81950     | -127.47100     | 3.0463                 | 1.00000        | 0.00000      |
|            | 27        | 0.05053              | 29.13830     | -130.92100     | 1.7986                 | 1.00000        | 0.00000      |
| 2009_12_05 | 0         | 4.28365              | 0.38650      | 34.45680       | 0.14136                | 1.00000        | 0.00000      |
|            | 1         | 3.14161              | 0.25616      | -134.81800     | 0.22205                | 1.00000        | 0.00000      |
|            | 2         | 6.68060              | 1.13670      | -137.00900     | 0.62274                | 1.00000        | 0.00000      |
|            | 3         | 1.07687              | 3.12157      | -122.38400     | 1.9172                 | 1.00000        | 0.00000      |
|            | 4         | 3.90914              | 2.58382      | -143.80400     | 0.4608                 | 1.00000        | 0.00000      |
|            | 5         | 0.65950              | 3.46598      | -141.59700     | 0.36974                | 1.00000        | 0.00000      |
|            | 6         | 0.55662              | 5.09390      | -125.95400     | 0.58534                | 1.00000        | 0.00000      |
|            | 7         | 1.38347              | 4.36087      | -137.93300     | 0.51979                | 1.00000        | 0.00000      |
|            | 8         | 0.37993              | 5.22202      | -137.45100     | 0.36401                | 1.00000        | 0.00000      |
|            | 9         | 0.54350              | 6.40710      | -136.61300     | 0.31601                | 1.00000        | 0.00000      |
|            | 10        | 1.15307              | 6.59997      | -118.71200     | 1.6795                 | 1.00000        | 0.00000      |
|            | 11        | 0.97900              | 7.42373      | -130.91800     | 1.0375                 | 1.00000        | 0.00000      |
|            | 12        | 0.51786              | 7.97551      | -115.50600     | 1.4416                 | 1.00000        | 0.00000      |
|            | 13        | 0.08777              | 8.72012      | -135.53800     | 0                      | 1.00000        | 0.00000      |
|            | 14        | 0.45151              | 10.30820     | -128.80400     | 1.9923                 | 1.00000        | 0.00000      |
|            | 15        | 0.32702              | 10.57310     | -114.55300     | 1.0479                 | 1.00000        | 0.00000      |
|            | 16        | 0.29801              | 11.81210     | -125.26800     | 1.1643                 | 1.00000        | 0.00000      |
|            | 17        | 0.34009              | 11.75560     | -115.35600     | 0.89539                | 1.00000        | 0.00000      |
|            | 18        | 0.54604              | 13.03410     | -119.84900     | 1.6098                 | 1.00000        | 0.00000      |
|            | 19        | 0.82148              | 14.81170     | -117.86300     | 1.1814                 | 1.00000        | 0.00000      |
|            | 20        | 0.41174              | 16.03190     | -119.22200     | 1.1926                 | 1.00000        | 0.00000      |
|            | 21        | 1.38080              | 16.74050     | -124.60700     | 2.8892                 | 1.00000        | 0.00000      |
|            | 22        | 0.18304              | 19.24810     | -123.60200     | 1.0762                 | 1.00000        | 0.00000      |
|            | 23        | 0.07068              | 20.53920     | -122.20500     | 0.77556                | 1.00000        | 0.00000      |
|            | 24        | 0.70215              | 21.08390     | -128.91600     | 2.7855                 | 1.00000        | 0.00000      |
|            | 25        | 0.14361              | 23.02400     | -124.51800     | 1.3896                 | 1.00000        | 0.00000      |
|            | 26        | 0.32432              | 25.82740     | -127.57300     | 3.0755                 | 1.00000        | 0.00000      |
|            | 27        | 0.04407              | 30.15440     | -128.38000     | 2.1926                 | 1.00000        | 0.00000      |
| 2010_01_26 | 0         | 4.29675              | 0.42884      | 40.63320       | 0.11526                | 1.00000        | 0.00000      |
|            | 1         | 3.18783              | 0.28057      | -144.24700     | 0.23066                | 1.00000        | 0.00000      |
|            | 2         | 5.95727              | 1.20280      | -140.06800     | 0.67236                | 1.00000        | 0.00000      |
|            | 3         | 3.66166              | 2.68828      | -143.88400     | 0.5003                 | 1.00000        | 0.00000      |
|            | 4         | 0.57028              | 2.97954      | -114.74300     | 1.252                  | 1.00000        | 0.00000      |
|            | 5         | 1.56873              | 4.25314      | -137.44900     | 0.83378                | 1.00000        | 0.00000      |
|            | 6         | 1.26294              | 5.31628      | -132.10900     | 1.4383                 | 1.00000        | 0.00000      |
|            | 7         | 0.95805              | 7.17021      | -132.58800     | 1.3483                 | 1.00000        | 0.00000      |
|            | 8         | 1.98353              | 7.24840      | -119.13500     | 2.5936                 | 1.00000        | 0.00000      |
|            | 9         | 0.16917              | 10.27750     | -136.18900     | 0.28215                | 1.00000        | 0.00000      |
|            | 10        | 1.59016              | 11.91360     | -119.58800     | 2.5127                 | 1.00000        | 0.00000      |
|            | 11        | 0.88350              | 14.98460     | -117.85400     | 1.1311                 | 1.00000        | 0.00000      |
|            | 12        | 1.48546              | 16.54280     | -123.35500     | 2.7767                 | 1.00000        | 0.00000      |

Continued on next page



Table 15 – continued from previous page

| Epoch | Component | Flux density<br>(Jy) | Rad<br>(mas) | Theta<br>(deg) | Major<br>axis<br>(mas) | Axial<br>ratio | Phi<br>(deg) |
|-------|-----------|----------------------|--------------|----------------|------------------------|----------------|--------------|
|       | 13        | 1.21226              | 20.75940     | -127.08700     | 3.9612                 | 1.00000        | 0.00000      |
|       | 14        | 0.40733              | 26.29160     | -128.27400     | 4.4865                 | 1.00000        | 0.00000      |

Table 16: Modelfit parameters for all epochs. 15.4 GHz data.

| Epoch      | Component | Flux density<br>(Jy) | Rad<br>(mas) | Theta<br>(deg) | Major<br>axis<br>(mas) | Axial<br>ratio | Phi<br>(deg) |
|------------|-----------|----------------------|--------------|----------------|------------------------|----------------|--------------|
| 2009_08_28 | 0         | 3.06823              | 0.18284      | 57.27830       | 0                      | 1.00000        | 0.00000      |
|            | 1         | 5.10380              | 0.19266      | -175.15000     | 0.12804                | 1.00000        | 0.00000      |
|            | 2         | 3.46831              | 1.02181      | -149.71100     | 0.40645                | 1.00000        | 0.00000      |
|            | 3         | 1.20052              | 1.44013      | -134.32600     | 0.24653                | 1.00000        | 0.00000      |
|            | 4         | 2.98236              | 1.66172      | -143.62500     | 0.5668                 | 1.00000        | 0.00000      |
|            | 5         | 2.62848              | 2.94393      | -147.98600     | 0.31233                | 1.00000        | 0.00000      |
|            | 6         | 0.93457              | 3.02914      | -140.41100     | 0.87756                | 1.00000        | 0.00000      |
|            | 7         | 0.29605              | 3.90407      | -116.05400     | 1.6039                 | 1.00000        | 0.00000      |
|            | 8         | 0.61835              | 3.99318      | -142.49400     | 0.39936                | 1.00000        | 0.00000      |
|            | 9         | 0.54887              | 4.58144      | -141.79800     | 0.33515                | 1.00000        | 0.00000      |
|            | 10        | 1.17502              | 5.08876      | -136.83700     | 1.063                  | 1.00000        | 0.00000      |
|            | 11        | 0.30646              | 6.78805      | -139.40300     | 0.66449                | 1.00000        | 0.00000      |
|            | 12        | 1.61377              | 7.09228      | -125.95700     | 2.0069                 | 1.00000        | 0.00000      |
|            | 13        | 0.21518              | 7.78861      | -134.70900     | 0.2782                 | 1.00000        | 0.00000      |
|            | 14        | 0.18028              | 8.69480      | -134.37000     | 0.96613                | 1.00000        | 0.00000      |
|            | 15        | 0.96806              | 11.73450     | -120.64300     | 2.8295                 | 1.00000        | 0.00000      |
|            | 16        | 0.62774              | 15.14990     | -119.32100     | 1.4644                 | 1.00000        | 0.00000      |
|            | 17        | 0.73813              | 16.68480     | -123.57900     | 2.2956                 | 1.00000        | 0.00000      |
|            | 18        | 0.43198              | 20.80890     | -127.15700     | 2.9425                 | 1.00000        | 0.00000      |
| 2009_10_25 | 0         | 2.52987              | 0.19943      | 64.70120       | 0                      | 1.00000        | 0.00000      |
|            | 1         | 3.44077              | 0.22737      | -178.58100     | 0                      | 1.00000        | 0.00000      |
|            | 2         | 3.02081              | 0.35982      | -155.44900     | 0.23676                | 1.00000        | 0.00000      |
|            | 3         | 3.04091              | 1.16730      | -149.87100     | 0.36508                | 1.00000        | 0.00000      |
|            | 4         | 1.11355              | 1.48034      | -133.03700     | 0                      | 1.00000        | 0.00000      |
|            | 5         | 0.73874              | 1.76376      | -153.99200     | 0.23088                | 1.00000        | 0.00000      |
|            | 6         | 1.78840              | 1.91710      | -141.18000     | 0.34688                | 1.00000        | 0.00000      |
|            | 7         | 0.36217              | 2.70963      | -132.58800     | 0.44366                | 1.00000        | 0.00000      |
|            | 8         | 0.81818              | 2.94121      | -149.55500     | 0                      | 1.00000        | 0.00000      |
|            | 9         | 2.05510              | 3.17223      | -147.06100     | 0.28276                | 1.00000        | 0.00000      |
|            | 10        | 0.50840              | 3.75481      | -141.48000     | 0.3898                 | 1.00000        | 0.00000      |
|            | 11        | 0.34125              | 3.92562      | -118.59500     | 1.6404                 | 1.00000        | 0.00000      |
|            | 12        | 0.93739              | 4.63205      | -141.57600     | 0.57776                | 1.00000        | 0.00000      |
|            | 13        | 0.88718              | 5.29057      | -136.13700     | 1.0351                 | 1.00000        | 0.00000      |
|            | 14        | 0.26877              | 6.95431      | -138.85400     | 0.53609                | 1.00000        | 0.00000      |
|            | 15        | 1.79481              | 7.20847      | -125.58700     | 2.31                   | 1.00000        | 0.00000      |
|            | 16        | 0.20759              | 7.91669      | -134.58000     | 0.36268                | 1.00000        | 0.00000      |
|            | 17        | 0.19003              | 11.26300     | -130.80200     | 1.3174                 | 1.00000        | 0.00000      |
|            | 18        | 0.94731              | 12.11030     | -119.75600     | 2.5294                 | 1.00000        | 0.00000      |
|            | 19        | 0.37138              | 15.09500     | -118.69500     | 1.0182                 | 1.00000        | 0.00000      |
|            | 20        | 0.30269              | 16.24370     | -120.37800     | 1.4514                 | 1.00000        | 0.00000      |
|            | 21        | 0.82214              | 16.93830     | -124.86100     | 2.8772                 | 1.00000        | 0.00000      |
|            | 22        | 0.52838              | 21.43140     | -127.68600     | 3.1557                 | 1.00000        | 0.00000      |
|            | 23        | 0.10642              | 27.07750     | -126.52700     | 1.5719                 | 1.00000        | 0.00000      |
|            | 24        | 0.12499              | 8.69302      | -136.22500     | 0.65277                | 1.00000        | 0.00000      |
| 2009_12_05 | 0         | 2.51418              | 0.27828      | 46.39260       | 0.027273               | 1.00000        | 0.00000      |
|            | 1         | 3.56775              | 0.13015      | -177.36300     | 0                      | 1.00000        | 0.00000      |
|            | 2         | 3.29949              | 0.36578      | -149.31200     | 0.20179                | 1.00000        | 0.00000      |
|            | 3         | 2.68297              | 1.17132      | -147.29300     | 0.35884                | 1.00000        | 0.00000      |

Continued on next page

Table 16 – continued from previous page

| Epoch      | Component | Flux density<br>(Jy) | Rad<br>(mas) | Theta<br>(deg) | Major<br>axis<br>(mas) | Axial<br>ratio | Phi<br>(deg) |
|------------|-----------|----------------------|--------------|----------------|------------------------|----------------|--------------|
|            | 4         | 0.94769              | 1.45244      | -131.78600     | 0                      | 1.00000        | 0.00000      |
|            | 5         | 1.10094              | 1.77953      | -149.21700     | 0.39215                | 1.00000        | 0.00000      |
|            | 6         | 1.15739              | 1.85295      | -136.79900     | 0.26742                | 1.00000        | 0.00000      |
|            | 7         | 0.45345              | 2.68381      | -129.62400     | 0.9856                 | 1.00000        | 0.00000      |
|            | 8         | 0.34409              | 2.70890      | -148.78000     | 0                      | 1.00000        | 0.00000      |
|            | 9         | 2.50953              | 3.09957      | -146.01200     | 0.29964                | 1.00000        | 0.00000      |
|            | 10        | 0.53856              | 3.70017      | -140.16600     | 0.48623                | 1.00000        | 0.00000      |
|            | 11        | 0.21462              | 3.91927      | -114.85500     | 1.0181                 | 1.00000        | 0.00000      |
|            | 12        | 0.87207              | 4.63723      | -140.71100     | 0.51588                | 1.00000        | 0.00000      |
|            | 13        | 0.71531              | 5.21819      | -135.99500     | 0.79866                | 1.00000        | 0.00000      |
|            | 14        | 0.30097              | 6.77605      | -136.86700     | 0.55482                | 1.00000        | 0.00000      |
|            | 15        | 1.64083              | 7.27639      | -124.15000     | 2.2277                 | 1.00000        | 0.00000      |
|            | 16        | 0.15411              | 7.94023      | -133.85400     | 0.35292                | 1.00000        | 0.00000      |
|            | 17        | 0.19537              | 11.33630     | -129.65800     | 1.1592                 | 1.00000        | 0.00000      |
|            | 18        | 0.85420              | 12.17000     | -119.53200     | 2.2207                 | 1.00000        | 0.00000      |
|            | 19        | 0.39482              | 15.10840     | -118.29600     | 1.0144                 | 1.00000        | 0.00000      |
|            | 20        | 0.20156              | 16.24960     | -120.23400     | 1.0914                 | 1.00000        | 0.00000      |
|            | 21        | 0.91387              | 17.00080     | -124.26800     | 2.9532                 | 1.00000        | 0.00000      |
|            | 22        | 0.52607              | 21.53120     | -127.11700     | 2.8881                 | 1.00000        | 0.00000      |
|            | 23        | 0.13776              | 26.97930     | -128.58600     | 1.9797                 | 1.00000        | 0.00000      |
|            | 24        | 0.25192              | 8.51079      | -135.36700     | 1.4444                 | 1.00000        | 0.00000      |
|            | 25        | 0.12712              | 5.41992      | -122.42800     | 0.46295                | 1.00000        | 0.00000      |
| 2010_01_26 | 0         | 3.92088              | 0.19826      | 52.85920       | 0.050758               | 1.00000        | 0.00000      |
|            | 1         | 4.63989              | 0.36333      | -151.50000     | 0.16418                | 1.00000        | 0.00000      |
|            | 2         | 0.10013              | 0.62262      | -97.78700      | 4.942e-08              | 1.00000        | 0.00000      |
|            | 3         | 1.17170              | 1.12706      | -150.57900     | 0.11702                | 1.00000        | 0.00000      |
|            | 4         | 4.52161              | 1.60864      | -140.58700     | 0.69104                | 1.00000        | 0.00000      |
|            | 5         | 2.85314              | 3.14558      | -145.30600     | 0.41693                | 1.00000        | 0.00000      |
|            | 6         | 0.45913              | 3.39108      | -131.74700     | 0.35272                | 1.00000        | 0.00000      |
|            | 7         | 0.14949              | 4.34627      | -115.43200     | 0.20066                | 1.00000        | 0.00000      |
|            | 8         | 0.98651              | 4.72687      | -140.77200     | 0.52721                | 1.00000        | 0.00000      |
|            | 9         | 0.53196              | 5.34346      | -136.29600     | 0.73525                | 1.00000        | 0.00000      |
|            | 10        | 0.13025              | 6.70000      | -137.87900     | 0.025097               | 1.00000        | 0.00000      |
|            | 11        | 1.94142              | 7.22455      | -125.99100     | 2.4771                 | 1.00000        | 0.00000      |
|            | 12        | 0.23206              | 8.28929      | -134.38300     | 0.45083                | 1.00000        | 0.00000      |
|            | 13        | 1.02094              | 12.07250     | -121.02300     | 3.0096                 | 1.00000        | 0.00000      |
|            | 14        | 0.55114              | 15.40450     | -119.06400     | 1.4125                 | 1.00000        | 0.00000      |
|            | 15        | 0.69315              | 17.10450     | -124.38100     | 2.3233                 | 1.00000        | 0.00000      |
|            | 16        | 0.07213              | 19.68500     | -123.45000     | 0.057481               | 1.00000        | 0.00000      |
|            | 17        | 0.24388              | 21.69460     | -127.83100     | 1.6946                 | 1.00000        | 0.00000      |

Table 17: Modelfit parameters for all epochs. 23.8 GHz data.

| Epoch      | Component | Flux density<br>(Jy) | Rad<br>(mas) | Theta<br>(deg) | Major<br>axis<br>(mas) | Axial<br>ratio | Phi<br>(deg) |
|------------|-----------|----------------------|--------------|----------------|------------------------|----------------|--------------|
| 2009_08_28 | 0         | 2.60901              | 0.07257      | 31.13290       | 0.14862                | 1.00000        | 0.00000      |
|            | 1         | 3.59651              | 0.19132      | -148.07200     | 0.095285               | 1.00000        | 0.00000      |
|            | 2         | 2.15969              | 0.40725      | -145.90500     | 0.10573                | 1.00000        | 0.00000      |
|            | 3         | 0.51877              | 0.93264      | -131.02500     | 0.43928                | 1.00000        | 0.00000      |
|            | 4         | 1.68163              | 1.27416      | -149.48300     | 0.32325                | 1.00000        | 0.00000      |
|            | 5         | 0.62049              | 1.55909      | -133.05500     | 0.15511                | 1.00000        | 0.00000      |
|            | 6         | 2.37090              | 1.80220      | -139.87300     | 0.53683                | 1.00000        | 0.00000      |
|            | 7         | 2.09578              | 3.10967      | -146.58500     | 0.31417                | 1.00000        | 0.00000      |
|            | 8         | 0.34933              | 3.20028      | -135.63400     | 0.52987                | 1.00000        | 0.00000      |
|            | 9         | 0.16946              | 3.96532      | -118.15700     | 0.9216                 | 1.00000        | 0.00000      |

Continued on next page

Table 17 – continued from previous page

| Epoch      | Component | Flux density<br>(Jy) | Rad<br>(mas) | Theta<br>(deg) | Major<br>axis<br>(mas) | Axial<br>ratio | Phi<br>(deg) |
|------------|-----------|----------------------|--------------|----------------|------------------------|----------------|--------------|
|            | 10        | 0.27991              | 4.09003      | -142.56800     | 0.14755                | 1.00000        | 0.00000      |
|            | 11        | 0.47554              | 4.52051      | -140.75500     | 0.39905                | 1.00000        | 0.00000      |
|            | 12        | 0.79116              | 5.11704      | -137.14500     | 0.97797                | 1.00000        | 0.00000      |
|            | 13        | 0.12654              | 7.07092      | -138.02300     | 0.26658                | 1.00000        | 0.00000      |
|            | 14        | 0.94893              | 7.08859      | -127.19400     | 1.874                  | 1.00000        | 0.00000      |
|            | 15        | 0.22815              | 8.18445      | -135.54300     | 0.74747                | 1.00000        | 0.00000      |
|            | 16        | 0.27726              | 11.95380     | -118.09500     | 1.5164                 | 1.00000        | 0.00000      |
|            | 17        | 0.41109              | 15.70880     | -119.90500     | 1.655                  | 1.00000        | 0.00000      |
| 2009_10_25 | 0         | 0.91363              | 0.17910      | 48.09210       | 0                      | 1.00000        | 0.00000      |
|            | 1         | 2.70423              | 0.00633      | 87.43600       | 0.099564               | 1.00000        | 0.00000      |
|            | 2         | 2.46246              | 0.28267      | -147.69400     | 0.072133               | 1.00000        | 0.00000      |
|            | 3         | 3.07349              | 0.51292      | -145.57800     | 0.15856                | 1.00000        | 0.00000      |
|            | 4         | 0.99559              | 1.20079      | -140.00000     | 0.44784                | 1.00000        | 0.00000      |
|            | 5         | 1.05700              | 1.45275      | -150.65500     | 0.26405                | 1.00000        | 0.00000      |
|            | 6         | 0.78585              | 1.68252      | -133.35300     | 0.25748                | 1.00000        | 0.00000      |
|            | 7         | 1.84447              | 1.95209      | -140.56300     | 0.5408                 | 1.00000        | 0.00000      |
|            | 8         | 0.27026              | 3.02926      | -148.44400     | 0.054741               | 1.00000        | 0.00000      |
|            | 9         | 1.60975              | 3.27755      | -145.82000     | 0.22152                | 1.00000        | 0.00000      |
|            | 10        | 0.82661              | 3.28942      | -139.87600     | 0.99572                | 1.00000        | 0.00000      |
|            | 11        | 0.21641              | 4.21449      | -142.49300     | 0.24726                | 1.00000        | 0.00000      |
|            | 12        | 0.07780              | 4.50826      | -119.64700     | 0.38276                | 1.00000        | 0.00000      |
|            | 13        | 0.51607              | 4.74660      | -140.25700     | 0.41955                | 1.00000        | 0.00000      |
|            | 14        | 0.68795              | 5.29247      | -135.85100     | 0.97954                | 1.00000        | 0.00000      |
|            | 15        | 0.14572              | 7.18821      | -138.27200     | 0.35616                | 1.00000        | 0.00000      |
|            | 16        | 1.01557              | 7.27889      | -126.63600     | 2.0895                 | 1.00000        | 0.00000      |
|            | 17        | 0.22025              | 8.29436      | -135.03200     | 0.80468                | 1.00000        | 0.00000      |
|            | 18        | 0.33982              | 12.07030     | -118.86700     | 2.1947                 | 1.00000        | 0.00000      |
|            | 19        | 0.13639              | 15.40010     | -118.93500     | 0.73287                | 1.00000        | 0.00000      |
|            | 20        | 0.30091              | 16.35690     | -121.60100     | 1.6801                 | 1.00000        | 0.00000      |
| 2009_12_05 | 0         | 1.72655              | 0.12376      | 70.24520       | 0                      | 1.00000        | 0.00000      |
|            | 1         | 2.66988              | 0.08189      | -159.98200     | 0                      | 1.00000        | 0.00000      |
|            | 2         | 2.52670              | 0.41312      | -151.14100     | 0                      | 1.00000        | 0.00000      |
|            | 3         | 2.67326              | 0.63404      | -145.00900     | 0.12917                | 1.00000        | 0.00000      |
|            | 4         | 0.81379              | 1.29888      | -141.31200     | 0.44624                | 1.00000        | 0.00000      |
|            | 5         | 0.90798              | 1.53896      | -150.26700     | 0.28841                | 1.00000        | 0.00000      |
|            | 6         | 0.27882              | 1.76055      | -134.55700     | 2.6501e-07             | 1.00000        | 0.00000      |
|            | 7         | 1.97153              | 1.97752      | -140.39000     | 0.55746                | 1.00000        | 0.00000      |
|            | 8         | 0.37103              | 3.09700      | -146.63700     | 0.23859                | 1.00000        | 0.00000      |
|            | 9         | 1.51524              | 3.40942      | -145.68900     | 0.23513                | 1.00000        | 0.00000      |
|            | 10        | 0.65048              | 3.02350      | -138.46600     | 1.1134                 | 1.00000        | 0.00000      |
|            | 11        | 0.38920              | 4.08602      | -142.42500     | 0.58603                | 1.00000        | 0.00000      |
|            | 12        | 0.52695              | 4.90001      | -139.74400     | 0.39848                | 1.00000        | 0.00000      |
|            | 13        | 0.58862              | 5.61952      | -135.79600     | 0.91293                | 1.00000        | 0.00000      |
|            | 14        | 0.64276              | 7.43351      | -125.50100     | 1.7053                 | 1.00000        | 0.00000      |
|            | 15        | 0.14452              | 7.27094      | -138.15600     | 0.31235                | 1.00000        | 0.00000      |
|            | 16        | 0.26948              | 8.36337      | -134.39400     | 0.73193                | 1.00000        | 0.00000      |
|            | 17        | 0.17402              | 12.54220     | -119.68200     | 0.74576                | 1.00000        | 0.00000      |
|            | 18        | 0.18289              | 15.48150     | -118.77800     | 0.7208                 | 1.00000        | 0.00000      |
|            | 19        | 0.08542              | 16.85240     | -120.58100     | 0.37981                | 1.00000        | 0.00000      |
|            | 20        | 0.05753              | 11.37260     | -118.47300     | 0.3201                 | 1.00000        | 0.00000      |
|            | 21        | 0.11378              | 4.78395      | -120.38600     | 0.51669                | 1.00000        | 0.00000      |
| 2010_01_26 | 0         | 3.84280              | 0.07162      | 75.79260       | 0                      | 1.00000        | 0.00000      |
|            | 1         | 2.58871              | 0.15524      | -153.29400     | 0                      | 1.00000        | 0.00000      |
|            | 2         | 2.34321              | 0.54601      | -149.90700     | 0                      | 1.00000        | 0.00000      |
|            | 3         | 2.00968              | 0.78238      | -144.11700     | 0.065316               | 1.00000        | 0.00000      |
|            | 4         | 0.98149              | 1.49870      | -140.66200     | 0.41578                | 1.00000        | 0.00000      |
|            | 5         | 0.40383              | 1.90746      | -134.22600     | 0.050603               | 1.00000        | 0.00000      |

Continued on next page

Table 17 – continued from previous page

| Epoch | Component | Flux density<br>(Jy) | Rad<br>(mas) | Theta<br>(deg) | Major<br>axis<br>(mas) | Axial<br>ratio | Phi<br>(deg) |
|-------|-----------|----------------------|--------------|----------------|------------------------|----------------|--------------|
|       | 6         | 2.10064              | 2.08766      | -143.78800     | 0.67437                | 1.00000        | 0.00000      |
|       | 7         | 0.47980              | 3.06363      | -141.95600     | 0.32562                | 1.00000        | 0.00000      |
|       | 8         | 1.40028              | 3.52651      | -145.65500     | 0.22898                | 1.00000        | 0.00000      |
|       | 9         | 0.24058              | 3.54957      | -119.57500     | 0.94742                | 1.00000        | 0.00000      |
|       | 10        | 0.40794              | 4.16789      | -142.44500     | 0.45999                | 1.00000        | 0.00000      |
|       | 11        | 0.13728              | 4.73480      | -126.50400     | 0.46966                | 1.00000        | 0.00000      |
|       | 12        | 0.25325              | 5.03841      | -139.88900     | 0.23084                | 1.00000        | 0.00000      |
|       | 13        | 0.49666              | 5.48939      | -137.40200     | 0.70705                | 1.00000        | 0.00000      |
|       | 14        | 1.22730              | 7.09405      | -129.49700     | 2.1993                 | 1.00000        | 0.00000      |
|       | 15        | 0.18317              | 8.78776      | -134.26200     | 0.65526                | 1.00000        | 0.00000      |
|       | 16        | 0.06392              | 12.28890     | -118.64500     | 0.30902                | 1.00000        | 0.00000      |
|       | 17        | 0.06673              | 13.13530     | -124.26700     | 0.21573                | 1.00000        | 0.00000      |
|       | 18        | 0.09462              | 15.61040     | -118.86200     | 0.69556                | 1.00000        | 0.00000      |
|       | 19        | 0.21936              | 16.91630     | -120.51700     | 1.746                  | 1.00000        | 0.00000      |

Table 18: Modelfit parameters for all epochs. 43.2 GHz, both our data and Boston University data.

| Epoch      | Component | Flux density<br>(Jy) | Rad<br>(mas) | Theta<br>(deg) | Major<br>axis<br>(mas) | Axial<br>ratio | Phi<br>(deg) |
|------------|-----------|----------------------|--------------|----------------|------------------------|----------------|--------------|
| 2008_01_17 | 0         | 0.31375              | 0.56878      | 23.68380       | 0.15966                | 1.00000        | 0.00000      |
|            | 1         | 3.21155              | 0.01308      | -18.03360      | 0.069272               | 1.00000        | 0.00000      |
|            | 2         | 1.92224              | 0.15410      | -143.37300     | 0.32322                | 1.00000        | 0.00000      |
|            | 3         | 1.07777              | 0.25800      | -167.30200     | 0.06302                | 1.00000        | 0.00000      |
|            | 4         | 0.55896              | 0.70443      | -139.48400     | 0.013025               | 1.00000        | 0.00000      |
|            | 5         | 1.16909              | 0.74758      | -153.57100     | 0.099829               | 1.00000        | 0.00000      |
|            | 6         | 4.14909              | 0.85369      | -143.40900     | 0.25081                | 1.00000        | 0.00000      |
|            | 7         | 0.16749              | 1.06325      | -117.43600     | 0.15261                | 1.00000        | 0.00000      |
|            | 8         | 1.03758              | 1.98312      | -135.39200     | 0.33565                | 1.00000        | 0.00000      |
|            | 9         | 0.26386              | 2.06734      | -149.27300     | 0.17724                | 1.00000        | 0.00000      |
|            | 10        | 0.36491              | 3.01310      | -142.86500     | 0.16401                | 1.00000        | 0.00000      |
|            | 11        | 0.35015              | 3.61237      | -145.44000     | 0.30075                | 1.00000        | 0.00000      |
|            | 12        | 0.11072              | 4.49131      | -134.62800     | 0.62172                | 1.00000        | 0.00000      |
|            | 13        | 0.31526              | 5.92286      | -136.82000     | 0.7576                 | 1.00000        | 0.00000      |
| 2008_02_29 | 0         | 5.14351              | 0.01669      | -151.12200     | 0.043325               | 1.00000        | 0.00000      |
|            | 1         | 0.66972              | 0.43751      | -163.02200     | 0                      | 1.00000        | 0.00000      |
|            | 2         | 3.06859              | 0.76450      | -155.12300     | 0.091912               | 1.00000        | 0.00000      |
|            | 3         | 4.22860              | 0.78046      | -140.52300     | 0.18065                | 1.00000        | 0.00000      |
|            | 4         | 0.26442              | 1.40695      | -138.59700     | 0                      | 1.00000        | 0.00000      |
|            | 5         | 1.30689              | 1.92234      | -137.11500     | 0.38399                | 1.00000        | 0.00000      |
|            | 6         | 0.16628              | 2.73780      | -145.01200     | 0.098523               | 1.00000        | 0.00000      |
|            | 7         | 0.41837              | 3.20158      | -143.87000     | 0.16091                | 1.00000        | 0.00000      |
|            | 8         | 0.66488              | 3.91627      | -140.32400     | 0.61858                | 1.00000        | 0.00000      |
|            | 9         | 0.15038              | 5.10898      | -132.80800     | 0.15209                | 1.00000        | 0.00000      |
|            | 10        | 0.37702              | 5.93767      | -138.60300     | 0.30034                | 1.00000        | 0.00000      |
|            | 11        | 0.11785              | 6.00141      | -127.92400     | 0.28615                | 1.00000        | 0.00000      |
|            | 12        | 0.07589              | 6.59600      | -131.97300     | 0                      | 1.00000        | 0.00000      |
|            | 13        | 0.08329              | 9.98903      | -130.81600     | 0.49118                | 1.00000        | 0.00000      |
| 2008_06_12 | 0         | 1.26999              | 0.17361      | 31.76380       | 0.043039               | 1.00000        | 0.00000      |
|            | 1         | 3.62520              | 0.02698      | 50.80640       | 0.022524               | 1.00000        | 0.00000      |
|            | 2         | 3.23856              | 0.12887      | -135.45500     | 0.079926               | 1.00000        | 0.00000      |
|            | 3         | 2.07199              | 0.57829      | -156.29900     | 0.19259                | 1.00000        | 0.00000      |
|            | 4         | 3.54305              | 0.88632      | -140.95800     | 0.28745                | 1.00000        | 0.00000      |
|            | 5         | 2.46186              | 0.91288      | -153.78100     | 0.11284                | 1.00000        | 0.00000      |
|            | 6         | 0.34036              | 1.54333      | -146.33000     | 0                      | 1.00000        | 0.00000      |

Continued on next page

Table 18 – continued from previous page

| Epoch      | Component | Flux density (Jy) | Rad (mas) | Theta (deg) | Major axis (mas) | Axial ratio | Phi (deg) |
|------------|-----------|-------------------|-----------|-------------|------------------|-------------|-----------|
|            | 7         | 0.50979           | 1.92686   | -135.98100  | 0.15232          | 1.00000     | 0.00000   |
|            | 8         | 0.23834           | 2.18038   | -134.46100  | 0.084983         | 1.00000     | 0.00000   |
|            | 9         | 1.16583           | 3.02482   | -143.28000  | 0.46115          | 1.00000     | 0.00000   |
|            | 10        | 0.84890           | 5.16278   | -140.12200  | 0.99838          | 1.00000     | 0.00000   |
|            | 11        | 0.27806           | 7.94090   | -141.37700  | 0.29994          | 1.00000     | 0.00000   |
| 2008_07_06 | 0         | 1.40809           | 0.18197   | 31.49870    | 0.075132         | 1.00000     | 0.00000   |
|            | 1         | 2.93761           | 0.03583   | 20.91780    | 0.043801         | 1.00000     | 0.00000   |
|            | 2         | 2.55385           | 0.15684   | -137.30000  | 0.084445         | 1.00000     | 0.00000   |
|            | 3         | 0.76974           | 0.41533   | -105.62200  | 0.18899          | 1.00000     | 0.00000   |
|            | 4         | 4.19909           | 0.86089   | -139.67700  | 0.32882          | 1.00000     | 0.00000   |
|            | 5         | 1.08337           | 0.95932   | -153.98200  | 0.067008         | 1.00000     | 0.00000   |
|            | 6         | 0.87013           | 2.11751   | -141.06100  | 0.61957          | 1.00000     | 0.00000   |
|            | 7         | 0.24691           | 3.27639   | -143.20300  | 0.13226          | 1.00000     | 0.00000   |
|            | 8         | 0.54175           | 3.68999   | -138.70400  | 0.48247          | 1.00000     | 0.00000   |
|            | 9         | 0.38037           | 5.94768   | -135.25800  | 0.31163          | 1.00000     | 0.00000   |
| 2008_08_15 | 0         | 1.05949           | 0.05361   | 25.42330    | 0.11265          | 1.00000     | 0.00000   |
|            | 1         | 1.54956           | 0.06735   | -156.49800  | 0.11613          | 1.00000     | 0.00000   |
|            | 2         | 0.89140           | 0.28570   | -136.54100  | 0                | 1.00000     | 0.00000   |
|            | 3         | 0.63171           | 0.49847   | -155.25200  | 0.060435         | 1.00000     | 0.00000   |
|            | 4         | 0.29047           | 0.88285   | -160.03100  | 0.044546         | 1.00000     | 0.00000   |
|            | 5         | 1.88474           | 1.05895   | -150.02200  | 0.1498           | 1.00000     | 0.00000   |
|            | 6         | 1.25367           | 1.10865   | -136.88700  | 0.16779          | 1.00000     | 0.00000   |
|            | 7         | 0.15029           | 1.52178   | -132.26200  | 0.090986         | 1.00000     | 0.00000   |
|            | 8         | 0.15681           | 2.37936   | -147.18500  | 0.058338         | 1.00000     | 0.00000   |
|            | 9         | 0.30429           | 2.37982   | -136.20800  | 0.44565          | 1.00000     | 0.00000   |
|            | 10        | 0.32969           | 3.48798   | -144.09600  | 0.31417          | 1.00000     | 0.00000   |
|            | 11        | 0.21558           | 3.98284   | -142.70600  | 0.24837          | 1.00000     | 0.00000   |
|            | 12        | 0.07210           | 4.47092   | -137.21100  | 0.18304          | 1.00000     | 0.00000   |
|            | 13        | 0.11340           | 5.86753   | -138.78200  | 0.23383          | 1.00000     | 0.00000   |
|            | 14        | 0.05486           | 5.88716   | -130.57800  | 0                | 1.00000     | 0.00000   |
|            | 15        | 0.17609           | 6.55061   | -140.22100  | 0.49481          | 1.00000     | 0.00000   |
|            | 16        | 0.12934           | 7.19007   | -130.95400  | 0.50491          | 1.00000     | 0.00000   |
| 2008_09_10 | 0         | 0.72367           | 0.11821   | 38.26990    | 0.13619          | 1.00000     | 0.00000   |
|            | 1         | 2.39868           | 0.00898   | -108.96300  | 0.12599          | 1.00000     | 0.00000   |
|            | 2         | 1.16858           | 0.31451   | -135.76800  | 0.13746          | 1.00000     | 0.00000   |
|            | 3         | 0.70208           | 0.56379   | -155.65000  | 0.10058          | 1.00000     | 0.00000   |
|            | 4         | 3.16763           | 1.00388   | -143.80200  | 0.36162          | 1.00000     | 0.00000   |
|            | 5         | 1.04367           | 1.16578   | -151.57700  | 0.15855          | 1.00000     | 0.00000   |
|            | 6         | 0.88706           | 1.17655   | -136.41600  | 0.15062          | 1.00000     | 0.00000   |
|            | 7         | 0.43042           | 1.85758   | -140.16300  | 0.53382          | 1.00000     | 0.00000   |
|            | 8         | 0.37544           | 2.39287   | -146.29700  | 0.21087          | 1.00000     | 0.00000   |
|            | 9         | 0.27589           | 2.47370   | -134.40900  | 0.2121           | 1.00000     | 0.00000   |
|            | 10        | 0.50614           | 3.53753   | -143.13200  | 0.3065           | 1.00000     | 0.00000   |
|            | 11        | 0.38324           | 4.05332   | -142.01300  | 0.41052          | 1.00000     | 0.00000   |
|            | 12        | 0.19614           | 5.09690   | -137.11600  | 0.93531          | 1.00000     | 0.00000   |
|            | 13        | 0.16801           | 6.06963   | -136.38700  | 0.43608          | 1.00000     | 0.00000   |
|            | 14        | 0.05082           | 6.62205   | -140.81800  | 0                | 1.00000     | 0.00000   |
|            | 15        | 0.16687           | 6.93606   | -129.88200  | 0.41436          | 1.00000     | 0.00000   |
|            | 16        | 0.04886           | 7.47509   | -135.53000  | 0.12875          | 1.00000     | 0.00000   |
|            | 17        | 0.19794           | 8.03713   | -134.53400  | 0.55836          | 1.00000     | 0.00000   |
|            | 18        | 0.05402           | 9.30301   | -131.44400  | 0.05458          | 1.00000     | 0.00000   |
|            | 19        | 0.04055           | 10.97830  | -136.45500  | 0                | 1.00000     | 0.00000   |
| 2008_11_16 | 0         | 2.85038           | 0.05008   | 49.21560    | 0                | 1.00000     | 0.00000   |
|            | 1         | 1.77038           | 0.06052   | -141.85300  | 0                | 1.00000     | 0.00000   |
|            | 2         | 0.20649           | 0.23812   | -134.41800  | 0                | 1.00000     | 0.00000   |
|            | 3         | 0.88353           | 0.48922   | -142.42900  | 0.12986          | 1.00000     | 0.00000   |
|            | 4         | 0.67726           | 0.78807   | -154.94300  | 0.13824          | 1.00000     | 0.00000   |

Continued on next page

Table 18 – continued from previous page

| Epoch      | Component | Flux<br>density<br>(Jy) | Rad<br>(mas) | Theta<br>(deg) | Major<br>axis<br>(mas) | Axial<br>ratio | Phi<br>(deg) |
|------------|-----------|-------------------------|--------------|----------------|------------------------|----------------|--------------|
|            | 5         | 1.27409                 | 1.08965      | -138.53400     | 0.32291                | 1.00000        | 0.00000      |
|            | 6         | 0.76976                 | 1.11523      | -151.19500     | 0.1144                 | 1.00000        | 0.00000      |
|            | 7         | 1.23414                 | 1.31681      | -136.78100     | 0.15291                | 1.00000        | 0.00000      |
|            | 8         | 1.20624                 | 1.33356      | -149.42300     | 0.14527                | 1.00000        | 0.00000      |
|            | 9         | 0.35175                 | 1.64519      | -141.21200     | 0.44653                | 1.00000        | 0.00000      |
|            | 10        | 0.45694                 | 2.58552      | -134.98300     | 0.49832                | 1.00000        | 0.00000      |
|            | 11        | 0.38790                 | 2.60940      | -148.03900     | 0.16503                | 1.00000        | 0.00000      |
|            | 12        | 0.05893                 | 2.97791      | -145.91000     | 0                      | 1.00000        | 0.00000      |
|            | 13        | 0.62140                 | 3.72540      | -143.21200     | 0.27603                | 1.00000        | 0.00000      |
|            | 14        | 0.34575                 | 4.19848      | -142.49200     | 0.34367                | 1.00000        | 0.00000      |
|            | 15        | 0.34190                 | 4.82546      | -136.67200     | 0.94777                | 1.00000        | 0.00000      |
|            | 16        | 0.08966                 | 5.87867      | -137.93400     | 0.31683                | 1.00000        | 0.00000      |
|            | 17        | 0.17306                 | 6.53916      | -138.74200     | 0.51696                | 1.00000        | 0.00000      |
|            | 18        | 0.43845                 | 6.74020      | -128.36400     | 1.3643                 | 1.00000        | 0.00000      |
|            | 19        | 0.15838                 | 7.72168      | -135.32800     | 0.40713                | 1.00000        | 0.00000      |
|            | 20        | 0.17103                 | 9.59168      | -131.59300     | 1.6919                 | 1.00000        | 0.00000      |
|            | 21        | 0.04302                 | 10.76220     | -131.78700     | 0.096668               | 1.00000        | 0.00000      |
|            | 22        | 0.05198                 | 10.95940     | -126.45600     | 0                      | 1.00000        | 0.00000      |
| 2008_12_21 | 0         | 2.27673                 | 0.03266      | 22.24810       | 0.035172               | 1.00000        | 0.00000      |
|            | 1         | 1.61222                 | 0.07533      | -158.75100     | 0.069411               | 1.00000        | 0.00000      |
|            | 2         | 0.57190                 | 0.61753      | -143.20300     | 0.20024                | 1.00000        | 0.00000      |
|            | 3         | 0.32326                 | 0.89853      | -157.51300     | 0.12018                | 1.00000        | 0.00000      |
|            | 4         | 0.58892                 | 1.18925      | -149.21200     | 0.13288                | 1.00000        | 0.00000      |
|            | 5         | 1.39971                 | 1.32421      | -137.22900     | 0.28522                | 1.00000        | 0.00000      |
|            | 6         | 0.29533                 | 1.46904      | -150.96700     | 0.10662                | 1.00000        | 0.00000      |
|            | 7         | 0.18290                 | 1.88611      | -141.98000     | 0.27025                | 1.00000        | 0.00000      |
|            | 8         | 0.24781                 | 2.92460      | -133.82100     | 0.67531                | 1.00000        | 0.00000      |
|            | 9         | 0.26746                 | 2.70828      | -148.18300     | 0.17664                | 1.00000        | 0.00000      |
|            | 10        | 0.42114                 | 3.81503      | -142.93900     | 0.28506                | 1.00000        | 0.00000      |
|            | 11        | 0.16941                 | 4.31002      | -143.61300     | 0.37685                | 1.00000        | 0.00000      |
|            | 12        | 0.16842                 | 5.05096      | -135.90300     | 0.53035                | 1.00000        | 0.00000      |
|            | 13        | 0.37288                 | 6.81093      | -134.53200     | 1.5832                 | 1.00000        | 0.00000      |
| 2009_01_24 | 0         | 4.11894                 | 0.05145      | 42.92460       | 0.017517               | 1.00000        | 0.00000      |
|            | 1         | 4.77419                 | 0.03925      | -137.06900     | 0.010685               | 1.00000        | 0.00000      |
|            | 2         | 0.72020                 | 0.28568      | -142.15900     | 0.12674                | 1.00000        | 0.00000      |
|            | 3         | 0.22593                 | 0.56025      | -144.72000     | 0.096215               | 1.00000        | 0.00000      |
|            | 4         | 0.48514                 | 0.89674      | -155.68900     | 0.013086               | 1.00000        | 0.00000      |
|            | 5         | 0.73328                 | 0.89943      | -142.25100     | 0.27221                | 1.00000        | 0.00000      |
|            | 6         | 0.98319                 | 1.24282      | -150.19500     | 0.19759                | 1.00000        | 0.00000      |
|            | 7         | 1.14161                 | 1.33491      | -135.56000     | 0.23229                | 1.00000        | 0.00000      |
|            | 8         | 0.44053                 | 1.45532      | -148.62600     | 0.11622                | 1.00000        | 0.00000      |
|            | 9         | 0.83371                 | 1.57685      | -139.99700     | 0.4228                 | 1.00000        | 0.00000      |
|            | 10        | 0.50797                 | 2.74790      | -140.42600     | 0.65947                | 1.00000        | 0.00000      |
|            | 11        | 0.42660                 | 2.76585      | -148.67700     | 0.15505                | 1.00000        | 0.00000      |
|            | 12        | 0.06446                 | 3.53546      | -143.20700     | 0.080923               | 1.00000        | 0.00000      |
|            | 13        | 0.61115                 | 3.90466      | -142.91200     | 0.27707                | 1.00000        | 0.00000      |
|            | 14        | 0.27419                 | 4.47317      | -142.36400     | 0.40003                | 1.00000        | 0.00000      |
|            | 15        | 0.38389                 | 5.00777      | -135.93700     | 1.1485                 | 1.00000        | 0.00000      |
|            | 16        | 0.68761                 | 6.95003      | -134.24400     | 1.85                   | 1.00000        | 0.00000      |
| 2009_02_23 | 0         | 2.96430                 | 0.05205      | 47.02300       | 0.055715               | 1.00000        | 0.00000      |
|            | 1         | 6.23063                 | 0.04039      | -163.67100     | 0.045986               | 1.00000        | 0.00000      |
|            | 2         | 0.09761                 | 0.19168      | -140.18200     | 0                      | 1.00000        | 0.00000      |
|            | 3         | 0.71388                 | 0.65574      | -147.26900     | 0.40346                | 1.00000        | 0.00000      |
|            | 4         | 0.35549                 | 0.92298      | -153.91100     | 0.054483               | 1.00000        | 0.00000      |
|            | 5         | 0.40489                 | 1.19866      | -152.43900     | 0.11554                | 1.00000        | 0.00000      |
|            | 6         | 2.15232                 | 1.38408      | -140.68000     | 0.40374                | 1.00000        | 0.00000      |
|            | 7         | 0.14001                 | 1.57078      | -150.10800     | 0.12106                | 1.00000        | 0.00000      |

Continued on next page

Table 18 – continued from previous page

| Epoch      | Component | Flux<br>density<br>(Jy) | Rad<br>(mas) | Theta<br>(deg) | Major<br>axis<br>(mas) | Axial<br>ratio | Phi<br>(deg) |
|------------|-----------|-------------------------|--------------|----------------|------------------------|----------------|--------------|
|            | 8         | 0.06383                 | 2.01599      | -142.40000     | 0                      | 1.00000        | 0.00000      |
|            | 9         | 0.33397                 | 2.78876      | -139.12000     | 0.64794                | 1.00000        | 0.00000      |
|            | 10        | 0.46761                 | 2.80581      | -148.41600     | 0.14829                | 1.00000        | 0.00000      |
|            | 11        | 0.63456                 | 3.97022      | -142.33500     | 0.48039                | 1.00000        | 0.00000      |
|            | 12        | 0.12895                 | 4.60429      | -141.09800     | 0.16027                | 1.00000        | 0.00000      |
|            | 13        | 0.12443                 | 5.09360      | -135.25600     | 0.47217                | 1.00000        | 0.00000      |
|            | 14        | 0.06450                 | 5.85151      | -138.62700     | 0.10973                | 1.00000        | 0.00000      |
|            | 15        | 0.44134                 | 7.21700      | -132.68300     | 1.8621                 | 1.00000        | 0.00000      |
| 2009_04_02 | 0         | 1.75592                 | 0.16572      | 42.02630       | 0.084824               | 1.00000        | 0.00000      |
|            | 1         | 6.35683                 | 0.03149      | 41.53960       | 0.059724               | 1.00000        | 0.00000      |
|            | 2         | 4.80217                 | 0.07347      | -149.81200     | 0.062674               | 1.00000        | 0.00000      |
|            | 3         | 0.45160                 | 0.53846      | -149.61300     | 0.25059                | 1.00000        | 0.00000      |
|            | 4         | 0.43706                 | 0.95266      | -138.45600     | 0.20709                | 1.00000        | 0.00000      |
|            | 5         | 0.72335                 | 0.96590      | -154.95600     | 0.1111                 | 1.00000        | 0.00000      |
|            | 6         | 0.74087                 | 1.23133      | -151.70800     | 0.19925                | 1.00000        | 0.00000      |
|            | 7         | 0.32311                 | 1.31201      | -135.57700     | 0.1036                 | 1.00000        | 0.00000      |
|            | 8         | 0.67673                 | 1.50117      | -148.04600     | 0.23771                | 1.00000        | 0.00000      |
|            | 9         | 1.23406                 | 1.47794      | -136.10100     | 0.3128                 | 1.00000        | 0.00000      |
|            | 10        | 0.11072                 | 2.03601      | -141.63500     | 0                      | 1.00000        | 0.00000      |
|            | 11        | 0.87561                 | 2.84437      | -148.39200     | 0.20217                | 1.00000        | 0.00000      |
|            | 12        | 0.45729                 | 2.84137      | -138.12400     | 0.79041                | 1.00000        | 0.00000      |
|            | 13        | 0.51561                 | 3.89891      | -142.36000     | 0.25921                | 1.00000        | 0.00000      |
|            | 14        | 0.23791                 | 4.39868      | -143.03900     | 0.20932                | 1.00000        | 0.00000      |
|            | 15        | 0.49133                 | 4.84052      | -136.96400     | 1.0652                 | 1.00000        | 0.00000      |
|            | 16        | 0.05906                 | 5.92011      | -140.33700     | 0.089756               | 1.00000        | 0.00000      |
|            | 17        | 0.68044                 | 7.13207      | -132.35600     | 1.951                  | 1.00000        | 0.00000      |
| 2009_05_30 | 0         | 1.06329                 | 0.21031      | 43.55740       | 0                      | 1.00000        | 0.00000      |
|            | 1         | 4.61866                 | 0.06917      | 23.47630       | 0.05796                | 1.00000        | 0.00000      |
|            | 2         | 4.12171                 | 0.11764      | -142.82800     | 0.08253                | 1.00000        | 0.00000      |
|            | 3         | 0.13704                 | 0.60704      | -168.55600     | 0                      | 1.00000        | 0.00000      |
|            | 4         | 0.56624                 | 0.89136      | -142.28800     | 0.28183                | 1.00000        | 0.00000      |
|            | 5         | 0.34692                 | 1.06935      | -155.20200     | 0.037892               | 1.00000        | 0.00000      |
|            | 6         | 0.23502                 | 1.27883      | -152.52600     | 0.090239               | 1.00000        | 0.00000      |
|            | 7         | 0.43194                 | 1.40714      | -132.78100     | 0.18357                | 1.00000        | 0.00000      |
|            | 8         | 1.19664                 | 1.42961      | -141.99700     | 0.36805                | 1.00000        | 0.00000      |
|            | 9         | 0.17121                 | 1.87664      | -149.41800     | 0.23042                | 1.00000        | 0.00000      |
|            | 10        | 0.05310                 | 2.06987      | -139.73700     | 0                      | 1.00000        | 0.00000      |
|            | 11        | 0.37429                 | 2.87962      | -139.41400     | 0.67196                | 1.00000        | 0.00000      |
|            | 12        | 0.94928                 | 2.91130      | -147.85700     | 0.2139                 | 1.00000        | 0.00000      |
|            | 13        | 0.39454                 | 3.91367      | -141.97600     | 0.2764                 | 1.00000        | 0.00000      |
|            | 14        | 0.06272                 | 4.08861      | -137.11500     | 0.081092               | 1.00000        | 0.00000      |
|            | 15        | 0.28170                 | 4.47245      | -142.35800     | 0.26781                | 1.00000        | 0.00000      |
|            | 16        | 0.16262                 | 5.19540      | -135.77500     | 0.5799                 | 1.00000        | 0.00000      |
|            | 17        | 0.04696                 | 5.85946      | -140.74500     | 0                      | 1.00000        | 0.00000      |
|            | 18        | 0.36387                 | 7.31531      | -132.99000     | 1.7377                 | 1.00000        | 0.00000      |
|            | 19        | 0.31308                 | 1.68821      | -135.59400     | 0.16789                | 1.00000        | 0.00000      |
| 2009_06_21 | 0         | 1.29701                 | 0.22810      | 41.20320       | 0.096577               | 1.00000        | 0.00000      |
|            | 1         | 2.05434                 | 0.07529      | 55.03700       | 0                      | 1.00000        | 0.00000      |
|            | 2         | 2.79853                 | 0.08268      | -155.03600     | 0.060985               | 1.00000        | 0.00000      |
|            | 3         | 0.75271                 | 0.27801      | -147.88600     | 0                      | 1.00000        | 0.00000      |
|            | 4         | 0.33789                 | 0.89835      | -154.01900     | 0.069347               | 1.00000        | 0.00000      |
|            | 5         | 0.16395                 | 1.01790      | -144.09700     | 0.073076               | 1.00000        | 0.00000      |
|            | 6         | 0.27257                 | 1.26825      | -155.98500     | 0.18783                | 1.00000        | 0.00000      |
|            | 7         | 1.55190                 | 1.48713      | -138.71700     | 0.37696                | 1.00000        | 0.00000      |
|            | 8         | 0.15140                 | 1.77119      | -146.64100     | 0.063067               | 1.00000        | 0.00000      |
|            | 9         | 0.59375                 | 2.82108      | -147.36500     | 0.19654                | 1.00000        | 0.00000      |
|            | 10        | 0.33612                 | 3.08086      | -147.90100     | 0.16775                | 1.00000        | 0.00000      |

Continued on next page



Table 18 – continued from previous page

| Epoch      | Component | Flux density (Jy) | Rad (mas) | Theta (deg) | Major axis (mas) | Axial ratio | Phi (deg) |
|------------|-----------|-------------------|-----------|-------------|------------------|-------------|-----------|
|            | 11        | 0.13801           | 3.36105   | -138.26300  | 0.22403          | 1.00000     | 0.00000   |
|            | 12        | 0.26567           | 3.88756   | -142.64300  | 0.20037          | 1.00000     | 0.00000   |
|            | 13        | 0.13001           | 4.51306   | -143.23500  | 0.13835          | 1.00000     | 0.00000   |
|            | 14        | 0.13507           | 5.02417   | -136.31500  | 0.43051          | 1.00000     | 0.00000   |
| 2009_07_26 | 0         | 0.77975           | 0.30365   | 37.63350    | 0.12084          | 1.00000     | 0.00000   |
|            | 1         | 1.74074           | 0.11095   | 42.34080    | 0.019174         | 1.00000     | 0.00000   |
|            | 2         | 3.05770           | 0.06098   | -138.88900  | 0.11496          | 1.00000     | 0.00000   |
|            | 3         | 1.10019           | 0.29438   | -143.98000  | 0.085015         | 1.00000     | 0.00000   |
|            | 4         | 0.30185           | 0.43723   | -161.73100  | 0                | 1.00000     | 0.00000   |
|            | 5         | 0.37528           | 0.93607   | -152.66200  | 0.11323          | 1.00000     | 0.00000   |
|            | 6         | 0.47120           | 1.10349   | -135.97900  | 0.3861           | 1.00000     | 0.00000   |
|            | 7         | 0.62637           | 1.31546   | -152.19600  | 0.27512          | 1.00000     | 0.00000   |
|            | 8         | 0.85711           | 1.55959   | -135.83000  | 0.25926          | 1.00000     | 0.00000   |
|            | 9         | 0.68867           | 1.83990   | -142.68600  | 0.55575          | 1.00000     | 0.00000   |
|            | 10        | 0.13418           | 2.86121   | -148.87400  | 0                | 1.00000     | 0.00000   |
|            | 11        | 1.11713           | 2.99525   | -146.54300  | 0.29317          | 1.00000     | 0.00000   |
|            | 12        | 0.10760           | 3.86989   | -141.12300  | 0                | 1.00000     | 0.00000   |
|            | 13        | 0.42383           | 4.36097   | -141.12100  | 0.55096          | 1.00000     | 0.00000   |
|            | 14        | 0.10268           | 5.31605   | -132.49800  | 0.17926          | 1.00000     | 0.00000   |
|            | 15        | 0.06915           | 6.50367   | -126.23400  | 0                | 1.00000     | 0.00000   |
| 2009_08_16 | 0         | 0.59339           | 0.32515   | 34.40950    | 0.052645         | 1.00000     | 0.00000   |
|            | 1         | 0.97037           | 0.18802   | 34.39050    | 0.055269         | 1.00000     | 0.00000   |
|            | 2         | 1.36056           | 0.03631   | -15.90840   | 0.10663          | 1.00000     | 0.00000   |
|            | 3         | 1.67950           | 0.21217   | -144.57500  | 0.16517          | 1.00000     | 0.00000   |
|            | 4         | 0.10991           | 0.81701   | -131.10300  | 0.042299         | 1.00000     | 0.00000   |
|            | 5         | 0.06103           | 0.86137   | -152.20600  | 0.044869         | 1.00000     | 0.00000   |
|            | 6         | 0.61983           | 1.18809   | -150.54200  | 0.28452          | 1.00000     | 0.00000   |
|            | 7         | 0.26709           | 1.43091   | -131.32000  | 0.20847          | 1.00000     | 0.00000   |
|            | 8         | 0.89220           | 1.66139   | -138.22400  | 0.46191          | 1.00000     | 0.00000   |
|            | 9         | 0.03808           | 2.16428   | -138.93800  | 0                | 1.00000     | 0.00000   |
|            | 10        | 0.08032           | 2.83322   | -149.27900  | 0                | 1.00000     | 0.00000   |
|            | 11        | 0.86504           | 2.98826   | -146.23700  | 0.29265          | 1.00000     | 0.00000   |
|            | 12        | 0.07193           | 3.21110   | -133.52700  | 0.28272          | 1.00000     | 0.00000   |
|            | 13        | 0.18231           | 3.92075   | -141.65700  | 0.30533          | 1.00000     | 0.00000   |
|            | 14        | 0.15818           | 4.50634   | -141.28800  | 0.3138           | 1.00000     | 0.00000   |
|            | 15        | 0.01641           | 5.02041   | -139.66200  | 0                | 1.00000     | 0.00000   |
|            | 16        | 0.17268           | 5.04722   | -134.67000  | 0.68884          | 1.00000     | 0.00000   |
|            | 17        | 0.26912           | 7.06492   | -131.21800  | 1.7182           | 1.00000     | 0.00000   |
|            | 18        | 0.03221           | 8.23090   | -132.13800  | 0                | 1.00000     | 0.00000   |
| 2009_08_28 | 0         | 1.51082           | 0.03115   | 76.75750    | 0                | 1.00000     | 0.00000   |
|            | 1         | 1.17196           | 0.11960   | -155.42300  | 0                | 1.00000     | 0.00000   |
|            | 2         | 1.62572           | 0.25329   | -138.83700  | 0.051023         | 1.00000     | 0.00000   |
|            | 3         | 2.76029           | 0.48462   | -146.75300  | 0.14823          | 1.00000     | 0.00000   |
|            | 4         | 0.18319           | 0.76430   | -150.88300  | 0.061427         | 1.00000     | 0.00000   |
|            | 5         | 0.60650           | 1.24111   | -139.44500  | 0.39942          | 1.00000     | 0.00000   |
|            | 6         | 0.57198           | 1.45192   | -151.09400  | 0.17258          | 1.00000     | 0.00000   |
|            | 7         | 0.81332           | 1.79347   | -144.75100  | 0.38214          | 1.00000     | 0.00000   |
|            | 8         | 0.64806           | 1.80393   | -134.69000  | 0.20349          | 1.00000     | 0.00000   |
|            | 9         | 0.15643           | 2.07072   | -136.68100  | 0.08008          | 1.00000     | 0.00000   |
|            | 10        | 0.43403           | 2.29587   | -141.92700  | 0.53677          | 1.00000     | 0.00000   |
|            | 11        | 0.19603           | 3.13361   | -148.92000  | 0.047605         | 1.00000     | 0.00000   |
|            | 12        | 1.26612           | 3.30709   | -146.20600  | 0.23825          | 1.00000     | 0.00000   |
|            | 13        | 0.17031           | 3.35300   | -135.16400  | 0.44275          | 1.00000     | 0.00000   |
|            | 14        | 0.30203           | 4.17871   | -142.15800  | 0.28707          | 1.00000     | 0.00000   |
|            | 15        | 0.24560           | 4.79604   | -141.42600  | 0.33347          | 1.00000     | 0.00000   |
|            | 16        | 0.39012           | 5.26237   | -136.73900  | 0.92534          | 1.00000     | 0.00000   |
|            | 17        | 0.62635           | 7.39092   | -133.25500  | 2.0519           | 1.00000     | 0.00000   |

Continued on next page

Table 18 – continued from previous page

| Epoch      | Component | Flux density (Jy) | Rad (mas) | Theta (deg) | Major axis (mas) | Axial ratio | Phi (deg) |
|------------|-----------|-------------------|-----------|-------------|------------------|-------------|-----------|
|            | 18        | 0.06421           | 8.84911   | -134.96400  | 0.18734          | 1.00000     | 0.00000   |
|            | 19        | 0.20710           | 11.37160  | -130.38400  | 1.7497           | 1.00000     | 0.00000   |
|            | 20        | 0.19552           | 15.73770  | -119.88200  | 1.3644           | 1.00000     | 0.00000   |
| 2009_09_16 | 0         | 1.23844           | 0.06959   | 39.32430    | 0                | 1.00000     | 0.00000   |
|            | 1         | 2.13444           | 0.03929   | -143.23000  | 0                | 1.00000     | 0.00000   |
|            | 2         | 1.74378           | 0.21782   | -131.67300  | 0.11092          | 1.00000     | 0.00000   |
|            | 3         | 0.36213           | 0.37480   | -144.23100  | 0                | 1.00000     | 0.00000   |
|            | 4         | 2.46497           | 0.52405   | -144.85500  | 0.14981          | 1.00000     | 0.00000   |
|            | 5         | 0.62145           | 1.40825   | -139.78800  | 0.25614          | 1.00000     | 0.00000   |
|            | 6         | 0.74019           | 1.48439   | -150.07300  | 0.20379          | 1.00000     | 0.00000   |
|            | 7         | 0.94150           | 1.81931   | -133.97200  | 0.24704          | 1.00000     | 0.00000   |
|            | 8         | 0.48611           | 2.02912   | -146.02800  | 0.25307          | 1.00000     | 0.00000   |
|            | 9         | 0.21981           | 2.13480   | -138.47800  | 0.15335          | 1.00000     | 0.00000   |
|            | 10        | 0.41477           | 3.14013   | -148.12200  | 0.10536          | 1.00000     | 0.00000   |
|            | 11        | 0.41800           | 3.31350   | -141.71800  | 0.59327          | 1.00000     | 0.00000   |
|            | 12        | 0.95216           | 3.32775   | -145.47400  | 0.1888           | 1.00000     | 0.00000   |
|            | 13        | 0.17039           | 4.18980   | -142.28700  | 0.18441          | 1.00000     | 0.00000   |
|            | 14        | 0.47426           | 4.82497   | -140.08300  | 0.67185          | 1.00000     | 0.00000   |
|            | 15        | 0.08217           | 5.55298   | -132.86600  | 0.10078          | 1.00000     | 0.00000   |
|            | 16        | 0.07376           | 6.68584   | -138.06000  | 0.022443         | 1.00000     | 0.00000   |
|            | 17        | 0.25222           | 7.81655   | -135.23400  | 1.6676           | 1.00000     | 0.00000   |
| 2009_10_16 | 0         | 2.30115           | 0.10434   | 20.56450    | 0.069033         | 1.00000     | 0.00000   |
|            | 1         | 2.52355           | 0.01939   | -95.37050   | 0.074109         | 1.00000     | 0.00000   |
|            | 2         | 1.32090           | 0.18912   | -126.19100  | 0.11614          | 1.00000     | 0.00000   |
|            | 3         | 1.33952           | 0.41968   | -142.31500  | 0.11203          | 1.00000     | 0.00000   |
|            | 4         | 2.13205           | 0.57897   | -141.24100  | 0.16933          | 1.00000     | 0.00000   |
|            | 5         | 0.87067           | 1.38620   | -141.26600  | 0.4195           | 1.00000     | 0.00000   |
|            | 6         | 0.39887           | 1.54141   | -150.80900  | 0.17964          | 1.00000     | 0.00000   |
|            | 7         | 0.29127           | 1.78947   | -132.15500  | 0.16326          | 1.00000     | 0.00000   |
|            | 8         | 1.42487           | 1.98389   | -139.28500  | 0.53146          | 1.00000     | 0.00000   |
|            | 9         | 0.13845           | 3.08114   | -139.10200  | 0.16199          | 1.00000     | 0.00000   |
|            | 10        | 0.31936           | 3.09204   | -146.82000  | 0.16431          | 1.00000     | 0.00000   |
|            | 11        | 1.18652           | 3.37701   | -145.29000  | 0.22887          | 1.00000     | 0.00000   |
|            | 12        | 0.06636           | 3.57176   | -138.90800  | 0.15665          | 1.00000     | 0.00000   |
|            | 13        | 0.13321           | 4.20470   | -140.92200  | 0.187            | 1.00000     | 0.00000   |
|            | 14        | 0.49170           | 4.80888   | -139.58000  | 0.59348          | 1.00000     | 0.00000   |
|            | 15        | 0.19978           | 5.78774   | -134.96800  | 0.78075          | 1.00000     | 0.00000   |
|            | 16        | 0.44582           | 7.72880   | -133.83100  | 1.9265           | 1.00000     | 0.00000   |
| 2009_10_25 | 0         | 2.95704           | 0.04855   | 43.20500    | 0                | 1.00000     | 0.00000   |
|            | 1         | 2.54111           | 0.06157   | -144.56700  | 0.016581         | 1.00000     | 0.00000   |
|            | 2         | 1.23691           | 0.23020   | -135.90000  | 0.06911          | 1.00000     | 0.00000   |
|            | 3         | 1.54680           | 0.48531   | -146.48800  | 0.10378          | 1.00000     | 0.00000   |
|            | 4         | 2.04869           | 0.64127   | -142.46200  | 0.15508          | 1.00000     | 0.00000   |
|            | 5         | 0.70259           | 1.41953   | -140.66500  | 0.42343          | 1.00000     | 0.00000   |
|            | 6         | 0.50065           | 1.57468   | -150.59600  | 0.20461          | 1.00000     | 0.00000   |
|            | 7         | 0.27921           | 1.84372   | -133.12700  | 0.11084          | 1.00000     | 0.00000   |
|            | 8         | 1.56775           | 2.02139   | -140.16600  | 0.56813          | 1.00000     | 0.00000   |
|            | 9         | 0.20978           | 3.15801   | -148.12700  | 0.10631          | 1.00000     | 0.00000   |
|            | 10        | 0.48533           | 3.39220   | -140.44400  | 0.87179          | 1.00000     | 0.00000   |
|            | 11        | 1.18374           | 3.42244   | -145.55500  | 0.22607          | 1.00000     | 0.00000   |
|            | 12        | 0.15735           | 4.27776   | -141.92200  | 0.16916          | 1.00000     | 0.00000   |
|            | 13        | 0.31744           | 4.86324   | -140.35000  | 0.44847          | 1.00000     | 0.00000   |
|            | 14        | 0.47731           | 5.36780   | -136.67000  | 1.054            | 1.00000     | 0.00000   |
|            | 15        | 0.67283           | 7.69826   | -133.60500  | 2.0413           | 1.00000     | 0.00000   |
| 2009_11_28 | 0         | 1.39182           | 0.13259   | 35.97300    | 0                | 1.00000     | 0.00000   |
|            | 1         | 6.14786           | 0.03013   | -146.45200  | 0                | 1.00000     | 0.00000   |
|            | 2         | 1.46427           | 0.33293   | -140.16800  | 0                | 1.00000     | 0.00000   |

Continued on next page

Table 18 – continued from previous page

| Epoch      | Component | Flux<br>density<br>(Jy) | Rad<br>(mas) | Theta<br>(deg) | Major<br>axis<br>(mas) | Axial<br>ratio | Phi<br>(deg) |
|------------|-----------|-------------------------|--------------|----------------|------------------------|----------------|--------------|
|            | 3         | 1.15535                 | 0.58220      | -149.29500     | 0                      | 1.00000        | 0.00000      |
|            | 4         | 1.75955                 | 0.70198      | -140.36600     | 0.10054                | 1.00000        | 0.00000      |
|            | 5         | 0.52910                 | 1.53930      | -138.29100     | 0.37651                | 1.00000        | 0.00000      |
|            | 6         | 0.39694                 | 1.55972      | -150.35900     | 0.1665                 | 1.00000        | 0.00000      |
|            | 7         | 0.29638                 | 1.98256      | -133.88500     | 0.14347                | 1.00000        | 0.00000      |
|            | 8         | 1.36813                 | 2.04276      | -142.67300     | 0.63419                | 1.00000        | 0.00000      |
|            | 9         | 0.12847                 | 3.02246      | -147.18100     | 0                      | 1.00000        | 0.00000      |
|            | 10        | 0.46737                 | 3.39514      | -139.58700     | 0.81978                | 1.00000        | 0.00000      |
|            | 11        | 1.10900                 | 3.47457      | -145.49300     | 0.23167                | 1.00000        | 0.00000      |
|            | 12        | 0.11879                 | 4.26029      | -142.68500     | 0.19734                | 1.00000        | 0.00000      |
|            | 13        | 0.23194                 | 4.93461      | -139.86800     | 0.45434                | 1.00000        | 0.00000      |
|            | 14        | 0.54419                 | 5.32455      | -135.89600     | 1.231                  | 1.00000        | 0.00000      |
|            | 15        | 0.04715                 | 7.41222      | -138.81600     | 0.095408               | 1.00000        | 0.00000      |
|            | 16        | 0.49737                 | 8.43814      | -132.00600     | 2.3362                 | 1.00000        | 0.00000      |
| 2009_12_05 | 0         | 3.60107                 | 0.06514      | 37.46620       | 0                      | 1.00000        | 0.00000      |
|            | 1         | 3.91462                 | 0.04810      | -142.92600     | 0                      | 1.00000        | 0.00000      |
|            | 2         | 0.93707                 | 0.21848      | -137.68900     | 0.018223               | 1.00000        | 0.00000      |
|            | 3         | 1.73949                 | 0.51721      | -145.71600     | 0.116                  | 1.00000        | 0.00000      |
|            | 4         | 1.78837                 | 0.70114      | -140.95600     | 0.16166                | 1.00000        | 0.00000      |
|            | 5         | 0.56471                 | 1.44011      | -141.89200     | 0.32069                | 1.00000        | 0.00000      |
|            | 6         | 0.27909                 | 1.71369      | -152.85700     | 0.17216                | 1.00000        | 0.00000      |
|            | 7         | 0.14922                 | 1.86132      | -131.23600     | 0.080305               | 1.00000        | 0.00000      |
|            | 8         | 1.53592                 | 2.03413      | -140.17600     | 0.60923                | 1.00000        | 0.00000      |
|            | 9         | 0.33698                 | 3.14789      | -146.20600     | 0.30435                | 1.00000        | 0.00000      |
|            | 10        | 0.97079                 | 3.50060      | -145.25000     | 0.21955                | 1.00000        | 0.00000      |
|            | 11        | 0.31638                 | 3.58715      | -137.00000     | 0.93575                | 1.00000        | 0.00000      |
|            | 12        | 0.16747                 | 4.31079      | -141.40900     | 0.2387                 | 1.00000        | 0.00000      |
|            | 13        | 0.31964                 | 4.94763      | -139.85300     | 0.45722                | 1.00000        | 0.00000      |
|            | 14        | 0.31827                 | 5.64305      | -136.47000     | 0.94469                | 1.00000        | 0.00000      |
|            | 15        | 0.57991                 | 7.70626      | -133.61200     | 2.3151                 | 1.00000        | 0.00000      |
| 2010_01_10 | 0         | 5.94949                 | 0.03378      | 22.64340       | 0                      | 1.00000        | 0.00000      |
|            | 1         | 5.04968                 | 0.05137      | -139.23100     | 0.029247               | 1.00000        | 0.00000      |
|            | 2         | 0.60687                 | 0.33122      | -135.24900     | 0                      | 1.00000        | 0.00000      |
|            | 3         | 2.47716                 | 0.52936      | -145.38900     | 0.094853               | 1.00000        | 0.00000      |
|            | 4         | 1.34264                 | 0.84449      | -139.45100     | 0.13239                | 1.00000        | 0.00000      |
|            | 5         | 0.30106                 | 1.52379      | -136.49800     | 0.24718                | 1.00000        | 0.00000      |
|            | 6         | 0.23460                 | 1.74422      | -149.40500     | 0.1025                 | 1.00000        | 0.00000      |
|            | 7         | 2.00414                 | 2.01732      | -141.20800     | 0.70264                | 1.00000        | 0.00000      |
|            | 8         | 0.17284                 | 3.01487      | -146.51500     | 0                      | 1.00000        | 0.00000      |
|            | 9         | 0.16330                 | 3.40253      | -134.80400     | 0.13108                | 1.00000        | 0.00000      |
|            | 10        | 1.08096                 | 3.52778      | -144.98000     | 0.19014                | 1.00000        | 0.00000      |
|            | 11        | 0.21078                 | 3.98563      | -141.75200     | 0.17786                | 1.00000        | 0.00000      |
|            | 12        | 0.46910                 | 5.02650      | -139.07300     | 0.55866                | 1.00000        | 0.00000      |
|            | 13        | 0.10830                 | 5.86065      | -137.94500     | 0.07193                | 1.00000        | 0.00000      |
|            | 14        | 0.62091                 | 7.38915      | -134.43000     | 2.2775                 | 1.00000        | 0.00000      |
| 2010_01_26 | 0         | 4.37310                 | 0.05786      | 33.75500       | 0.025397               | 1.00000        | 0.00000      |
|            | 1         | 6.82700                 | 0.07985      | -141.36900     | 0.040724               | 1.00000        | 0.00000      |
|            | 2         | 1.49312                 | 0.27925      | -141.00900     | 0.043362               | 1.00000        | 0.00000      |
|            | 3         | 1.44748                 | 0.58064      | -146.06400     | 0.11687                | 1.00000        | 0.00000      |
|            | 4         | 1.67608                 | 0.81895      | -139.70700     | 0.16686                | 1.00000        | 0.00000      |
|            | 5         | 0.58766                 | 1.55212      | -139.70500     | 0.3601                 | 1.00000        | 0.00000      |
|            | 6         | 0.30388                 | 1.79581      | -150.77000     | 0.17875                | 1.00000        | 0.00000      |
|            | 7         | 1.11526                 | 2.08394      | -138.21200     | 0.54337                | 1.00000        | 0.00000      |
|            | 8         | 0.32497                 | 2.27505      | -150.17800     | 0.21408                | 1.00000        | 0.00000      |
|            | 9         | 0.11963                 | 3.10459      | -146.51800     | 0.069138               | 1.00000        | 0.00000      |
|            | 10        | 0.43615                 | 3.28965      | -138.34200     | 0.81817                | 1.00000        | 0.00000      |
|            | 11        | 0.96895                 | 3.60800      | -144.91600     | 0.22939                | 1.00000        | 0.00000      |

Continued on next page

Table 18 – continued from previous page

| Epoch      | Component | Flux density (Jy) | Rad (mas) | Theta (deg) | Major axis (mas) | Axial ratio | Phi (deg) |
|------------|-----------|-------------------|-----------|-------------|------------------|-------------|-----------|
|            | 12        | 0.13157           | 4.13155   | -141.65600  | 0.17666          | 1.00000     | 0.00000   |
|            | 13        | 0.46586           | 5.08951   | -138.72100  | 0.55749          | 1.00000     | 0.00000   |
|            | 14        | 0.22186           | 6.13600   | -135.41300  | 0.96406          | 1.00000     | 0.00000   |
|            | 15        | 0.38416           | 8.30263   | -133.71500  | 1.8587           | 1.00000     | 0.00000   |
| 2010_02_11 | 0         | 4.66594           | 0.02432   | 89.39610    | 0                | 1.00000     | 0.00000   |
|            | 1         | 7.37256           | 0.05844   | -141.71100  | 0                | 1.00000     | 0.00000   |
|            | 2         | 2.60249           | 0.50368   | -145.84800  | 0.032042         | 1.00000     | 0.00000   |
|            | 3         | 1.11028           | 0.90602   | -139.78400  | 0                | 1.00000     | 0.00000   |
|            | 4         | 0.46130           | 1.57496   | -133.05700  | 0.17104          | 1.00000     | 0.00000   |
|            | 5         | 0.52132           | 1.90627   | -152.04900  | 0.11831          | 1.00000     | 0.00000   |
|            | 6         | 0.77862           | 2.05849   | -140.79700  | 0.19007          | 1.00000     | 0.00000   |
|            | 7         | 0.21622           | 2.55254   | -149.24000  | 0                | 1.00000     | 0.00000   |
|            | 8         | 0.12586           | 3.22013   | -131.36700  | 0.074317         | 1.00000     | 0.00000   |
|            | 9         | 1.04987           | 3.60536   | -144.61700  | 0.25571          | 1.00000     | 0.00000   |
|            | 10        | 0.27737           | 5.20389   | -139.15900  | 0.24909          | 1.00000     | 0.00000   |
| 2010_03_06 | 0         | 2.82268           | 0.18239   | 38.49700    | 0                | 1.00000     | 0.00000   |
|            | 1         | 6.25462           | 0.04241   | 37.46480    | 0.058321         | 1.00000     | 0.00000   |
|            | 2         | 5.41389           | 0.08728   | -140.19000  | 0.066301         | 1.00000     | 0.00000   |
|            | 3         | 0.69489           | 0.29099   | -143.14200  | 0.042894         | 1.00000     | 0.00000   |
|            | 4         | 1.23979           | 0.57706   | -147.33900  | 0.13136          | 1.00000     | 0.00000   |
|            | 5         | 1.51161           | 0.77518   | -139.65800  | 0.16384          | 1.00000     | 0.00000   |
|            | 6         | 0.15401           | 1.05376   | -141.52000  | 0                | 1.00000     | 0.00000   |
|            | 7         | 0.66627           | 1.63787   | -137.39700  | 0.4357           | 1.00000     | 0.00000   |
|            | 8         | 0.37199           | 1.72913   | -151.64500  | 0.18235          | 1.00000     | 0.00000   |
|            | 9         | 0.86589           | 2.16749   | -138.47800  | 0.50138          | 1.00000     | 0.00000   |
|            | 10        | 0.38595           | 2.27727   | -150.24500  | 0.20161          | 1.00000     | 0.00000   |
|            | 11        | 0.24266           | 3.07137   | -145.03000  | 0.35026          | 1.00000     | 0.00000   |
|            | 12        | 0.06062           | 3.21060   | -134.19600  | 2.6464e-08       | 1.00000     | 0.00000   |
|            | 13        | 0.67063           | 3.54562   | -144.92700  | 0.19621          | 1.00000     | 0.00000   |
|            | 14        | 0.35652           | 3.75343   | -143.12400  | 0.36304          | 1.00000     | 0.00000   |
|            | 15        | 0.13265           | 3.78035   | -130.14400  | 0.87291          | 1.00000     | 0.00000   |
|            | 16        | 0.13987           | 4.33595   | -141.32400  | 0.39815          | 1.00000     | 0.00000   |
|            | 17        | 0.28552           | 5.05096   | -139.37300  | 0.40983          | 1.00000     | 0.00000   |
|            | 18        | 0.28774           | 5.77077   | -136.14900  | 1.0107           | 1.00000     | 0.00000   |
|            | 19        | 0.61732           | 7.78870   | -132.61400  | 2.4812           | 1.00000     | 0.00000   |
| 2010_05_19 | 0         | 1.62676           | 0.32978   | 42.48590    | 0                | 1.00000     | 0.00000   |
|            | 1         | 3.39272           | 0.18655   | 46.21020    | 0.053216         | 1.00000     | 0.00000   |
|            | 2         | 3.04591           | 0.03132   | 53.87940    | 0.062094         | 1.00000     | 0.00000   |
|            | 3         | 3.70804           | 0.12745   | -150.15400  | 0.079336         | 1.00000     | 0.00000   |
|            | 4         | 1.05586           | 0.54770   | -148.77000  | 0.20857          | 1.00000     | 0.00000   |
|            | 5         | 1.00380           | 0.82710   | -139.39400  | 0.19326          | 1.00000     | 0.00000   |
|            | 6         | 0.42361           | 1.57951   | -137.46200  | 0.44246          | 1.00000     | 0.00000   |
|            | 7         | 0.21149           | 1.81432   | -153.72800  | 0.20052          | 1.00000     | 0.00000   |
|            | 8         | 0.74475           | 2.08884   | -139.78900  | 0.55029          | 1.00000     | 0.00000   |
|            | 9         | 0.35331           | 2.30345   | -150.92800  | 0.12356          | 1.00000     | 0.00000   |
|            | 10        | 0.17733           | 2.85962   | -145.22700  | 0.39692          | 1.00000     | 0.00000   |
|            | 11        | 0.59348           | 3.57138   | -144.67300  | 0.22712          | 1.00000     | 0.00000   |
|            | 12        | 0.36757           | 3.78773   | -140.52200  | 0.74393          | 1.00000     | 0.00000   |
|            | 13        | 0.14505           | 5.15161   | -139.23500  | 0.38625          | 1.00000     | 0.00000   |
|            | 14        | 0.05885           | 5.77705   | -136.95900  | 0.19758          | 1.00000     | 0.00000   |
|            | 15        | 0.07126           | 6.24395   | -136.33600  | 0.32511          | 1.00000     | 0.00000   |
|            | 16        | 0.03079           | 8.31940   | -128.91800  | 0.11041          | 1.00000     | 0.00000   |
| 2010_06_14 | 0         | 1.32993           | 0.21644   | 34.59110    | 0                | 1.00000     | 0.00000   |
|            | 1         | 1.75373           | 0.08944   | 38.28180    | 0                | 1.00000     | 0.00000   |
|            | 2         | 1.41093           | 0.05114   | -131.15400  | 0                | 1.00000     | 0.00000   |
|            | 3         | 1.84183           | 0.15248   | -131.49100  | 0.035455         | 1.00000     | 0.00000   |
|            | 4         | 2.47777           | 0.30352   | -139.31200  | 0.086788         | 1.00000     | 0.00000   |

Continued on next page

Table 18 – continued from previous page

| Epoch      | Component | Flux<br>density<br>(Jy) | Rad<br>(mas) | Theta<br>(deg) | Major<br>axis<br>(mas) | Axial<br>ratio | Phi<br>(deg) |
|------------|-----------|-------------------------|--------------|----------------|------------------------|----------------|--------------|
|            | 5         | 0.75045                 | 0.69278      | -145.43800     | 0.20629                | 1.00000        | 0.00000      |
|            | 6         | 0.90723                 | 1.00551      | -137.68700     | 0.1998                 | 1.00000        | 0.00000      |
|            | 7         | 0.13982                 | 1.92514      | -150.83500     | 0.21494                | 1.00000        | 0.00000      |
|            | 8         | 0.64732                 | 2.00373      | -139.23500     | 0.60418                | 1.00000        | 0.00000      |
|            | 9         | 0.31314                 | 2.45608      | -149.81300     | 0.12709                | 1.00000        | 0.00000      |
|            | 10        | 0.07114                 | 2.81084      | -139.40100     | 0.22747                | 1.00000        | 0.00000      |
|            | 11        | 0.40976                 | 3.74416      | -144.22100     | 0.22471                | 1.00000        | 0.00000      |
|            | 12        | 0.13945                 | 4.02719      | -142.06500     | 0.42575                | 1.00000        | 0.00000      |
|            | 13        | 0.10248                 | 5.14507      | -137.53300     | 0.45289                | 1.00000        | 0.00000      |
|            | 14        | 0.07200                 | 6.13532      | -137.22700     | 0.19134                | 1.00000        | 0.00000      |
| 2010_08_01 | 0         | 1.87176                 | 0.05260      | 48.82680       | 0                      | 1.00000        | 0.00000      |
|            | 1         | 2.25880                 | 0.06916      | -144.96200     | 0                      | 1.00000        | 0.00000      |
|            | 2         | 0.92841                 | 0.22639      | -140.84100     | 0.074058               | 1.00000        | 0.00000      |
|            | 3         | 3.37850                 | 0.41523      | -141.59300     | 0.095026               | 1.00000        | 0.00000      |
|            | 4         | 2.48756                 | 0.60988      | -142.80000     | 0.11504                | 1.00000        | 0.00000      |
|            | 5         | 0.56749                 | 0.98804      | -146.13000     | 0.20794                | 1.00000        | 0.00000      |
|            | 6         | 1.05774                 | 1.27620      | -137.68400     | 0.19265                | 1.00000        | 0.00000      |
|            | 7         | 0.91873                 | 2.21259      | -139.25500     | 0.65167                | 1.00000        | 0.00000      |
|            | 8         | 0.21186                 | 2.30313      | -152.47100     | 0.20636                | 1.00000        | 0.00000      |
|            | 9         | 0.55466                 | 2.74792      | -149.27300     | 0.17721                | 1.00000        | 0.00000      |
|            | 10        | 0.30963                 | 3.33251      | -141.20100     | 0.75418                | 1.00000        | 0.00000      |
|            | 11        | 0.56473                 | 4.01136      | -143.37200     | 0.28002                | 1.00000        | 0.00000      |
|            | 12        | 0.13679                 | 4.39222      | -143.18400     | 0.19148                | 1.00000        | 0.00000      |
|            | 13        | 0.23886                 | 5.77851      | -138.96600     | 0.81542                | 1.00000        | 0.00000      |
| 2010_08_21 | 0         | 2.57538                 | 0.00947      | 58.17740       | 0                      | 1.00000        | 0.00000      |
|            | 1         | 0.80143                 | 0.10053      | -134.24600     | 0                      | 1.00000        | 0.00000      |
|            | 2         | 2.26353                 | 0.43509      | -138.19200     | 0.08131                | 1.00000        | 0.00000      |
|            | 3         | 2.17151                 | 0.62312      | -144.52600     | 0.16434                | 1.00000        | 0.00000      |
|            | 4         | 1.07760                 | 1.32706      | -138.07400     | 0.20325                | 1.00000        | 0.00000      |
|            | 5         | 0.24968                 | 2.15363      | -150.66100     | 0.18287                | 1.00000        | 0.00000      |
|            | 6         | 0.49866                 | 2.49762      | -136.63600     | 0.6284                 | 1.00000        | 0.00000      |
|            | 7         | 0.40407                 | 2.78241      | -148.82300     | 0.14956                | 1.00000        | 0.00000      |
|            | 8         | 0.58390                 | 4.04396      | -142.89900     | 0.44312                | 1.00000        | 0.00000      |
| 2010_09_18 | 0         | 1.93607                 | 0.07568      | 36.65670       | 0                      | 1.00000        | 0.00000      |
|            | 1         | 4.59247                 | 0.06817      | -159.45400     | 0.10953                | 1.00000        | 0.00000      |
|            | 2         | 0.59029                 | 0.30351      | -138.44500     | 0                      | 1.00000        | 0.00000      |
|            | 3         | 6.43988                 | 0.56461      | -142.42600     | 0.17648                | 1.00000        | 0.00000      |
|            | 4         | 1.29317                 | 0.79171      | -145.23800     | 0.10635                | 1.00000        | 0.00000      |
|            | 5         | 0.30516                 | 1.10075      | -147.01000     | 0                      | 1.00000        | 0.00000      |
|            | 6         | 2.00284                 | 1.39466      | -139.65000     | 0.30603                | 1.00000        | 0.00000      |
|            | 7         | 0.85329                 | 2.34323      | -151.71400     | 0.26854                | 1.00000        | 0.00000      |
|            | 8         | 0.67785                 | 2.42183      | -137.16600     | 0.31942                | 1.00000        | 0.00000      |
|            | 9         | 0.64742                 | 2.83936      | -149.26600     | 0.19034                | 1.00000        | 0.00000      |
|            | 10        | 0.66200                 | 3.26853      | -143.43500     | 0.44712                | 1.00000        | 0.00000      |
|            | 11        | 0.93235                 | 4.16150      | -143.87500     | 0.32351                | 1.00000        | 0.00000      |
|            | 12        | 0.20747                 | 5.28966      | -146.69900     | 0.29592                | 1.00000        | 0.00000      |
|            | 13        | 0.24036                 | 6.37384      | -148.32200     | 0.2969                 | 1.00000        | 0.00000      |
|            | 14        | 0.20253                 | 8.02345      | -146.70300     | 0.21462                | 1.00000        | 0.00000      |
| 2010_10_24 | 0         | 1.92579                 | 0.06756      | 42.25850       | 0.030026               | 1.00000        | 0.00000      |
|            | 1         | 2.36657                 | 0.06984      | -138.65900     | 0.056291               | 1.00000        | 0.00000      |
|            | 2         | 0.45086                 | 0.20851      | -134.40600     | 0.040827               | 1.00000        | 0.00000      |
|            | 3         | 0.95433                 | 0.46125      | -142.36300     | 0.12519                | 1.00000        | 0.00000      |
|            | 4         | 3.03736                 | 0.64388      | -140.14900     | 0.11875                | 1.00000        | 0.00000      |
|            | 5         | 1.00433                 | 0.83221      | -141.60800     | 0.13759                | 1.00000        | 0.00000      |
|            | 6         | 0.27163                 | 1.19092      | -142.02400     | 0.17284                | 1.00000        | 0.00000      |
|            | 7         | 1.06991                 | 1.46571      | -138.09200     | 0.24943                | 1.00000        | 0.00000      |
|            | 8         | 0.08910                 | 2.23929      | -149.73400     | 0.062411               | 1.00000        | 0.00000      |

Continued on next page

Table 18 – continued from previous page

| Epoch      | Component | Flux<br>density<br>(Jy) | Rad<br>(mas) | Theta<br>(deg) | Major<br>axis<br>(mas) | Axial<br>ratio | Phi<br>(deg) |
|------------|-----------|-------------------------|--------------|----------------|------------------------|----------------|--------------|
|            | 9         | 0.48003                 | 2.40534      | -137.03000     | 0.50073                | 1.00000        | 0.00000      |
|            | 10        | 0.23538                 | 2.45658      | -151.46400     | 0.093026               | 1.00000        | 0.00000      |
|            | 11        | 0.54107                 | 2.87321      | -148.87600     | 0.20818                | 1.00000        | 0.00000      |
|            | 12        | 0.27454                 | 3.26595      | -143.40500     | 0.41099                | 1.00000        | 0.00000      |
|            | 13        | 0.14466                 | 3.68800      | -134.08400     | 0.99981                | 1.00000        | 0.00000      |
|            | 14        | 0.44336                 | 4.15741      | -142.47100     | 0.32393                | 1.00000        | 0.00000      |
|            | 15        | 0.11972                 | 4.58429      | -141.89800     | 0.2154                 | 1.00000        | 0.00000      |
|            | 16        | 0.07077                 | 5.70870      | -137.91000     | 0.26754                | 1.00000        | 0.00000      |
|            | 17        | 0.02693                 | 6.03612      | -138.20700     | 0                      | 1.00000        | 0.00000      |
|            | 18        | 0.11292                 | 6.89965      | -135.77800     | 1.0437                 | 1.00000        | 0.00000      |
|            | 19        | 0.08029                 | 8.89292      | -117.18800     | 0.50813                | 1.00000        | 0.00000      |
|            | 20        | 0.04673                 | 9.39959      | -128.32900     | 0.46931                | 1.00000        | 0.00000      |
| 2010_12_04 | 0         | 1.44968                 | 0.06440      | 42.60080       | 0                      | 1.00000        | 0.00000      |
|            | 1         | 1.82983                 | 0.07363      | -154.10200     | 0.083313               | 1.00000        | 0.00000      |
|            | 2         | 0.06903                 | 0.33115      | -130.22900     | 0                      | 1.00000        | 0.00000      |
|            | 3         | 0.82638                 | 0.52487      | -142.30900     | 0.16522                | 1.00000        | 0.00000      |
|            | 4         | 1.99965                 | 0.75403      | -140.97500     | 0.10303                | 1.00000        | 0.00000      |
|            | 5         | 0.50933                 | 0.90090      | -143.94500     | 0.20125                | 1.00000        | 0.00000      |
|            | 6         | 0.20081                 | 1.38544      | -143.32700     | 0.089543               | 1.00000        | 0.00000      |
|            | 7         | 0.60070                 | 1.55931      | -137.56400     | 0.23005                | 1.00000        | 0.00000      |
|            | 8         | 0.41718                 | 2.37917      | -138.30200     | 0.64446                | 1.00000        | 0.00000      |
|            | 9         | 0.19900                 | 2.51704      | -150.89900     | 0.098656               | 1.00000        | 0.00000      |
|            | 10        | 0.46443                 | 2.96371      | -148.77300     | 0.2048                 | 1.00000        | 0.00000      |
|            | 11        | 0.23594                 | 3.40623      | -141.40300     | 0.52331                | 1.00000        | 0.00000      |
|            | 12        | 0.37108                 | 4.27281      | -142.01200     | 0.39198                | 1.00000        | 0.00000      |
|            | 13        | 0.03399                 | 4.75139      | -141.94700     | 0                      | 1.00000        | 0.00000      |
|            | 14        | 0.05191                 | 5.82692      | -138.38100     | 0.15476                | 1.00000        | 0.00000      |
|            | 15        | 0.04847                 | 6.83477      | -132.48000     | 0.20647                | 1.00000        | 0.00000      |
| 2011_01_02 | 0         | 2.27002                 | 0.06211      | 25.34570       | 0.10433                | 1.00000        | 0.00000      |
|            | 1         | 1.32198                 | 0.06935      | -160.04600     | 0.10005                | 1.00000        | 0.00000      |
|            | 2         | 0.44725                 | 0.14367      | -134.31200     | 0                      | 1.00000        | 0.00000      |
|            | 3         | 0.10767                 | 0.35163      | -146.34500     | 0                      | 1.00000        | 0.00000      |
|            | 4         | 0.92564                 | 0.57111      | -140.56300     | 0.19616                | 1.00000        | 0.00000      |
|            | 5         | 2.44030                 | 0.80906      | -139.76100     | 0.12851                | 1.00000        | 0.00000      |
|            | 6         | 0.63724                 | 0.97660      | -143.07400     | 0.25061                | 1.00000        | 0.00000      |
|            | 7         | 0.69226                 | 1.50773      | -138.95200     | 0.2474                 | 1.00000        | 0.00000      |
|            | 8         | 0.15563                 | 1.71111      | -135.27700     | 0                      | 1.00000        | 0.00000      |
|            | 9         | 0.12164                 | 1.77680      | -143.62900     | 0.11912                | 1.00000        | 0.00000      |
|            | 10        | 0.40195                 | 2.48497      | -137.09900     | 0.56653                | 1.00000        | 0.00000      |
|            | 11        | 0.28543                 | 2.59502      | -150.90900     | 0.17741                | 1.00000        | 0.00000      |
|            | 12        | 0.64999                 | 3.00265      | -148.29000     | 0.24385                | 1.00000        | 0.00000      |
|            | 13        | 0.28485                 | 3.37985      | -142.56600     | 0.47236                | 1.00000        | 0.00000      |
|            | 14        | 0.36494                 | 4.29240      | -141.58700     | 0.3894                 | 1.00000        | 0.00000      |
|            | 15        | 0.11438                 | 4.76039      | -141.55400     | 0.23649                | 1.00000        | 0.00000      |
|            | 16        | 0.05010                 | 5.83710      | -137.66000     | 0.12073                | 1.00000        | 0.00000      |
|            | 17        | 0.08741                 | 6.48107      | -138.51400     | 0.39913                | 1.00000        | 0.00000      |
|            | 18        | 0.08659                 | 8.18765      | -137.73200     | 0.43309                | 1.00000        | 0.00000      |
|            | 19        | 0.07697                 | 9.32846      | -131.34900     | 0.92623                | 1.00000        | 0.00000      |
|            | 20        | 0.03966                 | 4.21959      | -129.70200     | 0.14843                | 1.00000        | 0.00000      |
|            | 21        | 0.02757                 | 4.87752      | -133.36600     | 0.12757                | 1.00000        | 0.00000      |
| 2011_02_05 | 0         | 1.76845                 | 0.06528      | 26.36480       | 0.079878               | 1.00000        | 0.00000      |
|            | 1         | 1.28354                 | 0.08505      | -139.55200     | 0.083219               | 1.00000        | 0.00000      |
|            | 2         | 0.28012                 | 0.32137      | -148.19900     | 0.13001                | 1.00000        | 0.00000      |
|            | 3         | 0.46937                 | 0.56837      | -138.39700     | 0.16921                | 1.00000        | 0.00000      |
|            | 4         | 0.84606                 | 0.80502      | -138.13300     | 0.14806                | 1.00000        | 0.00000      |
|            | 5         | 1.54590                 | 0.92892      | -140.90000     | 0.15707                | 1.00000        | 0.00000      |
|            | 6         | 0.15012                 | 1.21392      | -141.55700     | 0                      | 1.00000        | 0.00000      |

Continued on next page

Table 18 – continued from previous page

| Epoch      | Component | Flux<br>density<br>(Jy) | Rad<br>(mas) | Theta<br>(deg) | Major<br>axis<br>(mas) | Axial<br>ratio | Phi<br>(deg) |
|------------|-----------|-------------------------|--------------|----------------|------------------------|----------------|--------------|
|            | 7         | 0.28880                 | 1.48210      | -136.97500     | 0.24249                | 1.00000        | 0.00000      |
|            | 8         | 0.48669                 | 1.79787      | -139.82800     | 0.32101                | 1.00000        | 0.00000      |
|            | 9         | 0.16903                 | 2.55573      | -134.90200     | 0.25853                | 1.00000        | 0.00000      |
|            | 10        | 0.19810                 | 2.67235      | -150.25200     | 0.15415                | 1.00000        | 0.00000      |
|            | 11        | 0.47443                 | 3.04477      | -147.93100     | 0.27689                | 1.00000        | 0.00000      |
|            | 12        | 0.37634                 | 3.42760      | -142.58000     | 0.65875                | 1.00000        | 0.00000      |
|            | 13        | 0.13270                 | 4.32024      | -141.74500     | 0.23497                | 1.00000        | 0.00000      |
|            | 14        | 0.21724                 | 4.70413      | -139.98400     | 0.58554                | 1.00000        | 0.00000      |
|            | 15        | 0.04233                 | 6.08161      | -138.42300     | 0.26836                | 1.00000        | 0.00000      |
|            | 16        | 0.03609                 | 6.73198      | -135.85100     | 0.087022               | 1.00000        | 0.00000      |
|            | 17        | 0.03965                 | 7.25027      | -132.88600     | 0.38194                | 1.00000        | 0.00000      |
| 2011_04_22 | 0         | 1.66607                 | 0.08438      | 37.58620       | 0.033651               | 1.00000        | 0.00000      |
|            | 1         | 2.16818                 | 0.03416      | -148.13400     | 0                      | 1.00000        | 0.00000      |
|            | 2         | 1.04673                 | 0.16586      | -140.72900     | 0                      | 1.00000        | 0.00000      |
|            | 3         | 0.37212                 | 0.39154      | -149.25300     | 0.083604               | 1.00000        | 0.00000      |
|            | 4         | 0.78023                 | 0.70094      | -139.31100     | 0.23118                | 1.00000        | 0.00000      |
|            | 5         | 1.09340                 | 1.00063      | -141.11700     | 0.13878                | 1.00000        | 0.00000      |
|            | 6         | 1.59500                 | 1.15642      | -141.44400     | 0.12787                | 1.00000        | 0.00000      |
|            | 7         | 0.78079                 | 1.73150      | -139.60600     | 0.37904                | 1.00000        | 0.00000      |
|            | 8         | 0.14557                 | 2.07314      | -139.04100     | 0.12194                | 1.00000        | 0.00000      |
|            | 9         | 0.43352                 | 2.80070      | -137.31300     | 0.68525                | 1.00000        | 0.00000      |
|            | 10        | 0.29602                 | 2.87288      | -149.90300     | 0.20875                | 1.00000        | 0.00000      |
|            | 11        | 0.68463                 | 3.23344      | -147.95200     | 0.26387                | 1.00000        | 0.00000      |
|            | 12        | 0.44581                 | 3.78745      | -142.01500     | 0.51624                | 1.00000        | 0.00000      |
|            | 13        | 0.35455                 | 4.81870      | -140.73000     | 0.49124                | 1.00000        | 0.00000      |
|            | 14        | 0.09564                 | 4.81226      | -132.05400     | 0.14286                | 1.00000        | 0.00000      |
|            | 15        | 0.05386                 | 6.76833      | -131.42900     | 0.14563                | 1.00000        | 0.00000      |
|            | 16        | 0.06462                 | 6.79447      | -136.81100     | 0.18645                | 1.00000        | 0.00000      |
|            | 17        | 0.08382                 | 8.42686      | -136.75300     | 0.2574                 | 1.00000        | 0.00000      |
| 2011_05_22 | 0         | 2.07032                 | 0.05915      | 41.32920       | 0.048746               | 1.00000        | 0.00000      |
|            | 1         | 2.29799                 | 0.07839      | -141.67800     | 0.055038               | 1.00000        | 0.00000      |
|            | 2         | 0.54590                 | 0.25234      | -144.96900     | 0.072105               | 1.00000        | 0.00000      |
|            | 3         | 0.17358                 | 0.46577      | -146.51300     | 0.073969               | 1.00000        | 0.00000      |
|            | 4         | 0.47061                 | 0.75490      | -139.01700     | 0.18516                | 1.00000        | 0.00000      |
|            | 5         | 0.63454                 | 1.02648      | -140.40600     | 0.18917                | 1.00000        | 0.00000      |
|            | 6         | 1.49847                 | 1.20887      | -141.64100     | 0.15631                | 1.00000        | 0.00000      |
|            | 7         | 0.56175                 | 1.77333      | -140.28000     | 0.32603                | 1.00000        | 0.00000      |
|            | 8         | 0.17751                 | 2.18498      | -140.93300     | 0.14926                | 1.00000        | 0.00000      |
|            | 9         | 0.26803                 | 2.92881      | -149.26700     | 0.20529                | 1.00000        | 0.00000      |
|            | 10        | 0.27936                 | 2.94914      | -138.81300     | 0.4743                 | 1.00000        | 0.00000      |
|            | 11        | 0.55391                 | 3.32187      | -148.15000     | 0.25069                | 1.00000        | 0.00000      |
|            | 12        | 0.33935                 | 3.66275      | -140.30900     | 0.49155                | 1.00000        | 0.00000      |
|            | 13        | 0.48765                 | 4.80227      | -140.23400     | 0.97459                | 1.00000        | 0.00000      |
|            | 14        | 0.07879                 | 4.86770      | -132.86800     | 0.098796               | 1.00000        | 0.00000      |
|            | 15        | 0.20358                 | 7.21654      | -135.20900     | 1.0556                 | 1.00000        | 0.00000      |
|            | 16        | 0.07762                 | 8.70832      | -136.37000     | 0.45744                | 1.00000        | 0.00000      |
| 2011_06_12 | 0         | 1.03608                 | 0.15923      | 35.83920       | 0.0313                 | 1.00000        | 0.00000      |
|            | 1         | 2.83271                 | 0.02134      | 40.12620       | 0.05015                | 1.00000        | 0.00000      |
|            | 2         | 1.34536                 | 0.13676      | -143.34300     | 0.02524                | 1.00000        | 0.00000      |
|            | 3         | 0.36247                 | 0.44462      | -145.48200     | 0.19837                | 1.00000        | 0.00000      |
|            | 4         | 0.38861                 | 0.72194      | -140.77300     | 0.15194                | 1.00000        | 0.00000      |
|            | 5         | 0.56613                 | 0.99894      | -142.45800     | 0.15392                | 1.00000        | 0.00000      |
|            | 6         | 1.30230                 | 1.21116      | -141.37100     | 0.12621                | 1.00000        | 0.00000      |
|            | 7         | 0.16415                 | 1.36488      | -141.10500     | 0                      | 1.00000        | 0.00000      |
|            | 8         | 0.65813                 | 1.79903      | -140.02700     | 0.41767                | 1.00000        | 0.00000      |
|            | 9         | 0.17244                 | 2.22269      | -142.65100     | 0.1287                 | 1.00000        | 0.00000      |
|            | 10        | 0.25893                 | 2.96337      | -137.04200     | 0.41362                | 1.00000        | 0.00000      |

Continued on next page



Table 18 – continued from previous page

| Epoch      | Component | Flux<br>density<br>(Jy) | Rad<br>(mas) | Theta<br>(deg) | Major<br>axis<br>(mas) | Axial<br>ratio | Phi<br>(deg) |
|------------|-----------|-------------------------|--------------|----------------|------------------------|----------------|--------------|
|            | 11        | 0.36653                 | 2.99255      | -149.84600     | 0.22694                | 1.00000        | 0.00000      |
|            | 12        | 0.66064                 | 3.33993      | -147.46800     | 0.26322                | 1.00000        | 0.00000      |
|            | 13        | 0.24019                 | 3.71301      | -142.70000     | 0.35734                | 1.00000        | 0.00000      |
|            | 14        | 0.34720                 | 4.65954      | -140.31700     | 0.75721                | 1.00000        | 0.00000      |
|            | 15        | 0.11298                 | 4.80369      | -131.35900     | 0.15135                | 1.00000        | 0.00000      |
|            | 16        | 0.07160                 | 7.00511      | -132.42700     | 0.28237                | 1.00000        | 0.00000      |
|            | 17        | 0.11505                 | 7.71899      | -138.24000     | 0.084939               | 1.00000        | 0.00000      |
| 2011_07_21 | 0         | 1.77048                 | 0.09520      | 43.62510       | 0.055761               | 1.00000        | 0.00000      |
|            | 1         | 2.71037                 | 0.03232      | -141.98500     | 0.037701               | 1.00000        | 0.00000      |
|            | 2         | 0.96965                 | 0.18196      | -141.58600     | 0.068836               | 1.00000        | 0.00000      |
|            | 3         | 0.26023                 | 0.38187      | -143.48700     | 0.14823                | 1.00000        | 0.00000      |
|            | 4         | 0.82292                 | 0.80223      | -140.03800     | 0.2924                 | 1.00000        | 0.00000      |
|            | 5         | 0.26835                 | 1.12991      | -142.64100     | 0.086468               | 1.00000        | 0.00000      |
|            | 6         | 1.28348                 | 1.32955      | -141.11500     | 0.16475                | 1.00000        | 0.00000      |
|            | 7         | 0.50653                 | 1.90116      | -141.51100     | 0.29795                | 1.00000        | 0.00000      |
|            | 8         | 0.11110                 | 2.25238      | -139.33000     | 0.093384               | 1.00000        | 0.00000      |
|            | 9         | 0.59653                 | 2.85483      | -139.55900     | 0.94475                | 1.00000        | 0.00000      |
|            | 10        | 0.16953                 | 3.12235      | -149.96100     | 0.23089                | 1.00000        | 0.00000      |
|            | 11        | 0.75326                 | 3.41089      | -147.74200     | 0.2559                 | 1.00000        | 0.00000      |
|            | 12        | 0.55985                 | 3.93023      | -141.38700     | 0.74367                | 1.00000        | 0.00000      |
|            | 13        | 0.28959                 | 5.15560      | -140.46700     | 0.50582                | 1.00000        | 0.00000      |
|            | 14        | 0.10537                 | 4.87288      | -131.56200     | 0.22351                | 1.00000        | 0.00000      |
|            | 15        | 0.05596                 | 6.98974      | -131.35600     | 0.17253                | 1.00000        | 0.00000      |
|            | 16        | 0.69919                 | 8.11172      | -132.13800     | 3.2007                 | 1.00000        | 0.00000      |
| 2011_08_23 | 0         | 0.31698                 | 0.22883      | 33.91560       | 0.19054                | 1.00000        | 0.00000      |
|            | 1         | 2.59218                 | 0.06763      | 51.25610       | 0.016741               | 1.00000        | 0.00000      |
|            | 2         | 2.20811                 | 0.09966      | -134.66100     | 0                      | 1.00000        | 0.00000      |
|            | 3         | 0.21264                 | 0.36958      | -156.74500     | 0.1725                 | 1.00000        | 0.00000      |
|            | 4         | 0.37745                 | 0.67556      | -143.37100     | 0.15248                | 1.00000        | 0.00000      |
|            | 5         | 0.47607                 | 0.99038      | -140.57400     | 0.2405                 | 1.00000        | 0.00000      |
|            | 6         | 0.61238                 | 1.35657      | -139.55900     | 0.12936                | 1.00000        | 0.00000      |
|            | 7         | 0.45167                 | 1.37229      | -144.56600     | 0.15345                | 1.00000        | 0.00000      |
|            | 8         | 0.50752                 | 1.86926      | -142.16700     | 0.39425                | 1.00000        | 0.00000      |
|            | 9         | 0.25631                 | 2.35423      | -140.18600     | 0.45708                | 1.00000        | 0.00000      |
|            | 10        | 0.28019                 | 3.05035      | -136.50200     | 0.43758                | 1.00000        | 0.00000      |
|            | 11        | 0.28081                 | 3.16814      | -148.86200     | 0.30843                | 1.00000        | 0.00000      |
|            | 12        | 0.72535                 | 3.44551      | -147.71200     | 0.27994                | 1.00000        | 0.00000      |
|            | 13        | 0.29431                 | 3.72347      | -142.10800     | 0.51227                | 1.00000        | 0.00000      |
|            | 14        | 0.21435                 | 4.41145      | -138.99700     | 0.68163                | 1.00000        | 0.00000      |
|            | 15        | 0.08047                 | 4.88517      | -131.48600     | 0.20491                | 1.00000        | 0.00000      |
|            | 16        | 0.21376                 | 5.22334      | -140.63900     | 0.4592                 | 1.00000        | 0.00000      |
|            | 17        | 0.17139                 | 7.26255      | -134.18000     | 1.1676                 | 1.00000        | 0.00000      |
|            | 18        | 0.06912                 | 8.76370      | -136.63200     | 0.44587                | 1.00000        | 0.00000      |
| 2011_09_16 | 0         | 0.42591                 | 0.20233      | 45.67520       | 0.055877               | 1.00000        | 0.00000      |
|            | 1         | 1.47291                 | 0.04773      | 54.35040       | 0.051852               | 1.00000        | 0.00000      |
|            | 2         | 1.34238                 | 0.07431      | -155.96300     | 0                      | 1.00000        | 0.00000      |
|            | 3         | 1.03620                 | 0.22319      | -142.16300     | 0.079982               | 1.00000        | 0.00000      |
|            | 4         | 0.11647                 | 0.63704      | -147.51100     | 0                      | 1.00000        | 0.00000      |
|            | 5         | 0.39709                 | 0.87620      | -141.95100     | 0.17739                | 1.00000        | 0.00000      |
|            | 6         | 0.98979                 | 1.41161      | -141.75300     | 0.23539                | 1.00000        | 0.00000      |
|            | 7         | 0.38572                 | 1.96572      | -143.09400     | 0.39769                | 1.00000        | 0.00000      |
|            | 8         | 0.07090                 | 2.38330      | -140.68200     | 0                      | 1.00000        | 0.00000      |
|            | 9         | 0.33240                 | 2.99786      | -137.78400     | 0.58115                | 1.00000        | 0.00000      |
|            | 10        | 0.58172                 | 3.53168      | -147.55200     | 0.25522                | 1.00000        | 0.00000      |
|            | 11        | 0.19776                 | 3.80521      | -141.61100     | 0.5211                 | 1.00000        | 0.00000      |
|            | 12        | 0.25315                 | 4.70230      | -136.28200     | 1.124                  | 1.00000        | 0.00000      |
|            | 13        | 0.12241                 | 5.31280      | -140.44000     | 0.30378                | 1.00000        | 0.00000      |

Continued on next page

Table 18 – continued from previous page

| Epoch      | Component | Flux<br>density<br>(Jy) | Rad<br>(mas) | Theta<br>(deg) | Major<br>axis<br>(mas) | Axial<br>ratio | Phi<br>(deg) |
|------------|-----------|-------------------------|--------------|----------------|------------------------|----------------|--------------|
|            | 14        | 0.15418                 | 7.41703      | -136.58500     | 1.2306                 | 1.00000        | 0.00000      |
|            | 15        | 0.06561                 | 9.47455      | -128.16400     | 0.66845                | 1.00000        | 0.00000      |
|            | 16        | 0.05990                 | 3.08273      | -150.45700     | 0.034059               | 1.00000        | 0.00000      |
|            | 17        | 0.15064                 | 3.31720      | -149.01600     | 0.06665                | 1.00000        | 0.00000      |
| 2011_10_16 | 0         | 0.28169                 | 0.18433      | 36.04130       | 0.055488               | 1.00000        | 0.00000      |
|            | 1         | 1.85059                 | 0.04508      | 50.84720       | 0.056801               | 1.00000        | 0.00000      |
|            | 2         | 1.53467                 | 0.10519      | -146.98200     | 0.050122               | 1.00000        | 0.00000      |
|            | 3         | 0.98045                 | 0.28220      | -141.84700     | 0.038001               | 1.00000        | 0.00000      |
|            | 4         | 0.21865                 | 0.42730      | -148.24300     | 0.18445                | 1.00000        | 0.00000      |
|            | 5         | 0.46521                 | 0.86904      | -141.84200     | 0.1977                 | 1.00000        | 0.00000      |
|            | 6         | 0.32093                 | 1.63329      | -141.92700     | 0.090275               | 1.00000        | 0.00000      |
|            | 7         | 0.32433                 | 2.10372      | -142.22200     | 0.20793                | 1.00000        | 0.00000      |
|            | 8         | 0.52974                 | 2.83152      | -140.51700     | 0.78634                | 1.00000        | 0.00000      |
|            | 9         | 0.11831                 | 3.41829      | -136.16500     | 0.22247                | 1.00000        | 0.00000      |
|            | 10        | 0.15663                 | 3.34116      | -149.17200     | 0.15943                | 1.00000        | 0.00000      |
|            | 11        | 0.83138                 | 3.59839      | -147.28700     | 0.26166                | 1.00000        | 0.00000      |
|            | 12        | 0.33511                 | 4.03377      | -141.40600     | 0.62041                | 1.00000        | 0.00000      |
|            | 13        | 0.07555                 | 4.91306      | -130.10700     | 0.24855                | 1.00000        | 0.00000      |
|            | 14        | 0.24451                 | 5.36785      | -140.19500     | 0.5558                 | 1.00000        | 0.00000      |
|            | 15        | 0.90392                 | 1.45955      | -141.02800     | 0.32646                | 1.00000        | 0.00000      |
|            | 16        | 0.20743                 | 7.38098      | -134.27500     | 0.91368                | 1.00000        | 0.00000      |
|            | 17        | 0.09302                 | 9.00078      | -136.24600     | 0.4142                 | 1.00000        | 0.00000      |
| 2011_12_02 | 0         | 0.98605                 | 0.12022      | 43.93480       | 0                      | 1.00000        | 0.00000      |
|            | 1         | 1.55102                 | 0.01154      | -130.66600     | 0                      | 1.00000        | 0.00000      |
|            | 2         | 0.81113                 | 0.15483      | -139.51000     | 0.065015               | 1.00000        | 0.00000      |
|            | 3         | 0.65397                 | 0.43138      | -145.54300     | 0.085424               | 1.00000        | 0.00000      |
|            | 4         | 0.19124                 | 0.83281      | -141.07900     | 0.14139                | 1.00000        | 0.00000      |
|            | 5         | 0.06939                 | 0.99873      | -140.27500     | 0.060263               | 1.00000        | 0.00000      |
|            | 6         | 0.49290                 | 1.48611      | -141.24800     | 0.35129                | 1.00000        | 0.00000      |
|            | 7         | 0.35995                 | 1.72589      | -141.60400     | 0.14335                | 1.00000        | 0.00000      |
|            | 8         | 0.23334                 | 2.17961      | -143.60600     | 0.34011                | 1.00000        | 0.00000      |
|            | 9         | 0.27763                 | 2.85934      | -137.44800     | 0.61572                | 1.00000        | 0.00000      |
|            | 10        | 0.05655                 | 3.22802      | -134.12700     | 0.15382                | 1.00000        | 0.00000      |
|            | 11        | 0.15691                 | 3.32909      | -147.68800     | 0.22955                | 1.00000        | 0.00000      |
|            | 12        | 0.08618                 | 3.60836      | -137.73400     | 0.21744                | 1.00000        | 0.00000      |
|            | 13        | 0.69716                 | 3.70629      | -147.03100     | 0.31978                | 1.00000        | 0.00000      |
|            | 14        | 0.15523                 | 4.16415      | -140.59400     | 0.47141                | 1.00000        | 0.00000      |
|            | 15        | 0.24830                 | 5.05367      | -135.14200     | 1.0129                 | 1.00000        | 0.00000      |
|            | 16        | 0.08497                 | 5.57521      | -140.80400     | 0.29768                | 1.00000        | 0.00000      |
|            | 17        | 0.16580                 | 7.60733      | -134.30500     | 1.0379                 | 1.00000        | 0.00000      |
|            | 18        | 0.08765                 | 8.98517      | -135.77400     | 0.83408                | 1.00000        | 0.00000      |
| 2012_01_27 | 0         | 1.56654                 | 0.11347      | 40.26380       | 0.055567               | 1.00000        | 0.00000      |
|            | 1         | 2.59605                 | 0.03331      | -121.78300     | 0                      | 1.00000        | 0.00000      |
|            | 2         | 1.11699                 | 0.23804      | -139.66100     | 0.054458               | 1.00000        | 0.00000      |
|            | 3         | 0.31045                 | 0.44548      | -144.02500     | 0                      | 1.00000        | 0.00000      |
|            | 4         | 0.33506                 | 0.84531      | -137.95200     | 0.060891               | 1.00000        | 0.00000      |
|            | 5         | 0.13331                 | 0.95948      | -146.50400     | 0.15618                | 1.00000        | 0.00000      |
|            | 6         | 0.60980                 | 1.56992      | -142.26100     | 0.48099                | 1.00000        | 0.00000      |
|            | 7         | 0.39703                 | 1.84916      | -142.00400     | 0.12341                | 1.00000        | 0.00000      |
|            | 8         | 0.12398                 | 2.27081      | -142.01700     | 0                      | 1.00000        | 0.00000      |
|            | 9         | 0.08131                 | 2.48785      | -140.45400     | 0                      | 1.00000        | 0.00000      |
|            | 10        | 0.06631                 | 2.60247      | -129.13100     | 0                      | 1.00000        | 0.00000      |
|            | 11        | 0.25425                 | 3.11164      | -136.34000     | 0.4139                 | 1.00000        | 0.00000      |
|            | 12        | 0.22360                 | 3.41988      | -147.56300     | 0.31373                | 1.00000        | 0.00000      |
|            | 13        | 0.15087                 | 3.75564      | -137.31000     | 0.15524                | 1.00000        | 0.00000      |
|            | 14        | 0.80433                 | 3.84032      | -146.40500     | 0.29863                | 1.00000        | 0.00000      |
|            | 15        | 0.15533                 | 4.49321      | -140.67900     | 0.18228                | 1.00000        | 0.00000      |

Continued on next page

Table 18 – continued from previous page

| Epoch      | Component | Flux<br>density<br>(Jy) | Rad<br>(mas) | Theta<br>(deg) | Major<br>axis<br>(mas) | Axial<br>ratio | Phi<br>(deg) |
|------------|-----------|-------------------------|--------------|----------------|------------------------|----------------|--------------|
|            | 16        | 0.10328                 | 4.75505      | -133.55200     | 0.22191                | 1.00000        | 0.00000      |
|            | 17        | 0.20329                 | 5.47094      | -139.73900     | 0.47663                | 1.00000        | 0.00000      |
|            | 18        | 0.08064                 | 7.80244      | -132.46100     | 0.34241                | 1.00000        | 0.00000      |
| 2012_03_05 | 0         | 0.41456                 | 0.22957      | 46.49100       | 0.044808               | 1.00000        | 0.00000      |
|            | 1         | 1.03498                 | 0.07830      | 41.46300       | 0.086477               | 1.00000        | 0.00000      |
|            | 2         | 1.28643                 | 0.06977      | -147.31800     | 0.075201               | 1.00000        | 0.00000      |
|            | 3         | 0.40288                 | 0.25948      | -141.84200     | 0.11015                | 1.00000        | 0.00000      |
|            | 4         | 0.33788                 | 0.76241      | -141.97700     | 0.28419                | 1.00000        | 0.00000      |
|            | 5         | 0.20937                 | 1.38515      | -144.59800     | 0.34819                | 1.00000        | 0.00000      |
|            | 6         | 0.37030                 | 1.87108      | -142.73200     | 0.31595                | 1.00000        | 0.00000      |
|            | 7         | 0.20109                 | 2.54889      | -140.58100     | 0.59088                | 1.00000        | 0.00000      |
|            | 8         | 0.01548                 | 32.08470     | -112.61100     | 0.25765                | 1.00000        | 0.00000      |
|            | 9         | 0.04558                 | 2.93540      | -135.98700     | 0.23459                | 1.00000        | 0.00000      |
|            | 10        | 0.10976                 | 3.43446      | -148.28900     | 0.24516                | 1.00000        | 0.00000      |
|            | 11        | 0.15365                 | 3.40359      | -135.86700     | 0.49144                | 1.00000        | 0.00000      |
|            | 12        | 0.44760                 | 3.85710      | -146.16800     | 0.32052                | 1.00000        | 0.00000      |
|            | 13        | 0.04635                 | 4.37666      | -140.05900     | 0.15817                | 1.00000        | 0.00000      |
|            | 14        | 0.06908                 | 5.72036      | -140.82000     | 0.39811                | 1.00000        | 0.00000      |
|            | 15        | 0.05012                 | 10.25390     | -117.84300     | 0.51887                | 1.00000        | 0.00000      |
|            | 16        | 0.29225                 | 4.70777      | -137.09000     | 1.2328                 | 1.00000        | 0.00000      |
|            | 17        | 0.51902                 | 7.90225      | -132.68800     | 4.3561                 | 1.00000        | 0.00000      |
|            | 18        | 0.06162                 | 14.97550     | -119.83100     | 1.226                  | 1.00000        | 0.00000      |
| 2012_04_03 | 0         | 0.56201                 | 0.25559      | 44.70710       | 0.18                   | 0.38942        | 24.99980     |
|            | 1         | 1.46002                 | 0.06905      | 39.62700       | 0.066794               | 1.00000        | 0.00000      |
|            | 2         | 1.50143                 | 0.07044      | -134.06500     | 0.062108               | 1.00000        | 0.00000      |
|            | 3         | 1.23144                 | 0.26935      | -136.16400     | 0.10614                | 1.00000        | 0.00000      |
|            | 4         | 0.35626                 | 0.82446      | -139.12200     | 0.20358                | 1.00000        | 0.00000      |
|            | 5         | 0.21816                 | 1.36338      | -140.53300     | 0.22206                | 1.00000        | 0.00000      |
|            | 6         | 0.62168                 | 1.81937      | -141.38700     | 0.33278                | 1.00000        | 0.00000      |
|            | 7         | 0.21884                 | 2.16684      | -142.29600     | 0.17892                | 1.00000        | 0.00000      |
|            | 8         | 0.09181                 | 2.68887      | -140.02900     | 0.22584                | 1.00000        | 0.00000      |
|            | 9         | 0.05142                 | 3.18046      | -141.40500     | 0                      | 1.00000        | 0.00000      |
|            | 10        | 0.25200                 | 3.62713      | -148.40200     | 0.42509                | 1.00000        | 0.00000      |
|            | 11        | 0.14181                 | 3.65373      | -135.05500     | 0.18302                | 1.00000        | 0.00000      |
|            | 12        | 0.55590                 | 3.99505      | -145.77300     | 0.31859                | 1.00000        | 0.00000      |
|            | 13        | 0.12712                 | 4.33420      | -140.71600     | 0.14325                | 1.00000        | 0.00000      |
|            | 14        | 0.09877                 | 5.70816      | -138.38400     | 0.25955                | 1.00000        | 0.00000      |
| 2012_05_26 | 0         | 0.68672                 | 0.16294      | 42.22140       | 0                      | 1.00000        | 0.00000      |
|            | 1         | 2.58472                 | 0.01595      | -116.04000     | 0                      | 1.00000        | 0.00000      |
|            | 2         | 0.42504                 | 0.58647      | -145.54700     | 0.1677                 | 1.00000        | 0.00000      |
|            | 3         | 0.23751                 | 1.06638      | -139.55200     | 0.14907                | 1.00000        | 0.00000      |
|            | 4         | 0.60794                 | 1.86936      | -140.70300     | 0.40417                | 1.00000        | 0.00000      |
|            | 5         | 0.55856                 | 2.34328      | -141.72400     | 0.35677                | 1.00000        | 0.00000      |
|            | 6         | 0.08384                 | 2.93938      | -140.07700     | 0.14469                | 1.00000        | 0.00000      |
|            | 7         | 0.20327                 | 3.70262      | -133.41100     | 0.36384                | 1.00000        | 0.00000      |
|            | 8         | 0.15417                 | 3.76074      | -146.71900     | 0.21431                | 1.00000        | 0.00000      |
|            | 9         | 0.55729                 | 4.15181      | -145.26500     | 0.25888                | 1.00000        | 0.00000      |
|            | 10        | 0.54376                 | 4.55170      | -138.82100     | 0.92636                | 1.00000        | 0.00000      |
|            | 11        | 0.08556                 | 5.78294      | -137.59100     | 0.13845                | 1.00000        | 0.00000      |
|            | 12        | 1.23192                 | 0.29430      | -136.46300     | 0.071193               | 1.00000        | 0.00000      |
| 2012_07_04 | 0         | 1.19909                 | 0.10977      | 45.58000       | 0                      | 1.00000        | 0.00000      |
|            | 1         | 1.57694                 | 0.01825      | -112.33300     | 0                      | 1.00000        | 0.00000      |
|            | 2         | 0.89680                 | 0.14670      | -139.61800     | 0.089864               | 1.00000        | 0.00000      |
|            | 3         | 0.40658                 | 0.48683      | -142.33700     | 0.13785                | 1.00000        | 0.00000      |
|            | 4         | 0.34593                 | 1.96195      | -141.21300     | 0.24915                | 1.00000        | 0.00000      |
|            | 5         | 0.31722                 | 2.44016      | -143.98200     | 0.27901                | 1.00000        | 0.00000      |
|            | 6         | 0.05499                 | 2.85811      | -139.89500     | 0                      | 1.00000        | 0.00000      |

Continued on next page

Table 18 – continued from previous page

| Epoch      | Component | Flux density (Jy) | Rad (mas) | Theta (deg) | Major axis (mas) | Axial ratio | Phi (deg) |
|------------|-----------|-------------------|-----------|-------------|------------------|-------------|-----------|
|            | 7         | 0.19763           | 3.57021   | -134.89600  | 0.395            | 1.00000     | 0.00000   |
|            | 8         | 0.12648           | 3.70031   | -146.35500  | 0.20908          | 1.00000     | 0.00000   |
|            | 9         | 0.05371           | 3.98811   | -133.31200  | 0                | 1.00000     | 0.00000   |
|            | 10        | 0.59580           | 4.20353   | -145.34000  | 0.30889          | 1.00000     | 0.00000   |
|            | 11        | 0.51866           | 5.09383   | -135.67100  | 1.2661           | 1.00000     | 0.00000   |
|            | 12        | 0.04246           | 5.93923   | -140.51600  | 2.9533e-08       | 1.00000     | 0.00000   |
|            | 13        | 0.43402           | 8.18872   | -132.37300  | 1.8861           | 1.00000     | 0.00000   |
|            | 14        | 0.19772           | 1.09536   | -139.44700  | 0.3211           | 1.00000     | 0.00000   |
|            | 15        | 0.07558           | 1.40673   | -140.97600  | 0.1182           | 1.00000     | 0.00000   |
| 2012_08_13 | 0         | 1.23678           | 0.10019   | 44.99480    | 0.027892         | 1.00000     | 0.00000   |
|            | 1         | 1.48050           | 0.06261   | -130.42300  | 0.019812         | 1.00000     | 0.00000   |
|            | 2         | 0.48302           | 0.18575   | -134.54900  | 0                | 1.00000     | 0.00000   |
|            | 3         | 0.28121           | 0.60209   | -142.02300  | 0.15576          | 1.00000     | 0.00000   |
|            | 4         | 0.18702           | 1.19428   | -140.11700  | 0.1255           | 1.00000     | 0.00000   |
|            | 5         | 0.05601           | 1.45026   | -141.93600  | 0                | 1.00000     | 0.00000   |
|            | 6         | 0.36565           | 2.09205   | -142.28000  | 0.29567          | 1.00000     | 0.00000   |
|            | 7         | 0.25823           | 2.62992   | -143.26900  | 0.35312          | 1.00000     | 0.00000   |
|            | 8         | 0.04801           | 3.25844   | -133.78900  | 0.062437         | 1.00000     | 0.00000   |
|            | 9         | 0.10246           | 3.79233   | -144.93900  | 0.22067          | 1.00000     | 0.00000   |
|            | 10        | 0.09252           | 3.90015   | -135.79700  | 0.18806          | 1.00000     | 0.00000   |
|            | 11        | 0.43823           | 4.32362   | -145.37400  | 0.29792          | 1.00000     | 0.00000   |
|            | 12        | 0.33607           | 4.88422   | -136.59800  | 1.0312           | 1.00000     | 0.00000   |
|            | 13        | 0.11640           | 6.02870   | -138.41100  | 0.38429          | 1.00000     | 0.00000   |
|            | 14        | 0.07596           | 7.66228   | -137.39500  | 0.59196          | 1.00000     | 0.00000   |
|            | 15        | 0.10424           | 8.94476   | -133.25800  | 1.0516           | 1.00000     | 0.00000   |
|            | 16        | 0.12885           | 15.23910  | -125.21200  | 1.1462           | 1.00000     | 0.00000   |
| 2012_10_28 | 0         | 0.77893           | 0.12646   | 45.57060    | 0                | 1.00000     | 0.00000   |
|            | 1         | 1.69069           | 0.01708   | 51.06050    | 0                | 1.00000     | 0.00000   |
|            | 2         | 1.25649           | 0.09627   | -128.22400  | 0.038637         | 1.00000     | 0.00000   |
|            | 3         | 0.50105           | 0.24035   | -130.98100  | 0.065829         | 1.00000     | 0.00000   |
|            | 4         | 0.12117           | 0.42360   | -137.71900  | 0.12731          | 1.00000     | 0.00000   |
|            | 5         | 0.19205           | 0.89267   | -140.11500  | 0.25462          | 1.00000     | 0.00000   |
|            | 6         | 0.15540           | 1.37027   | -140.09500  | 0.22529          | 1.00000     | 0.00000   |
|            | 7         | 0.28271           | 2.14712   | -140.86500  | 0.29526          | 1.00000     | 0.00000   |
|            | 8         | 0.31141           | 2.72363   | -142.36200  | 0.36784          | 1.00000     | 0.00000   |
|            | 9         | 0.02159           | 3.15666   | -148.26900  | 0.057741         | 1.00000     | 0.00000   |
|            | 10        | 0.13745           | 3.23682   | -136.03400  | 0.87276          | 1.00000     | 0.00000   |
|            | 11        | 0.09079           | 4.01266   | -134.51000  | 0.32519          | 1.00000     | 0.00000   |
|            | 12        | 0.12051           | 4.12399   | -145.64300  | 0.26919          | 1.00000     | 0.00000   |
|            | 13        | 0.40908           | 4.53479   | -144.35300  | 0.35231          | 1.00000     | 0.00000   |
|            | 14        | 0.29337           | 4.99196   | -135.74100  | 0.96228          | 1.00000     | 0.00000   |
|            | 15        | 0.04011           | 5.80271   | -129.14000  | 0.21325          | 1.00000     | 0.00000   |
|            | 16        | 0.03968           | 6.09023   | -139.02600  | 0.095823         | 1.00000     | 0.00000   |
|            | 17        | 0.12070           | 6.44807   | -138.45100  | 0.70534          | 1.00000     | 0.00000   |
|            | 18        | 0.16034           | 8.27179   | -133.03900  | 1.5065           | 1.00000     | 0.00000   |
|            | 19        | 0.10396           | 10.66020  | -117.79800  | 1.3111           | 1.00000     | 0.00000   |
|            | 20        | 0.10740           | 15.76420  | -122.17100  | 1.4776           | 1.00000     | 0.00000   |
| 2012_12_22 | 0         | 0.79346           | 0.18152   | 25.36280    | 0.060975         | 1.00000     | 0.00000   |
|            | 1         | 4.37677           | 0.02475   | -108.62300  | 0.21291          | 1.00000     | 0.00000   |
|            | 2         | 0.20882           | 0.36226   | -145.71000  | 0                | 1.00000     | 0.00000   |
|            | 3         | 0.13875           | 0.50374   | -132.52600  | 0                | 1.00000     | 0.00000   |
|            | 4         | 0.72756           | 1.94828   | -140.77000  | 0.53248          | 1.00000     | 0.00000   |
|            | 5         | 0.61834           | 3.40954   | -142.36900  | 0.6229           | 1.00000     | 0.00000   |
|            | 6         | 0.12156           | 4.69963   | -136.27800  | 0.26547          | 1.00000     | 0.00000   |
|            | 7         | 0.37570           | 4.74904   | -145.51400  | 0.39182          | 1.00000     | 0.00000   |
|            | 8         | 0.02545           | 6.03787   | -136.33200  | 0                | 1.00000     | 0.00000   |
